# Supplementary material for: Uncertainty in the Hot Hand Fallacy: Detecting Streaky Alternatives to Random Bernoulli Sequences
Source: arXiv:1908.01406 ancillary file (2021-04-02)
Supplement: Supplementary file 1 [file hot_hand_online.pdf]

Online Appendix for  
**Uncertainty in the Hot Hand Fallacy:  
Detecting Streaky Alternatives to Random Bernoulli Sequences**

David M. Ritzwoller      Joseph P. Romano  
Stanford University      Stanford University

January 21, 2021

## Contents

|          |                                                                                                              |           |
|----------|--------------------------------------------------------------------------------------------------------------|-----------|
| <b>A</b> | <b>Application to Two Problems in Empirical Finance</b>                                                      | <b>3</b>  |
| A.1      | Tests of the Weak Form Efficient Market Hypothesis . . . . .                                                 | 3         |
| A.1.1    | Discussion of Fama (1965) . . . . .                                                                          | 3         |
| A.1.2    | Methods . . . . .                                                                                            | 3         |
| A.1.3    | Data . . . . .                                                                                               | 5         |
| A.1.4    | Results . . . . .                                                                                            | 6         |
| A.1.5    | Power . . . . .                                                                                              | 7         |
| A.2      | Tests of Persistence in the Performance of Mutual Funds . . . . .                                            | 11        |
| <b>B</b> | <b>Dynamic Potential Outcome Notation</b>                                                                    | <b>15</b> |
| B.1      | Relationship Between Independence and State Dependence . . . . .                                             | 15        |
| B.2      | Stationarity and Dependence of Observed Outcomes . . . . .                                                   | 21        |
| B.3      | Markov Chain Streaky Alternatives . . . . .                                                                  | 22        |
| <b>C</b> | <b>Asymptotic Distributions of <math>\bar{P}_k(\mathbf{X})</math> and <math>\bar{D}_k(\mathbf{X})</math></b> | <b>23</b> |
| <b>D</b> | <b>Second Order Approximations</b>                                                                           | <b>24</b> |
| <b>E</b> | <b>Variance Estimation</b>                                                                                   | <b>28</b> |
| <b>F</b> | <b>A General Convergence Theorem Under <math>\alpha</math>-Mixing</b>                                        | <b>30</b> |
| <b>G</b> | <b>Additional Methods for Joint Hypothesis Testing</b>                                                       | <b>32</b> |
| G.1      | Combining Results for Several Individuals with One Statistic . . . . .                                       | 33        |
| G.2      | Combining the Results of Several Joint Test Statistics . . . . .                                             | 34        |
| G.3      | Power Simulations . . . . .                                                                                  | 34        |
| G.4      | Application to GVT . . . . .                                                                                 | 34        |

|          |                                                                                      |           |
|----------|--------------------------------------------------------------------------------------|-----------|
| <b>H</b> | <b>Asymptotic Power Approximations for General <math>m</math> and <math>k</math></b> | <b>36</b> |
| <b>I</b> | <b>Asymptotic Equivalence to the Wald-Wolfowitz Runs Test</b>                        | <b>41</b> |
| <b>J</b> | <b>Permutation Tests of Individual Hypotheses <math>H_0^i</math> in GVT</b>          | <b>43</b> |
| <b>K</b> | <b>Proofs of Theorems Presented in the Main Text</b>                                 | <b>48</b> |
| K.1      | Proof of Theorem 3.1 . . . . .                                                       | 48        |
| K.2      | Proof of Theorem 3.2 . . . . .                                                       | 52        |
| K.3      | Proof of Theorem 3.3 . . . . .                                                       | 53        |
| K.4      | Proof of Theorem 3.4 . . . . .                                                       | 60        |
| K.5      | Proof of Theorem 4.1 . . . . .                                                       | 63        |

## A Application to Two Problems in Empirical Finance

In this section, we outline the application of the permutation tests that we study and our asymptotic approximations to their power to two problems in Empirical Finance. First, we apply the permutation tests that we develop to test the weak form efficient market hypothesis in the spirit of Fama (1965). Second, we discuss the application of these methods to tests of persistence in the performance of mutual funds relative to benchmark portfolios.

### A.1 Tests of the Weak Form Efficient Market Hypothesis

There is a large literature in finance that aims to assess weak-form market efficiency by studying the serial dependence in asset returns (Fama, 1970; Malkiel, 2003). In a classical analysis, Fama (1965) argues that tests of the randomness of sequences of stock returns give tests of the weak-form efficient market hypothesis.<sup>1</sup> He concludes that there is limited evidence of serial dependence, but makes no formal quantification of uncertainty.

In this Section, we briefly discuss a component of Fama’s analysis, outline the application of the methods that we develop to this problem, and provide an example of their implementation on two datasets of sequences of stock prices. In our discussion, we will assume that the reader is familiar with the results developed in Sections 2, 3, and 4 of the main text. Our goal is not to break theoretical or empirical ground, but to provide an additional illustration of our methods.

#### A.1.1 Discussion of Fama (1965)

Fama (1965) studies approximately five years of daily prices for each of thirty stocks on the Dow-Jones Industrial Average (DJIA). In Section 5 of his paper, Fama tests the independence of the signs of log price changes at one, four, nine, and sixteen trading-day intervals. In particular, Fama compares the observed number of runs of the signs of log price changes (i.e., the number of times that the sign of a log price change switches on consecutive intervals) to the expected number of runs under i.i.d. sampling for each stock. Although there is no formal quantification of uncertainty, Fama finds that there are more runs of signs of log price changes than would be expected under i.i.d. sampling at daily intervals, but that the observed and expected number of runs of signs of log price changes are very close for four, nine, and sixteen trading-day price intervals.

#### A.1.2 Methods

The statistical framework and inferential methods developed in the main text are applicable to this problem. In fact, in Online Appendix I.1 we show that the test applied by Fama – the Wald and Wolfowitz (1940a) runs test – is asymptotically equivalent to the individual permutation tests that we develop in Section 3 of the main text with the test statistics  $\hat{D}_{n,k}(\mathbf{X}_i)$  and  $\hat{P}_{n,k}(\mathbf{X}_i) - \hat{p}_{n,i}$  with  $k = 1$ , defined in (2.4) and (2.5) of the main text. Our asymptotic power approximations, derived

---

<sup>1</sup>This analysis is extremely influential, holding 13,106 Google scholar citations on September 3<sup>rd</sup> 2020.

in Section 4, allow us to analyze the power of our methods – and the Wald-Wolfowitz Runs test – applied to this setting against particular alternatives.

Specifically, suppose that we observe price sequences for  $s$  stocks. Each observation of a price is separated from its two adjacent price observations by a time interval  $t$ , e.g., if  $t$  equals four trading days we say that prices are observed with a time interval of four trading-days. For each stock, we observe prices for  $n + 1$  consecutive time intervals. Let  $\{v_{ij}\}_{j=1}^{n+1}$  denote the vector of observed prices for stock  $i$ .

Following Fama (1965), we test the null hypotheses that the sequences of the signs of log price changes are independent and identically distributed for each stock. Formally, let

$$X_{ij} = \begin{cases} 1 & \text{if } \log(v_{i(j+1)}) - \log(v_{ij}) > 0 \\ 0 & \text{otherwise,} \end{cases}$$

$\mathbf{X}_i = \{X_{ij}\}_{j=1}^n$ , and  $\mathbf{X} = \{\mathbf{X}_i\}_{i=1}^s$ . We are interested in testing the individual null hypotheses

$$H_0^i : \mathbf{X}_i \text{ is i.i.d.}$$

against alternatives in which the parameters  $\theta_P^k(\mathbb{P}_i)$  and  $\theta_D^k(\mathbb{P}_i)$ , defined in (2.2) and (2.3) in the main text, are not equal to zero for some integer  $k$ .<sup>2</sup> We assume  $\mathbf{X}_i$  follows a stationary Bernoulli( $p_i$ ) process  $\mathbb{P}_i$  for each  $i$ .

Additionally, we estimate and construct confidence intervals for the parameters  $\theta_P^k(\mathbb{P}_i)$  and  $\theta_D^k(\mathbb{P}_i)$ . We estimate these parameters with the estimators  $\tilde{P}_{n,k}(\mathbf{X}_i)$  and  $\tilde{D}_{n,k}(\mathbf{X}_i)$ , defined in (3.3) in the main text, respectively. These estimators are bias-corrected under the joint null hypothesis  $H_0$ . We construct confidence intervals for  $\theta_P^k(\mathbb{P}_i)$  and  $\theta_D^k(\mathbb{P}_i)$  with

$$\tilde{P}_{n,k}(\mathbf{X}) \pm \sigma_P(\hat{p}_{n,i}, k) \frac{z_{1-\alpha/2}}{\sqrt{n}} \quad (\text{A.1})$$

and

$$\tilde{D}_{n,k}(\mathbf{X}_i) \pm \sigma_D(\hat{p}_{n,i}, k) \frac{z_{1-\alpha/2}}{\sqrt{n}}, \quad (\text{A.2})$$

respectively. These confidence intervals are valid under stationary alternatives contiguous to  $H_0$ .

In our main application to controlled basketball shooting experiments, when implementing tests of the joint null hypothesis

$$H_0 : \mathbf{X}_i \text{ is i.i.d. for each } i \text{ in } 1, \dots, s,$$

we operate under the assumption that the individual shooting sequences  $\mathbf{X}_i$  are independent across

---

<sup>2</sup>Note that in our application to controlled basketball shooting experiments, we consider alternatives in which  $\theta_P^k(\mathbb{P}_i)$  and  $\theta_D^k(\mathbb{P}_i)$  are positive (i.e “streaky” alternatives) because these alternatives are implied by models of the “belief in the law of small numbers”. In this case, the theory that we are testing does not discipline the signs of the alternatives that we are testing against. Thus, we consider two sided alternatives. For two-sided alternatives,  $p$ -values can be estimated by taking two times the minimum of the two one-sided  $p$ -values.

individuals. In this setting, the equivalent assumption – that  $\mathbf{X}_i$  are independent across stocks – is not realistic, as companies will be exposed to common macroeconomic or sectoral shocks. Thus, the methods for joint hypothesis testing developed in Sections 3 and 4 of the main text provide a test of the hypotheses that the sequences  $\mathbf{X}_i$  are i.i.d. *and* independent across stocks, which is significantly stronger than the weak-form efficient market hypothesis. Hence, we do not apply these methods in this section.<sup>3</sup>

However, the methods that we develop for testing the individual hypotheses  $H_0^i$ , and our approximations to their power, are applicable to this context and are of substantive interest. In most of his analyses, Fama (1965) displays statistics computed for all of the individual stocks separately or highlights statistics computed on individual stocks. Moreover, a rejection of an individual hypothesis  $H_0^i$ , robust to correction for multiple testing, is strong evidence against weak-form market efficiency.<sup>4</sup>

In fact, for this application, simultaneous tests of the individual hypotheses  $H_0^i$  are arguably of greater interest than joint tests of  $H_0$ . Specifically, Fama (1965) aims to assess whether there is information in past price patterns that can be leveraged profitably by investors. If an investor is able to leverage deviations in randomness in stock price profitably, then necessarily they have been able to identify *which* stocks deviate from randomness; knowing only that there exists some non-random stocks is insufficient.

### A.1.3 Data

We construct two datasets of sequences of stock prices.

**Panel of Daily Prices for DJIA Components:** In the spirit of Fama (1965), we collect a dataset of daily prices for 30 stocks on the Dow Jones Industrial Average (DJIA) between January 1<sup>st</sup>, 2000 and December 31<sup>st</sup>, 2019. To construct this dataset, we obtain a list of the 30 stocks that composed the DJIA on April 2<sup>nd</sup>, 2019.<sup>5</sup> In this list, we replace Visa with Hewlett-Packard, as Visa had its initial public offering on March 19<sup>th</sup>, 2008 and replaced Hewlett-Packard in the DJIA in 2013. To obtain a complete panel, we make a set of assumptions concerning the changes of

---

<sup>3</sup>One approach to a randomization test for  $H_0$  that imposes weaker restrictions on the dependence between the sequences  $\mathbf{X}_i$  for different companies, would be to apply the same permutation to each  $\mathbf{X}_i$  when recomputing joint test statistics. This imposes the restriction that  $X_{i,j}$  and  $X_{i',j'}$  are independent for  $i \neq i'$  and  $j \neq j'$ . It may be possible to apply the arguments developed in Sections 3 and 4 to approximate the power of this methods, but this is beyond the scope of our analysis.

<sup>4</sup>Again, the method for simultaneous inference on the individual hypotheses  $H_0^i$ , outlined in Section 3.2 applied in our analysis of controlled basketball shooting experiments, assumes that the tests of  $H_0^i$  are independent. As this is not the case in this setting, we apply the standard Bonferroni correction., i.e.,  $p$ -values are compared to  $\alpha/s$  rather than to  $\alpha$ . For more powerful tests, the stepdown method of Romano and Wolf (2005) can be considered, but this is beyond the scope of our analysis in this section.

<sup>5</sup>This list was derived from the map of securities on the DJIA available at <https://us.spindices.com/indexology/djia-and-sp-500/the-changing-djia>, accessed on September 1<sup>st</sup>, 2020.

stock ticker names coincident with mergers, acquisitions, and spin-offs.<sup>6</sup> Data on daily closing prices (or bid/ask averages if closing prices are unavailable) for these stocks for active trading days between January 1<sup>st</sup>, 2000 and December 31<sup>st</sup>, 2019 are obtained from the CRSP (2020) Daily Stock Security Files through the Wharton Research Data Services (WRDS). Closing prices and bid/ask averages are treated identically. Holidays and weekends are treated the same as consecutive trading days, e.g., Fridays and Mondays are treated as consecutive trading-days.

Again, following Fama (1965), we construct panels of the signs of log price changes with one, four, nine, and sixteen trading-day intervals between consecutive prices. We begin each panel on the earliest observed trading day (January 3<sup>rd</sup>, 2000). These are considerably larger panels than were analyzed in Fama (1965), who studied approximately five years of data. There are 5030, 1257, 558, and 314 observations of the sign of log price change  $X_{ij}$  at one, four, nine, and sixteen trading-day intervals for each stock, respectively.

**Intraday Prices for the DJIA Index:** In order to obtain a larger sample than the panel of daily prices, and to consider a setting without the constraints of multiple comparisons, we acquire a dataset with minute by minute closing prices for the DJIA index between May 1<sup>st</sup>, 2007 and September 2<sup>nd</sup>, 2020 from FirstRate Data.<sup>7</sup> We treat end-of-day closing prices as adjacent to beginning of day closing prices, i.e., we append the daily price sequences to make one long sequence. For this dataset, to maximize power and for the sake of parsimony of presentation, we only consider panels with one minute time intervals. We consider the sequence of prices for the year 2010. There are 101,969 observations of the sign of log price change  $X_j$  for this sample (we omit the subscript  $i$  as there is only one sequence).

#### A.1.4 Results

**Panel of Daily Prices for DJIA Components:** Figure 1 displays  $p$ -values of the individual permutation tests that use the test statistics  $\hat{D}_{n,k}(\mathbf{X}_i)$  and  $\hat{P}_{n,k}(\mathbf{X}_i) - \hat{p}_{n,i}$ , defined in (2.4) and (2.5), for each interval and each  $k$  in  $1, \dots, 4$  for the panel of daily prices of DJIA components. The  $p$ -values for tests that use  $\hat{D}_{n,k}(\mathbf{X}_i)$  and  $\hat{P}_{n,k}(\mathbf{X}_i) - \hat{p}_{n,i}$  are displayed in green and blue, respectively. The  $x$ -axis is displayed with a log scale base 10. Vertical black lines are placed at 0.05, 0.1/30, and 0.05/30. As there are 30 stocks in our sample, an estimated  $p$ -value less than  $\alpha/30$

<sup>6</sup>We associate Chevron with the ticker CHV for January 1<sup>st</sup>, 2000 through October 9<sup>th</sup>, 2001 and with CVX for the remainder of the panel. We associate Verizon with the ticker BEL for January 1<sup>st</sup>, 2000 through June 30<sup>th</sup>, 2000 and with VZ for the remainder of the panel. We associate The Travelers Companies with the tickers SPC for January 1<sup>st</sup>, 2000 through April 1<sup>th</sup>, 2004, STA for April 2<sup>th</sup>, 2004 through February 26<sup>th</sup>, 2007, and TRV for the remainder of the panel. We associate Walgreens Boots Alliance with the ticker WAG for January 1<sup>st</sup>, 2000 through December 30<sup>th</sup>, 2014 and WBA for the remainder of the sample. We associate Dow with the tickers DD for January 1<sup>st</sup>, 2000 through August 31<sup>st</sup>, 2017, DWDP for September 1<sup>st</sup>, 2017 through May 31<sup>st</sup>, 2019, and DOW for the remainder of the sample. We associate Hewlett-Packard with the ticker HWP for January 1<sup>st</sup>, 2000 through May 3<sup>rd</sup>, 2002 and with HPQ for the remainder of the sample.

<sup>7</sup>The data were purchased from FirstRate Data (2020) on September 3<sup>rd</sup>, 2020.

indicates a rejection of the individual null hypothesis  $H_0^i$  with the Bonferroni method with control of the familywise error rate at level  $\alpha$ .

No individual hypothesis is rejected by the Bonferroni method at level  $\alpha = 0.05$  or  $0.1$ . Overall, the  $p$ -values increase as the trading-day interval increases and as  $k$  increases. Six and four individual hypotheses have  $p$ -values less than  $0.05$  for the tests using  $\hat{D}_{n,k}(\mathbf{X}_i)$  and  $\hat{P}_{n,k}(\mathbf{X}_i) - \hat{p}_{n,i}$  for  $k = 1$  with single trading-day intervals, respectively. Again, the number of individual hypothesis with  $p$ -values less than  $0.05$  decrease as  $k$  increases and the trading-day interval increases. These results broadly match the conclusions of Fama (1965), who notes some weak evidence against randomness for daily trading intervals and no indication of deviations from randomness for longer trading-day intervals.

**Intraday Prices for the DJIA Index:** Panel A of Figure 2 overlays the realized values of  $\hat{D}_{n,k}(\mathbf{X})$  and  $\hat{P}_{n,k}(\mathbf{X}) - \hat{p}_{n,i}$  for the sequence of one minute DJIA index intraday prices for each  $k$  in  $1, \dots, 4$  on their permutation distributions, displayed with horizontal black to white gradients. The 2.5<sup>th</sup> and 97.5<sup>th</sup> quantiles of these distributions are denoted by vertical blue and green lines, respectively. The observed statistics are denoted with vertical black lines. The two-sided  $p$ -values of the permutation tests are displayed to the right of the corresponding permutation distributions. For  $\hat{D}_{n,k}(\mathbf{X})$ , there is a strong rejection of the null hypothesis  $H_0$  for each  $k$ . For  $\hat{P}_{n,k}(\mathbf{X}) - \hat{p}_{n,i}$ , there is a strong rejection of the null hypothesis with  $k = 1$ , but the  $p$ -value increases with  $k$ .

Panel B of Figure 2 plots the realizations of the estimators  $\hat{P}_{n,k}(\mathbf{X})$  and  $\tilde{D}_{n,k}(\mathbf{X})$  for the one minute DJIA Index intraday price sequence and the normal approximation confidence intervals, given in expressions (A.1) and (A.2), for each  $k$  in  $1, \dots, 4$ . The values of the realizations of  $\hat{P}_{n,k}(\mathbf{X})$  and  $\tilde{D}_{n,k}(\mathbf{X})$  are displayed to the right of the corresponding confidence intervals. These estimates increase with  $k$  for  $\tilde{D}_{n,k}(\mathbf{X})$  and decrease with  $k$  for  $\hat{P}_{n,k}(\mathbf{X})$ .

### A.1.5 Power

In Section 4 of the main text, we obtain an asymptotic approximation to the power of tests of the hypotheses  $H_0^i$  using the individual test statistics  $\hat{P}_{n,k}(\mathbf{X}_i) - \hat{p}_{n,i}$  and  $\hat{D}_{n,k}(\mathbf{X}_i)$ , defined in (2.4) and (2.5) of the main text, against a specific Markov chain alternative.

We make a series of conservative assumptions to obtain rough upper bounds to the power of these tests implemented on the two datasets outlined in Online Appendix Section A.1.3. To discipline this exercise, we inspect the unconditional distributions the means of the signs of the log price changes  $X_{ij}$  over given time intervals. First, we compute the mean of the signs of the log price changes  $X_{ij}$  for each stock  $i$  in each of the twenty years in each of our four panels of daily prices for DJIA components, i.e., we compute the proportion of positive log price increases for each stock in each year at each interval. Table 1 displays quantiles of the distributions of these statistics for each interval, taken over the collection of stocks and years. Second, we compute the

Online Appendix Figure 1: Permutation Tests of Individual Null Hypothesis  $H_0^i$  for the Panel Daily Prices for DJIA Components

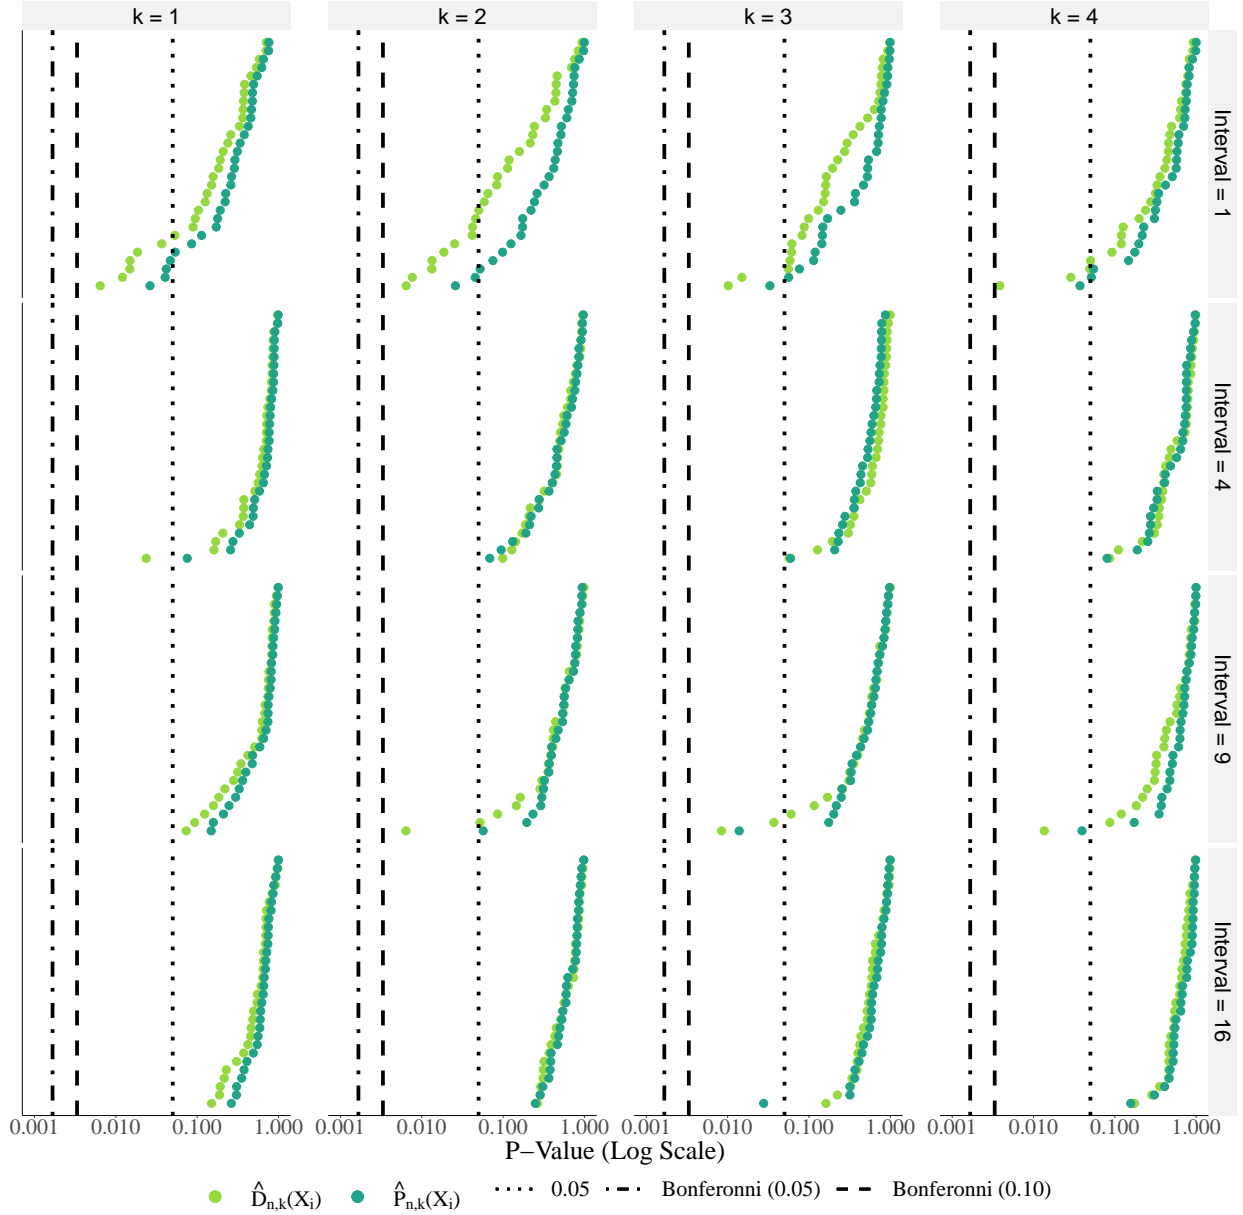

Notes: Figure displays two-sided  $p$ -values for the individual permutation tests using the test statistics  $\hat{D}_{n,k}(\mathbf{X}_i)$  and  $\hat{P}_{n,k}(\mathbf{X}_i) - \hat{p}_{n,i}$  for each  $k$  in  $1, \dots, 4$  and for each choice of interval length. The  $p$ -values computed using  $\hat{D}_{n,k}(\mathbf{X}_i)$  are displayed in green and the  $p$ -values using  $\hat{P}_{n,k}(\mathbf{X}_i) - \hat{p}_{n,i}$  are displayed in blue. The  $x$ -axis is displayed with a log scale base 10. The black vertical dotted line denotes 0.05. The black vertical dashed and dot-dashed lines denote the thresholds for rejection of the individual hypotheses with the Bonferroni multiple testing correction at level 0.1 and 0.05, respectively. We estimate the permutation distribution of  $\hat{D}_{n,k}(\mathbf{X}_i)$  and  $\hat{P}_{n,k}(\mathbf{X}_i) - \hat{p}_{n,i}$  under  $H_0^i$  by permuting each of the  $\mathbf{X}_i$ 's 100,000 times separately and recomputing  $\hat{D}_{n,k}(\mathbf{X}_i)$  and  $\hat{P}_{n,k}(\mathbf{X}_i) - \hat{p}_{n,i}$  for each permuted collection of sequences. The  $p$ -values are computed by taking 2 times the minimum the proportions of recomputed statistics smaller than and larger than the observed values of  $\hat{D}_{n,k}(\mathbf{X}_i)$  and  $\hat{P}_{n,k}(\mathbf{X}_i) - \hat{p}_{n,i}$ .

Online Appendix Figure 2: Permutation Tests of the Individual Null Hypothesis  $H_0$  and Normal Approximation Confidence Intervals for  $\theta_P^k(\mathbb{P})$  and  $\theta_D^k(\mathbb{P})$  for One Minute DJIA Index Intraday Prices

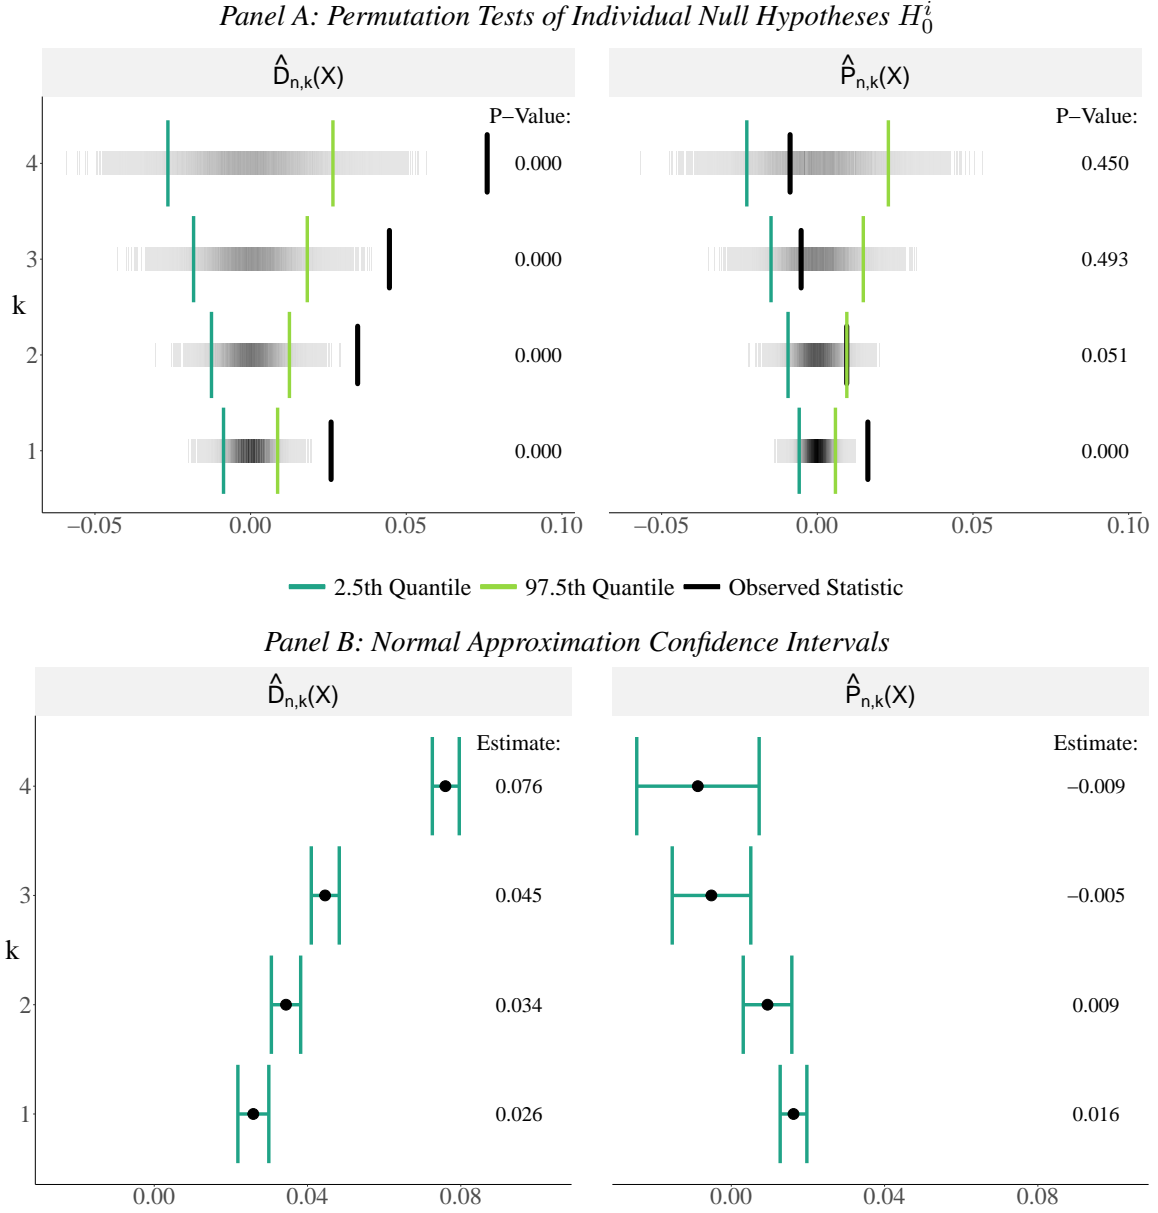

Notes: Panel A displays the observed values of  $\hat{D}_{n,k}(\mathbf{X})$  and  $\hat{P}_{n,k}(\mathbf{X}) - \hat{p}_{n,i}$  for the one minute DJIA Index Intraday Prices overlaid onto their permutation distributions under  $H_0$  for each  $k$  in  $1, \dots, 4$ . The observed values of  $\hat{D}_{n,k}(\mathbf{X})$  and  $\hat{P}_{n,k}(\mathbf{X}) - \hat{p}_{n,i}$  are indicated by black vertical line segments. The estimated 2.5<sup>th</sup> and 97.5<sup>th</sup> quantiles of the permutation distributions are denoted by vertical line segments, respectively. We estimate the permutation distributions with 100,000 permutations. The estimates of the permutation distributions are displayed in horizontal white to black gradients. The  $p$ -values of the two-sided test of  $H_0$ , computed as 2 times the minimum the proportions of recomputed statistics smaller than and larger than the observed values of  $\hat{D}_{n,k}(\mathbf{X})$  and  $\hat{P}_{n,k}(\mathbf{X}) - \hat{p}_{n,i}$ , are reported to the right of each distribution. Panel B displays the observed values of  $\hat{P}_{n,k}(\mathbf{X})$  and  $\hat{D}_{n,k}(\mathbf{X})$  for the one minute DJIA Index Intraday Prices and the normal approximation confidence intervals given in expressions (A.1) and (A.2) for each  $k$  in  $1, \dots, 4$ .

| Interval | Quantile |       |       |       |       |
|----------|----------|-------|-------|-------|-------|
|          | .25      | .33   | .50   | .66   | .75   |
| 1        | 0.486    | 0.494 | 0.508 | 0.524 | 0.536 |
| 4        | 0.492    | 0.500 | 0.524 | 0.556 | 0.571 |
| 9        | 0.481    | 0.500 | 0.556 | 0.593 | 0.607 |
| 16       | 0.467    | 0.500 | 0.563 | 0.625 | 0.625 |

Online Appendix Table 1: Quantiles of the Distributions of the Yearly Proportions of Positive Log Price Changes at Different Time Intervals for Thirty Stocks in the DJIA

Notes: Table displays quantiles of the distributions of the yearly proportions of daily positive log price changes for thirty stocks on the DJIA between 2000-2020. For each stock at each interval, we compute the proportion of positive log price increases in each year. The Table gives the quantiles of the distributions of these proportions for each interval, taken over the collection of stocks and years.

mean of signs of the log price changes  $X_j$  for the sequence of one minute DJIA Index Intraday prices in each trading-day between 2010 and 2020. Table 2 displays quantiles of the distributions of these statistics for each interval, taken over days.

Suppose that for each stock in the sample, the unconditional probability of a positive log price change is one half. By inspection of Tables 1 and 2, this assumption appears to be reasonably accurate for most stocks in the daily panel and for the intraday index. Furthermore, suppose the stocks have a  $100 \cdot \epsilon\%$  higher (lower) probability of a positive log price change after  $m$  consecutive positive (negative) log price changes than they would unconditionally. This is an instance of the Markov chain alternative model of a “streaky” individual developed in the main text in Section 4.1.

Figure 3 displays our asymptotic approximation to the power of the permutation test of an individual hypothesis  $H_0^i$  at level  $\alpha = 0.05$  using the test statistic  $\hat{D}_{n,k}(\mathbf{X}_i)$  against this alternative over a grid of  $\epsilon$ , for  $m = k$  for  $k$  in  $1, \dots, 4$ , and for  $n$  equal to its value for the panels of daily prices of DJIA components constructed at each interval. Without placing further restrictions on the dependence between the sequences  $\mathbf{X}_i$ , this is a strict upper bound to the probability of rejecting at least one null hypothesis  $H_0^i$  with the Bonferroni method with control of the familywise error rate at level  $\alpha = 0.05$ . Figure 3 displays an analogous figure for the sequence of intraday prices for the DJIA index.

In both cases, we target power against two values of  $\epsilon$ . The vertical dotted line denotes the value of  $\epsilon$  that corresponds to half the distance between the 33<sup>rd</sup> and 66<sup>th</sup> quantiles of the distributions of the proportions of positive log price changes at each interval displayed in Tables 1 and 2. The vertical dot-dashed line gives the equivalent distance between the 25<sup>th</sup> and 75<sup>th</sup> quantiles. As we are not fundamentally interested in targeting deviations from randomness that occur after streaks of a given length, we consider  $m = 1$  as a benchmark. Note that the limiting power of tests with  $k = 1$  is equal to the limiting power of the Wald-Wolfowitz runs test, applied implicitly in Fama (1965).

| Quantile |       |       |       |       |
|----------|-------|-------|-------|-------|
| .25      | .33   | .50   | .66   | .75   |
| 0.415    | 0.427 | 0.444 | 0.462 | 0.474 |

Online Appendix Table 2: Quantiles of the Distributions of the Daily Proportions of Positive Log Price Changes at One Minute Intervals for the DJIA Index

Notes: Table displays quantiles of the distributions of the daily proportions of one minute positive log price changes for the DJIA index between 2010-2020. We compute the proportion of one minute positive log price increases in each day. The Table gives the quantiles of the distributions of these proportions for each interval, taken over the collection of stocks and years.

In the case of the panel of daily prices for DJIA components, individual tests of  $H_0^i$  with  $m = k = 1$  have relatively large power, particularly for the larger value of  $\epsilon$ . This power decreases rapidly as  $k$  and  $m$  increase. Thus, the individual hypothesis tests implemented in the Online Appendix Section A.1.4 on this dataset – considered in isolation – have reasonable power against alternatives consistent with the variation in stock returns with  $m$  and  $k$  equal to one. As the tests of  $H_0^i$  are not perfectly dependent, the power of the multiple hypothesis test of the thirty hypotheses  $H_0^i$  against these alternatives will likely be considerably smaller. As the panel of daily prices that we have constructed in this Section is at least four times as large as the panel studied in Fama (1965), this result indicates that the simultaneous analysis in Fama (1965) is underpowered.

In the case of the sequence of intraday prices for the DJIA index, the test of the individual hypothesis  $H_0$  has power very close to one for  $m = k$  between 1 and 4 against both of the values of  $\epsilon$  that we consider. This exercise highlights the fact that very large datasets are necessary for individual tests to have substantial power.

## A.2 Tests of Persistence in the Performance of Mutual Funds

The objective of a large literature in empirical finance is to determine whether there is persistence in the performance of particular mutual funds relative to market indices (Jensen, 1968; Hendricks et al., 1993; Carhart, 1997). Motivated by the literature on the hot hand fallacy, Hendricks et al. (1993) specifically aim to assess whether mutual fund managers “delivering sustained short-run superior performance have ‘hot hands’,” noting evidence from Hendricks et al. (1997) documenting that investors move their money to funds that have performed well relative to benchmarks in recent periods. They argue that if they are unable to reject the null hypothesis that there is persistence in the performance of mutual funds relative to market indices, then these patterns in investment provide evidence of systematic misperception of randomness consistent with the hot hand fallacy.

Hendricks et al. (1993) study the quarterly returns for 165 growth-oriented mutual funds between 1974 and 1988. The number of funds observed each quarter varies and diminishes over time. The number of observations of quarterly returns per mutual fund is at most 56. In robust-

Online Appendix Figure 3: Power of Joint Tests of  $H_0$  Using  $\bar{D}_k(\mathbf{X})$  Against the Markov Chain Streaky Alternative with  $k = m$  by Interval Length for the Panel Daily Prices for DJIA Components

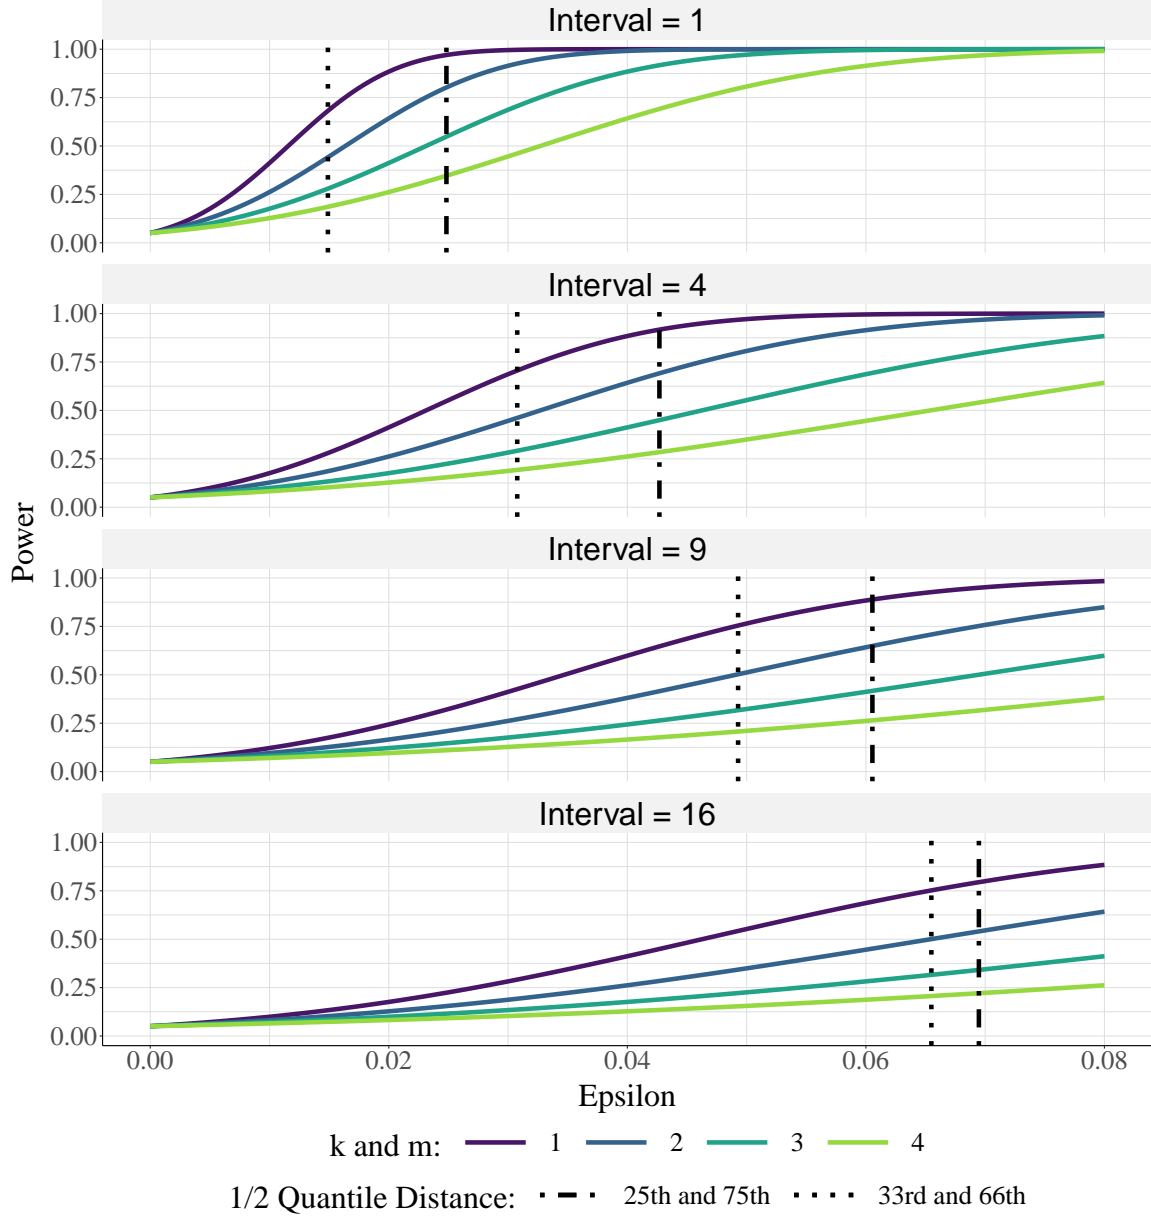

Notes: Figure displays asymptotic approximations to the power of the stratified permutation tests of the joint null hypothesis  $H_0$  using the test statistic  $\bar{D}_{n,k}(\mathbf{X}_i)$  against the Markov chain streaky alternative specified in Section 4.1 of the main text over a grid of  $\epsilon$ , for  $m = k$  for  $k$  in  $1, \dots, 4$ , and for  $n$  equal to its value for the panels of daily prices of DJIA components constructed at each interval. An expression for this asymptotic approximation is given in Online Appendix Corollary H.3, with  $h = \epsilon\sqrt{n}$ . The vertical dotted and dot-dashed lines denote the value of  $\epsilon$  that correspond to half the distance between the 33<sup>rd</sup> and 66<sup>th</sup> quantiles and the 25<sup>th</sup> and 75<sup>th</sup> quantiles of the distributions of the yearly proportions of positive log price changes at each interval.

Online Appendix Figure 4: Power of Joint Tests of  $H_0$  Using  $\bar{D}_k(\mathbf{X})$  Against the Markov Chain Streaky Alternative with  $k = m$  by Interval Length for One Minute DJIA Index Intraday Prices

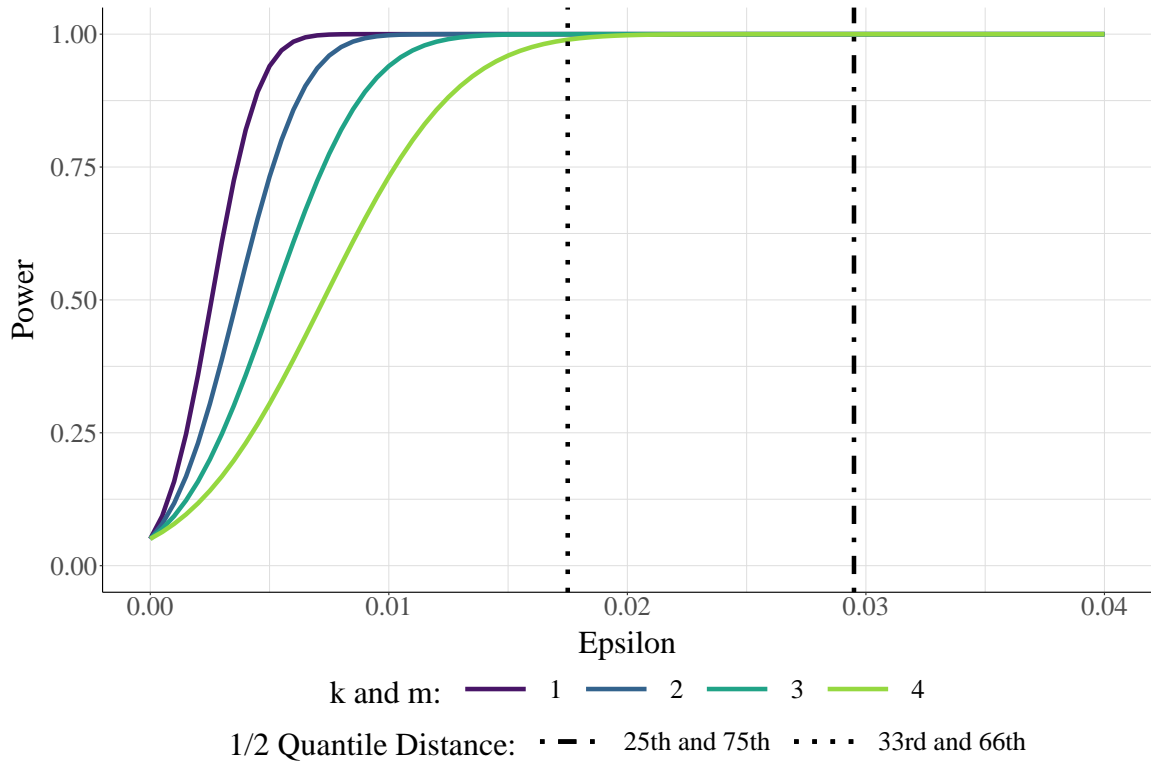

Notes: Figure displays asymptotic approximations to the power of the stratified permutation tests of the joint null hypothesis  $H_0$  using the test statistic  $\bar{D}_{n,k}(\mathbf{X}_i)$  against the Markov chain streaky alternative specified in Section 4.1 of the main text over a grid of  $\epsilon$ , for  $m = k$  for  $k$  in  $1, \dots, 4$ , and for  $n$  to its value for sequence of intraday prices for the DJIA index. An expression for this asymptotic approximation is given in Online Appendix Corollary H.3, with  $h = \epsilon\sqrt{n}$ . The vertical dotted and dot-dashed lines denote the value of  $\epsilon$  that correspond to half the distance between the 33<sup>rd</sup> and 66<sup>th</sup> quantiles and the 25<sup>th</sup> and 75<sup>th</sup> quantiles of the distributions of the daily proportions of one minute positive log price changes.

ness checks, they examine selected subsamples of this data. They find that there is positive and significant short-term persistence, but that this persistence diminishes over longer intervals.<sup>8</sup>

While Hendricks et al. (1993) measure persistence by computing the autocorrelation of the difference between the returns to each fund and the returns to an index, our methods are applicable to this setting, albeit with a somewhat different approach and interpretation. Rather than considering makes and misses in basketball shooting, one can consider a indicator variable for whether a mutual fund beats an index. Our asymptotic power approximations derived in Section 4 allow us to analyze the power of the permutation tests that we study in this application.

Tests of the individual hypotheses  $H_0^i$  – that the sequences of indicators for whether mutual fund  $i$  beats an index – against alternatives in which  $\theta_P^k(\mathbb{P}_i)$  and  $\theta_D^k(\mathbb{P}_i)$ , defined in (2.2) and (2.3) of the main text, are greater than zero assess whether the performance of the manager of mutual fund  $i$  deviates from randomness. The methods that we develop in Section 3 for testing the joint null hypotheses  $H_0$  assess whether the performance of any mutual fund manager deviates from randomness *and* whether the performance of mutual fund managers is dependent across managers. The latter hypothesis – independence in relative returns across managers – is perhaps less contentious than its equivalent in the case of the stock price sequences considered in Online Appendix A.1, but is substantially less convincing than its equivalent in the case of controlled basketball shooting experiments.

Similarly to the case of the stock price sequences considered in Online Appendix A.1, the multiple comparison problem is potentially of greater interest in this setting than the joint hypothesis  $H_0$ . If investors are able to successfully determine which mutual fund managers “have the hot hand”, then they necessarily can identify which mutual funds have performance records that deviate from randomness.

We make a series of conservative assumptions to obtain an upper bound to the power of individual tests applied to this problem. Suppose that for all mutual funds in the sample, the unconditional probability that they beat the index is one half. From Table A.II of the Appendix to Hendricks et al. (1993), we can see that average over mutual funds of the average quarterly differences between the returns to each mutual fund and two indices (Jensen’s  $\alpha$ ) are  $-0.28\%$  and  $-1.25\%$  with interquartile ranges of  $1.24\%$  and  $1.48\%$ . Thus, our assumption appears to be approximately true for one index (the value weighted CRSP index of NYSE and AMEX stocks) and is an overestimation for the other index (the equally weighted CRSP index of NYSE stocks). Furthermore, suppose that mutual funds have a  $5\%$  higher (lower) probability of beating the index following a period in which they beat (lost to) the index. Ideally, we would like to compute the distribution of the proportion of the time that each fund beats the index to inform these parameter choices, but this information is not readily available. Finally, we take an upper bound by assuming that we observe 56 daily prices for each stock.

The power of permutation tests of the individual hypotheses  $H_0^i$  that we consider with the best suited choice of test statistic implemented on a sequence of returns for one mutual fund in the data

---

<sup>8</sup>However, Carhart (1997), who constructs a significantly larger data set of mutual fund returns, argues that persistent performance is explained almost entirely by persistent differences in mutual fund expenses and transaction costs.

consider in Hendricks et al. (1993) is approximately 0.19. If we assume that the relative performance of mutual funds is independent across funds, then the power of the stratified permutation test of the joint null hypothesis  $H_0$  against this alternative is 0.99. This remains the case if the proportion of funds that deviate from randomness is reduced to 0.5. While it is beyond the scope of our analysis to provide a more detailed justification of alternatives, this exercise highlights the value of developing methods for joint testing in settings with possible dependence across individuals.

## B Dynamic Potential Outcome Notation

In this section, we study the relationship between testing the randomness of a stationary Bernoulli sequence and testing whether there is a causal effect of an outcome in previous periods on the current period's outcome in a Bernoulli process. In Section B.1, we show that these conditions are equivalent under an unconfoundedness type condition. In Section B.2, we show that stationary and  $\alpha$ -mixing alternatives are a natural class of alternatives to consider for this problem. In Section B.3, we specify the Markov chain alternatives studied in Section 4 of the main text with the dynamic potential outcomes notation studied in this section. We confine our consideration to the case with  $s = 1$ , and therefore drop the dependence on the individual  $i$ .

Define the potential outcome sequence

$$\mathbf{U}(\cdot) = \left( U_j(\cdot) = \{U_j(x)\}_{x \in \{0,1\}^m}, j \in \mathbb{Z}_+ \right)$$

such that  $U_j(x)$  is a Bernoulli random variable for every  $j$  and  $x$ . That is,  $\mathbf{U}(\cdot)$  is a  $2^m$ -vector valued Bernoulli process. Let the observed outcome sequence be defined recursively as

$$\begin{aligned} \mathbf{X} &= \left( \sum_{x \in \{0,1\}^m} U_j(x) \mathbb{I}\{(X_{j-1}, \dots, X_{j-m}) = x\}, j > m \right) \\ &= (U_j(X_{j-1}, \dots, X_{j-m}), j > m). \end{aligned}$$

Define the parameters

$$\begin{aligned} SD_j(x, x') &= \mathbb{E}[U_j(x) - U_j(x')] \text{ and} \\ SD_j(x) &= \mathbb{E}[U_j(x) - X_j]. \end{aligned}$$

### B.1 Relationship Between Independence and State Dependence

We are interested in the relationship between the conditions

$$SD_j(x, x') = 0 \text{ for all } x, x' \in \{0, 1\}^m \text{ and } j \in \mathbb{Z}^+, \quad (\text{B.1})$$

$$SD_j(x) = 0 \text{ for all } x \in \{0, 1\}^m \text{ and } j \in \mathbb{Z}^+, \quad (\text{B.2})$$

and the independence and identical distribution of the observed outcome sequence. The assumptions that

$$\forall x \in \{0, 1\}^m, U_j(x) \perp X_{j-1}, \dots, X_1 \text{ and} \quad (\text{B.3})$$

$$\forall x \in \{0, 1\}^m, x' \in \{0, 1\}, \mathbb{P}(U_j(x) = x') \mathbb{P}(X_{j-1:j-m} = x) = \mathbb{P}(U_j(x) = x', X_{j-1:j-m} = x) \quad (\text{B.4})$$

are pivotal in the characterization of this relationship.

**Remark B.1.** The condition (B.3) can be thought of as analogous to the “unconfoundedness” and “stable unit treatment values” assumptions in the literature on causal inference (Rubin, 1990; Imbens and Rubin, 2015). In the language of our empirical application, the potential outcomes for a shot  $j$  are independent of the outcomes of the previous  $m$  shots (the treatment assignment) and are additionally independent of the outcomes of all other previous shots (the treatment assignments for other shots). ■

We refer to the first condition (B.1) as “weak no state dependence” and the second condition (B.2) as “strong no state dependence”. The relative strength of the no state dependence conditions obtains from the following remark and the subsequent example. The relative strength of the unconfoundedness conditions follows from Remark B.3 and Example B.2.

**Remark B.2.** Strong no state dependence implies weak no state dependence. Suppose that  $SD_j(x) = 0$  for all  $x \in \{0, 1\}^m$ . Then we have that

$$\mathbb{E}[U_j(x) - X_i] = \mathbb{E}[U_j(x') - X_i]$$

for all  $x, x' \in \{0, 1\}^m$  which implies that  $\mathbb{E}[U_j(x) - U_j(x')] = 0$  for all  $x, x' \in \{0, 1\}^m$  and thus  $SD_j(x, x') = 0$  for all  $x, x' \in \{0, 1\}^m$ .

However, the two conditions are equivalent if we assume that (B.4) holds. Suppose that  $SD_j(x, x') = 0$  for all  $x, x' \in \{0, 1\}^m$  and unconfoundedness holds, then we can see that for  $z \in \{0, 1\}$

$$\begin{aligned} \mathbb{P}(X_j = z) &= \sum_{x \in \{0, 1\}^m} \mathbb{P}(U_j(x) = z, X_{j-1:j-m} = x) \\ &= \sum_{x \in \{0, 1\}^m} \mathbb{P}(U_j(x) = z) \mathbb{P}(X_{j-1:j-m} = x) \quad (\text{Weak Unconfoundedness}) \\ &= \sum_{x \in \{0, 1\}^m} \mathbb{P}(U_j(x') = z) \mathbb{P}(X_{j-1:j-m} = x) \quad (\text{Weak No State Dependence}) \\ &= \mathbb{P}(U_j(x') = z), \end{aligned}$$

so  $SD_j(x) = 0$  for all  $x \in \{0, 1\}^m$ . ■

**Example B.1.** In general, weak no state dependence does not imply strong no state dependence. To see this, suppose that  $\mathbf{X}$  are independent and identically distributed Bernoulli with probability

of success  $p$  and  $m = 1$ . Set  $U_j(X_{j-1}) = X_j$  but set

$$\begin{aligned} U_j(1) &\stackrel{d}{\sim} \text{Bernoulli}(p + \eta_1) \text{ if } X_{j-1} = 0 \\ U_j(0) &\stackrel{d}{\sim} \text{Bernoulli}(p + \eta_0) \text{ if } X_{j-1} = 1. \end{aligned}$$

We can impose  $SD_j(x, x') = 0$  for all  $x, x' \in \{0, 1\}^m$  by choosing  $\eta_1$  and  $\eta_0$  such that  $\mathbb{P}(U_j(1) = 1) = \mathbb{P}(U_j(0) = 1)$ . Observe that

$$\begin{aligned} \mathbb{P}(U_j(1) = 1) &= p\mathbb{P}(X_{j-1} = 1) + (p + 2\eta_1)\mathbb{P}(X_{j-1} = 0) = p + \eta_1(1 - p) \\ \mathbb{P}(U_j(0) = 1) &= (p + 2\eta_0)\mathbb{P}(X_{j-1} = 1) + p\mathbb{P}(X_{j-1} = 0) = p + \eta_0 p. \end{aligned}$$

So, it must be the case that

$$\eta_1(1 - p) = \eta_0 p$$

So if  $p = 1/4$ , then  $\eta_0 = 3\eta_1$ . In that case, if  $\eta_0 = 1/8$ , then  $\mathbb{P}(U_j(0) = 1) = 3/8 \neq 1/4 = \mathbb{P}(X_j = 1)$  and  $SD_j(0) \neq 0$ . ■

**Remark B.3.** It is clear that unconfoundedness (B.3) implies weak unconfoundedness (B.4). Note that if  $m = 1$ , then (B.4) is equivalent to

$$\forall x \in \{0, 1\}, U_j(x) \perp X_{j-1}$$

as both  $\{X_{j-1} = x\}$  and  $\{X_{j-1} \neq x\}$  are independent of  $\{U_j(x) = x'\}$  for  $x, x' \in \{0, 1\}$ . ■

**Example B.2.** If  $\mathbf{X}$  is independent and identically distributed and there is strong no state dependence in the sense of (B.2), then the condition (B.4) does not in general imply (B.3). Consider  $m = 2$  and suppose that  $\mathbf{X}$  are independent and identically distributed Bernoulli with probability of success  $p$ . Set  $U_j(X_{j-1}) = X_j$  and

$$U_j(x, x') \stackrel{d}{\sim} \text{Bernoulli}(p) \text{ if } X_{j-1} = z, X_{j-2} = z'$$

for all  $x, x', z, z' \in \{0, 1\}$  except

$$\begin{aligned} U_j(0, 0) &\stackrel{d}{\sim} \text{Bernoulli}(p - \eta) \text{ if } X_{j-1} = 0, X_{j-2} = 1 \text{ and} \\ U_j(0, 0) &\stackrel{d}{\sim} \text{Bernoulli}(p + \eta) \text{ if } X_{j-1} = 1, X_{j-2} = 0. \end{aligned}$$

Observe that,

$$\mathbb{P}(U_j(x, x')) = p$$

for all  $x, x' \in \{0, 1\}$  and so there is strong no state dependence. In particular,

$$\mathbb{P}(U_j(0, 0) = 1) = p \cdot \mathbb{P}(X_{j-1} = 1, X_{j-2} = 1) + (p - \eta) \cdot \mathbb{P}(X_{j-1} = 0, X_{j-2} = 1)$$

$$\begin{aligned}
& + (p + \eta) \cdot \mathbb{P}(X_{j-1} = 1, X_{j-2} = 0) + p \cdot \mathbb{P}(X_{j-1} = 0, X_{j-2} = 0) \\
& = p.
\end{aligned}$$

However, as

$$\mathbb{P}(U_j(0, 0) = 1 | X_{j-1} = 0, X_{j-2} = 1) \neq p,$$

unconfoundedness (B.3) does not hold. ■

Neither strong nor weak no state dependence is equivalent to independence and identical distribution of the observed outcome sequence  $\mathbf{X}$ . In fact, neither condition implies the other. First, we show that under strong no state dependence, the observed outcome sequence  $\mathbf{X}$  can be any sequence. Second, we give an example that shows that if the observed outcome sequence  $\mathbf{X}$  is independent and identically distributed, then there can still be state dependence of either form.

**Theorem B.1.** *Strong no state dependence in the sense of (B.2) places no restriction on  $\mathbf{X}$ . That is,  $\mathbf{X}$  can be any arbitrary sequence.*

*Proof.* Let  $\mathbf{A} = (A_j, j \in \mathbb{Z}_+)$  be any arbitrary sequence. Suppose

$$\mathbf{U}(x) = \mathbf{U}(x') = \mathbf{A}$$

for all  $x, x' \in \{0, 1\}^m$ . In this case,

$$X_j = U_j(X_{j-1}) = A_j$$

for each  $j$  and  $\mathbf{X} = \mathbf{A}$ . □

**Example B.3.** Note that if the observed outcomes  $\mathbf{X}$  are independent and identically distributed, then it is not necessarily the case that there is no strong state dependence. For example, suppose that  $\mathbf{X}$  are independent and identically distributed Bernoulli with probability of success  $p$  and  $m = 1$ . Set  $U_j(X_{j-1}) = X_j$  and  $U_j(1 - X_{j-1}) = 1 - X_j$ . Then

$$\mathbb{P}(U_j(1) = 1) = \mathbb{P}(X_j = 1, X_{j-1} = 1) + \mathbb{P}(X_j = 0, X_{j-1} = 0) = p^2 + (1 - p)^2 \neq p$$

unless  $p = 1/2$ . So unless  $p = 1/2$ ,  $\mathbb{P}(U_j(1) = 1) \neq \mathbb{P}(X_j = 1)$ . Moreover, in this example, it is not the case that there is no weak state dependence either. ■

In the following theorem, we demonstrate that the equivalence between strong no state dependence and the independence and identical distribution of the observed outcome sequence  $\mathbf{X}$  is conditional on weak unconfoundedness (B.4). Moreover, independent and identical distributed  $\mathbf{X}$  and no strong state dependence imply weak unconfoundedness.

**Theorem B.2.** *If  $\mathbf{U}(x)$  is identically distributed for all  $x$ , in the sense that, for each  $x$ ,  $U_j(x)$  is identically distributed for all  $j$ , then any two of the conditions*

*(i) the observed outcomes  $\mathbf{X}$  are independent and identically distributed,*

(ii) there is strong no state dependence in the sense of (B.2), and  
 (iii) there is weak unconfoundedness in the sense of (B.4)  
 imply the third.

*Proof.* First, we show that (i) and (iii) imply (ii). Let  $X_{j:j'}$  denote  $(X_j, \dots, X_{j'})$  for  $j > j'$ . We have that,

$$\begin{aligned}\mathbb{P}(U_j(x) = x') &= \mathbb{P}(U_j(x) = x', X_{j-1:j-m} = x) + \mathbb{P}(U_j(x) = x', X_{j-1:j-m} \neq x) \\ &= \mathbb{P}(X_j = x', X_{j-1:j-m} = x) + \mathbb{P}(U_j(x) = x', X_{j-1:j-m} \neq x) \\ &= \mathbb{P}(X_j = x') \mathbb{P}(X_{j-1:j-m} = x) + \mathbb{P}(U_j(x) = x', X_{j-1:j-m} \neq x). \end{aligned}$$

(Independence of  $\mathbf{X}$ )

From (B.4), we have that the events  $\{U_j(x) = x'\}$  and  $\{X_{j-1:j-m} = x\}$  are independent, which implies that the events  $\{U_j(x) = 1 - x'\}$  and  $\{X_{j-1:j-m} \neq x\}$  are independent. As  $x'$  is arbitrary, we have that

$$\mathbb{P}(U_j(x) = x', X_{j-1:j-m} \neq x) = \mathbb{P}(U_j(x) = x') \mathbb{P}(X_{j-1:j-m} \neq x)$$

Thus, we can see that

$$\mathbb{P}(U_j(x) = x') = \mathbb{P}(X_j = x') \mathbb{P}(X_{j-1:j-m} = x) + \mathbb{P}(U_j(x) = x') \mathbb{P}(X_{j-1:j-m} \neq x)$$

giving

$$\mathbb{P}(U_j(x) = x') (1 - \mathbb{P}(X_{j-1:j-m} \neq x)) = \mathbb{P}(X_j = x') \mathbb{P}(X_{j-1:j-m} = x),$$

and  $\mathbb{P}(U_j(x) = x') = \mathbb{P}(X_j = x')$  for all  $x', x$ .

Next, we show that (ii) and (iii) imply (i). Take  $j > j' \in \mathbb{Z}^+$ . Then we have that, for  $z, z' \in \{0, 1\}$ ,

$$\begin{aligned}\mathbb{P}[X_j = z, X_{j'} = z'] &= \sum_{x \in \{0,1\}^m} \mathbb{P}(U_j(x) = z, X_{j-1:j-m} = x, X_{j'} = z') \\ &= \sum_{x \in \{0,1\}^m} \mathbb{P}(U_j(x) = z) \mathbb{P}(X_{j-1:j-m} = x, X_{j'} = z') \quad \text{(Weak Unconfoundedness)} \\ &= \sum_{x \in \{0,1\}^m} \mathbb{P}(X_j = z) \mathbb{P}(X_{j-1:j-m} = x, X_{j'} = z') \quad \text{(Strong No State Dependence)} \\ &= \mathbb{P}(X_j = z) \sum_{x \in \{0,1\}^m} \mathbb{P}(X_{j-1:j-m} = x, X_{j'} = z') \\ &= \mathbb{P}(X_j = z) \mathbb{P}(X_{j'} = z')\end{aligned}$$

Thus,  $\mathbf{X}$  is pairwise independent. Now suppose by induction, that  $X_{j_1}, \dots, X_{j_{l-1}}$  are independent for arbitrary  $j_1, \dots, j_{l-1}$ . The event  $\{X_{j_l} = z\}$  is independent from the event  $\{(X_{j_1}, \dots, X_{j_{l-1}}) = z'\}$

for  $z \in \{0, 1\}$  and  $z' \in \{0, 1\}^{l-1}$  by the argument in the preceding display replacing  $X_j$  with  $X_{j_l}$  and  $X_{j'}$  with  $(X_{j_1}, \dots, X_{j_{l-1}})$ . Thus  $\mathbf{X}$  is independent by induction.

If additionally  $\mathbf{U}(x)$  is identically distributed for all  $x$ , then note that

$$\begin{aligned} \mathbb{P}(X_j = z) &= \mathbb{P}(U_j(x) = z) && \text{(Strong No State Dependence)} \\ &= \mathbb{P}(U_{j'}(x) = z) && \text{(Identically Distributed)} \\ &= \mathbb{P}(X_{j'} = z) && \text{(Strong No State Dependence)} \end{aligned}$$

for all  $z \in \{0, 1\}$  and  $x \in \{0, 1\}^m$  and any  $j, j' > m$  and thus  $\mathbf{X}$  is independent and identically distributed.

Finally, we show that (i) and (ii) imply (iii). Observe that

$$\begin{aligned} \mathbb{P}(U_j(x) = x') \mathbb{P}(X_{j-1:j-m} = x) &= \mathbb{P}(X_j = x') \mathbb{P}(X_{j-1:j-m} = x) && \text{(Strong No State Dependence)} \\ &= \mathbb{P}(X_j = x', X_{j-1:j-m} = x) && \text{(Independence of } \mathbf{X} \text{)} \\ &= \mathbb{P}(U_j(x) = x', X_{j-1:j-m} = x). && \text{(Definition of } \mathbf{X} \text{)} \end{aligned}$$

□

**Corollary B.1.** *If  $\mathbf{U}(x)$  is identically distributed for all  $x$ , in the sense that, for each  $x$ ,  $U_j(x)$  is identically distributed for all  $j$ , and the unconfoundedness assumption (B.3) holds, then testing for randomness is equivalent to testing for strong no state dependence.*

*Proof.* The corollary follows from Theorem B.2 and the observation that unconfoundedness implies weak unconfoundedness. □

**Corollary B.2.** *Suppose that the potential outcome sequence  $\mathbf{U}$  is independent and identically distributed and independent of  $X_1$ . Then the restriction of strong no state dependence in the sense of (B.2) implies that  $\mathbf{X}$  is independent and identically distributed.*

*Proof.* By Theorem B.2, it suffices to show that there is weak unconfoundedness. We show this for the case  $m = 1$ . The argument holds for general  $m$ , but the notation is more involved. Observe that

$$\begin{aligned} &\mathbb{P}(U_j(x) = x', X_{j-1} = x) \\ &= \sum_{x \in \{0,1\}^{j-1}} \mathbb{P}(U_j(x) = x', U_{j-1}(x_1) = x, \dots, U_2(x_{j-2}) = x_{j-1}, X_1 = x_{j-1}) \\ &= \sum_{x \in \{0,1\}^{j-1}} \mathbb{P}(U_j(x) = x') \mathbb{P}(U_{j-1}(x_1) = x, \dots, U_2(x_{j-2}) = x_{j-1}, X_1 = x_{j-1}) \\ &\hspace{15em} \text{(Independence)} \\ &= \mathbb{P}(U_j(x) = x') \sum_{x \in \{0,1\}^{j-1}} \mathbb{P}(U_{j-1}(x_1) = x, \dots, U_2(x_{j-2}) = x_{j-1}, X_1 = x_{j-1}) \\ &\hspace{15em} \text{(Strong No State Dependence)} \end{aligned}$$

$$= \mathbb{P}(U_j(x) = x') \mathbb{P}(U_{j-1}(x_1) = x)$$

Thus, (B.4) holds.  $\square$

**Remark B.4.** Note that, when proving that strong no state dependence (B.2) and weak unconfoundedness (B.4) imply that the observed outcomes  $\mathbf{X}$  are independent and identically distributed, the conclusion that  $\mathbf{X}$  is identically distributed follows only from the conditions of strong no state dependence and  $\mathbf{U}(x)$  is identically distributed for all  $x \in \{0, 1\}^m$ .  $\blacksquare$

**Remark B.5.** When proving that strong no state dependence (B.2) and weak unconfoundedness (B.4) imply that the observed outcomes  $\mathbf{X}$  are independent and identically distributed, we can weaken the strong no state dependence assumption to a weak no state dependence assumption without loss.  $\blacksquare$

**Remark B.6.** In general, if there is strong no state dependence (B.2) and  $\mathbf{U}(x)$  is identically distributed for a given  $x$ , then  $\mathbf{U}(x)$  is identically distributed for all  $x$ . This follows from

$$\begin{aligned} \mathbb{P}(U_j(x') = z) &= \mathbb{P}(X_j = z) && \text{(Strong No State Dependence)} \\ &= \mathbb{P}(U_j(x) = z) && \text{(Strong No State Dependence)} \\ &= \mathbb{P}(U_{j'}(x) = z) && \text{(Identically Distributed)} \\ &= \mathbb{P}(X_{j'} = z) = \mathbb{P}(U_{j'}(x') = z) && \text{(Strong No State Dependence)} \end{aligned}$$

for all  $z \in \{0, 1\}$ ,  $x' \in \{0, 1\}^m$  and  $j, j' > m$ .  $\blacksquare$

## B.2 Stationarity and Dependence of Observed Outcomes

We show that if the potential outcome sequence is identically distributed and independent of past observed outcomes, then the observed outcome sequence is a homogeneous Markov chain of order  $m$ . Under conditions implying that the observed outcome sequence is stationary, aperiodic, and irreducible, the observed outcome sequence is  $\alpha$ -mixing.

**Theorem B.3.** Suppose that  $\mathbf{U}(x)$  is identically distributed for all  $x$ , in the sense that, for each  $x$ ,  $U_j(x)$  is identically distributed for all  $j$ , and unconfoundedness (B.3) holds, then  $\mathbf{X}$  is a homogeneous Markov chain of order  $m$ . Moreover, a joint distribution of  $X_1, \dots, X_m$  can be chosen such that  $\mathbf{X}$  is stationary. In this case, if

$$\mathbb{P}(U_j(x') = x) > 0 \text{ for } x \in \{0, 1\} \text{ and } x' \in \{0, 1\}^m \quad (\text{B.5})$$

then  $\mathbf{X}$  is  $\alpha$ -mixing.

*Proof.* Fix  $x \in \{0, 1\}$  and  $(x_1, \dots, x_k) \in (0, 1)^m$ . Let  $B_{j,k}$  be the event  $\{X_{j-1} = x_1, \dots, X_{j-k} = x_k\}$ . We want to show that

$$\mathbb{P}(X_j = x | B_{j,k}) = \mathbb{P}(X_j = x | B_{j,m}).$$

By Bayes rule, the left-hand side of the preceding display is

$$\mathbb{P}(U_j(x_1, \dots, x_m) = x | B_{j,k}) = \frac{\mathbb{P}(B_{j,k} | U_j(x_1, \dots, x_m) = x) \mathbb{P}(U_j(x_1, \dots, x_m) = x)}{\mathbb{P}(B_{j,k})}.$$

By unconfoundedness (B.3),  $\mathbb{P}(B_{j,k} | U_j(x_1, \dots, x_m) = x) = \mathbb{P}(B_{j,k})$ , so

$$\mathbb{P}(X_j = x | B_{j,k}) = \mathbb{P}(U_j(x_1, \dots, x_m) = x) = \mathbb{P}(X_j = x | B_{j,m}).$$

This shows that  $\mathbf{X}$  satisfies the Markov property of order  $m$ . The transition properties are time-invariant as the middle expression in the preceding expression do not depend on  $j$  by identical distribution of  $\mathbf{U}$ . Thus, the Markov chain is homogeneous.

By representing the  $m^{\text{th}}$  order Markov chain as an ordinary Markov chain in the usual way by enlarging the state space to  $2^m$  values, there always exists a stationary distribution in which to start the process. Thus,  $X_1, \dots, X_m$  can be chosen such that the resulting process is stationary as well.

Now, suppose that  $X_1, \dots, X_m$  is chosen such that the process is stationary. It is straightforward to see that  $\mathbf{X}$  is irreducible, as if  $X_{j-1:j-m} = x \in \{0, 1\}^m$  there is a positive probability that  $X_{j+m-1:j} = x'$  for all  $x' \in \{0, 1\}^m$  by (B.5). In addition,  $\mathbf{X}$  is clearly aperiodic as the state  $(1, 1, \dots, 1) \in \{0, 1\}^m$  can return to itself in one period with positive probability by (B.5). Hence,  $\mathbf{X}$  is  $\alpha$ -mixing by Theorem 3.1 of Bradley (2005).  $\square$

**Remark B.7.** The condition (B.5) is stronger than necessary for  $\mathbf{X}$  to be  $\alpha$ -mixing. In fact, it is sufficient for  $\mathbf{X}$  to be aperiodic and irreducible.  $\blacksquare$

### B.3 Markov Chain Streaky Alternatives

Our Markov chain Streaky alternatives, specified in Section 4.1, can be written

$$U_j(x) \stackrel{d}{\sim} \text{Bernoulli}(p_x)$$

where

$$p_x = \begin{cases} 1/2 + \epsilon & x = \mathbf{1}_m, \\ 1/2 - \epsilon & x = \mathbf{0}_m, \\ 1/2 & \text{otherwise,} \end{cases}$$

where  $\mathbf{1}_m$  and  $\mathbf{0}_m$  are vectors of 1's and 0's of length  $m$ , respectively and  $U_j(x)$  are i.i.d for all  $x$  and  $j$ . Under this model, we have that

$$SD(x, x') = \begin{cases} 2\epsilon & x = \mathbf{1}_m, x' = \mathbf{0}_m, \\ -2\epsilon & x = \mathbf{0}_m, x' = \mathbf{1}_m, \\ \epsilon & x = \mathbf{1}_m, x' \notin \{\mathbf{1}_m, \mathbf{0}_m\}, \\ -\epsilon & x = \mathbf{0}_m, x' \notin \{\mathbf{1}_m, \mathbf{0}_m\}, \\ 0 & \text{otherwise,} \end{cases} \quad \text{and} \quad SD(x) = \begin{cases} \epsilon & x = \mathbf{1}_m, \\ -\epsilon & x = \mathbf{0}_m, \\ 0 & \text{otherwise.} \end{cases}$$

The test statistics  $\hat{D}_{n,k}(\mathbf{X}_i)$  and  $\hat{P}_{n,k}(\mathbf{X}_i) - \hat{p}_{i,n}$  can be thought of as natural statistics for testing the hypotheses

$$\begin{aligned} SD(\mathbf{1}_m, \mathbf{0}_m) &= 0 \text{ and} \\ SD(\mathbf{1}_m) &= 0 \end{aligned}$$

for  $k = m$ , respectively.

## C Asymptotic Distributions of $\bar{P}_k(\mathbf{X})$ and $\bar{D}_k(\mathbf{X})$

In this section, we study the asymptotic behavior the statistics  $\bar{P}_k(\mathbf{X})$  and  $\bar{D}_k(\mathbf{X})$ . First, note that by Theorem 3.1, for  $s$  individuals, with the  $i^{\text{th}}$  individual having success rate  $p_i$ , under  $H_0$ ,

$$\sqrt{ns}\bar{D}_k(\mathbf{X}) \xrightarrow{d} N\left(0, \frac{1}{s} \sum_{i=1}^s \sigma_D^2(p_i, k)\right). \quad (\text{C.1})$$

Next, consider the case where  $p_i$  are outcomes of a random variable  $S_i$ , where the  $S_i$  are i.i.d. according to  $\Lambda$ . If  $s \rightarrow \infty$  and  $\sigma_D^2(\Lambda, k)$  defined by

$$\sigma_D^2(\Lambda, k) \equiv \int_0^1 \sigma_D^2(p, k) d\Lambda(p)$$

satisfies  $\sigma_D^2(\Lambda, k) < \infty$ , then by the law of large numbers

$$\frac{1}{s} \sum_{i=1}^s \sigma_D^2(p_i, k) \rightarrow \sigma_D^2(\Lambda, k)$$

with probability one.

Furthermore, if  $s \rightarrow \infty$  and  $n \rightarrow \infty$ , we can conclude that under  $H_0$ ,

$$\sqrt{ns}\bar{D}_k(\mathbf{X}) \xrightarrow{d} N(0, \sigma_D^2(\Lambda, k)). \quad (\text{C.2})$$

First, consider one individual. Theorem 3.1 covers the limiting behavior conditional on  $S_i = p_i$ . So, under  $H_0$ ,

$$\mathbb{P}_i \left\{ \sqrt{n}\hat{D}_{n,k}(\mathbf{X}_i) \leq t \right\} = \int_0^1 \mathbb{P}_i \left\{ \sqrt{n}\hat{D}_{n,k}(\mathbf{X}_i) \leq t | S_i = p \right\} d\Lambda(p) \rightarrow \int \Phi(t/\sigma_D^2(p, k)) d\Lambda(p)$$

by dominated convergence. This limiting distribution, which is not normal unless  $\Lambda$  is degenerate, can be represented by a random variable  $B_i$  such that  $B_i | S_i = p$  is  $N(0, \sigma_D^2(p, k))$  and  $S_i \stackrel{d}{\sim} \Lambda$ .

Now, for  $s$  individuals with “random”  $p_i$ , conditional on  $S_1, \dots, S_s$ ,

$$\sqrt{ns}\bar{D}_k(\mathbf{X}) \xrightarrow{d} N\left(0, \frac{1}{s} \sum_{i=1}^s \sigma_D^2(p_i, k)\right).$$

But unconditionally, we can say for finite  $s$  that

$$\sqrt{ns}\bar{D}_k(\mathbf{X}) \xrightarrow{d} \frac{1}{\sqrt{s}} \sum_{i=1}^s B_i,$$

where the  $B_i$  are i.i.d. according to the Gaussian mixture as previously specified. Thus, if  $s \rightarrow \infty$ , then

$$\frac{1}{\sqrt{s}} \sum_{i=1}^s B_i \xrightarrow{d} N(0, \sigma_D^2(\Lambda, k)).$$

Now, as in the context of Section 3.3, assume that for each  $i$  in  $1, \dots, s$ ,  $\mathbf{X}_i = \{X_{ij}\}_{j=1}^\infty$  is a possibly dependent Bernoulli( $p_i$ ) sequence, where  $\hat{a}_{n,i}$  denotes the number of ones in the first  $n$  elements of  $\mathbf{X}_i$  and  $n^{-1/2}(\hat{a}_n - np_i)$  converges in distribution to some limiting distribution. Then, the stratified permutation distributions for  $\sqrt{ns}K_{n,s}$  based on the test statistics  $\bar{D}_k(\mathbf{X})$  satisfies

$$\sup_t \left| K_{n,s}(t) - \Phi\left(t / \sqrt{\frac{1}{s} \sum_{i=1}^s \sigma_D^2(p_i, k)}\right) \right| \xrightarrow{P} 0 \quad (\text{C.3})$$

as  $n \rightarrow \infty$ . An analogous result is obtained if the test statistic is chosen as  $\bar{P}_k(\mathbf{X})$ .

Interestingly, with  $s$  fixed and  $p_i$  random, the permutation distribution will not behave like the limiting distribution (C.2). It will behave as (C.1), so it is actually random in the limit (even for  $s = 1$ ) in that it depends on the outcome  $S_i = p_i$ . More formally, the stratified permutation distributions for  $\sqrt{ns}K_{n,s}$  based on the test statistics  $\bar{D}_k(\mathbf{X})$  satisfies (C.3). This is intuitive, because even for  $s = 1$ , the observed outcome sequence will behave like a random sequence from  $p_i$  and the permutation distribution can’t possibly know that some other value of  $p_i$  could have been drawn. So, technically, the permutation distribution does not behave like its unconditional distribution, even under  $H_0$ . But this is not a problem, as

$$\mathbb{P}\{\text{Permutation test rejects } H_0^i\} = \int \mathbb{P}\{\text{Permutation test rejects } H_0^i | S_i = p\} d\Lambda(p),$$

and the integrand is equal to  $\alpha$  for each  $p$ , and so the overall level is still  $\alpha$ .

## D Second Order Approximations

In this section, we give second order approximations to moments of the plug-in statistics studied in Section 2. First, let  $\hat{Q}_{n,k}(\mathbf{X}_i)$  denote the proportion of zeros following  $k$  consecutive zeros.

Recalling that,  $Z_{ijk} = \prod_{l=j}^{j+k} (1 - X_{il})$  and  $W_{ik} = \sum_{j=1}^{n-k} Z_{ijk}$ , then  $\hat{Q}_{n,k}(\mathbf{X}_i)$  is given by

$$\hat{Q}_{n,k}(\mathbf{X}_i) = W_{ik} / W_{i(k-1)}. \quad (\text{D.1})$$

**Theorem D.1.** *Under the assumption that  $\mathbf{X}_i = \{X_{ij}\}_{j=1}^n$  is a sequence of independent and identically distributed Bernoulli( $p_i$ ) random variables, then*

(i) *the expectation of  $\hat{P}_k(\mathbf{X}_i)$  has a second order approximation given by*

$$\mathbb{E} [\hat{P}_{n,k}(\mathbf{X}_i)] = p_i + n^{-1} p_i (1 - p_i^{-k}) + O(n^{-2}). \quad (\text{D.2})$$

(ii) *the expectation of  $\hat{D}_k(\mathbf{X}_i)$  has a second order approximation given by*

$$\mathbb{E} [\hat{D}_{n,k}(\mathbf{X}_i)] = n^{-1} (1 - (1 - p_i)^{1-k} - p_i^{1-k}) + O(n^{-2}). \quad (\text{D.3})$$

(iii) *Cov  $(\hat{P}_{n,k}(\mathbf{X}_i), \hat{Q}_{n,k}(\mathbf{X}_i))$  has a second order approximation given by*

$$\text{Cov} (\hat{P}_k(\mathbf{X}_i), \hat{Q}_k(\mathbf{X}_i)) = O(n^{-2}). \quad (\text{D.4})$$

*Proof.* We consider the case with  $s = 1$ , and therefore drop the dependence on the individual  $i$ . For notational simplicity, let  $\bar{V}_{n,k} = n^{-1} \sum_{j=1}^{n-k} Y_{jk}$  with  $Y_{jk} = \prod_{l=j}^{j+k} X_l$  and  $\bar{W}_{n,k} = n^{-1} \sum_{j=1}^{n-k} Z_{jk}$  with  $Z_{jk} = \prod_{l=j}^{j+k} (1 - X_l)$ .

Let  $g(\theta_1, \theta_2) = \theta_1 / \theta_2$ . The Taylor expansion of  $\mathbb{E} [\hat{P}_{n,k}(\mathbf{X})] = \mathbb{E} [g(\bar{V}_{n,k}, \bar{V}_{n,k-1})]$  about  $(p^{k+1}, p^k)$  is given by

$$\begin{aligned} \mathbb{E} [\hat{P}_{n,k}(\mathbf{X})] &= g(p^{k+1}, p^k) + \frac{1}{2} \text{Var}(\bar{V}_{n,k}) \frac{\partial^2 g}{\partial \bar{V}_k^2}(p^{k+1}, p^k) \\ &\quad + \frac{1}{2} \text{Var}(\bar{V}_{n,k-1}) \frac{\partial^2 g}{\partial \bar{V}_{n,k-1}^2}(p^{k+1}, p^k) + \text{Cov}(\bar{V}_{n,k}, \bar{V}_{n,k-1}) \frac{\partial^2 g}{\partial \bar{V}_{n,k} \partial \bar{V}_{n,k-1}}(p^{k+1}, p^k) + O(n^{-2}). \\ &= p + p^{1-2k} \text{Var}(\bar{V}_{n,k-1}) - \frac{1}{p^{2k}} \text{Cov}(\bar{V}_{n,k}, \bar{V}_{n,k-1}) + O(n^{-2}). \end{aligned}$$

This is given by

$$\begin{aligned} \mathbb{E} [\hat{P}_{n,k}(\mathbf{X})] &= p + \frac{p^{1-2k}}{n} \left( p^k - (2k-1)p^{2k} + \frac{2p^{k+1} - 2p^{2k}}{1-p} \right) + \\ &\quad - \frac{1}{np^{2k}} \left( 2p^{k+1} - 2kp^{2k+1} + \frac{2p^{k+2} - 2p^{2k+1}}{1-p} \right) + O(n^{-2}) \\ &= p + n^{-1} p (1 - p^{-k}) + O(n^{-2}). \end{aligned}$$

Similarly, to show (ii), we can see that

$$\mathbb{E} [\hat{D}_{n,k}(\mathbf{X})] = \mathbb{E} [\hat{P}_{n,k}(\mathbf{X})] - (1 - \mathbb{E} [\hat{Q}_{n,k}(\mathbf{X})])$$

$$\begin{aligned}
&= p + n^{-1}p(1 - p^{-k}) - \left(1 - (1 - p) - n^{-1}(1 - p)\left(1 - (1 - p)^{-k}\right)\right) + O(n^{-2}) \\
&= n^{-1}\left(1 - (1 - p)^{1-k} - p^{1-k}\right) + O(n^{-2}).
\end{aligned}$$

Finally, we show (iii). Let  $g(\theta_1, \theta_2, \theta_3, \theta_4) = \theta_1\theta_3/\theta_2\theta_4$ . The Taylor expansion of  $\mathbb{E}[\hat{P}_{n,k}(\mathbf{X})\hat{Q}_{n,k}(\mathbf{X})] = \mathbb{E}[g(\bar{V}_{n,k}, \bar{V}_{n,k-1}, \bar{W}_{n,k}, \bar{W}_{n,k-1})]$  about  $\rho = (p^{k+1}, p^k, (1-p)^{k+1}, (1-p)^k)$  is given by

$$\begin{aligned}
&\mathbb{E}[\hat{P}_{n,k}(\mathbf{X})\hat{Q}_{n,k}(\mathbf{X})] \\
&= g(\rho) \\
&+ \frac{1}{2} \text{Var}(\bar{V}_{n,k}) \frac{\partial^2 g}{\partial \bar{W}_{n,k}^2}(\rho) + \frac{1}{2} \text{Var}(\bar{V}_{n,k-1}) \frac{\partial^2 g}{\partial \bar{W}_{n,k-1}^2}(\rho) \\
&+ \frac{1}{2} \text{Var}(\bar{W}_{n,k}) \frac{\partial^2 g}{\partial \bar{V}_{n,k}^2}(\rho) + \frac{1}{2} \text{Var}(\bar{W}_{n,k-1}) \frac{\partial^2 g}{\partial \bar{V}_{n,k-1}^2}(\rho) \\
&+ \text{Cov}(\bar{V}_{n,k}, \bar{V}_{n,k-1}) \frac{\partial^2 g}{\partial \bar{V}_{n,k} \partial \bar{V}_{n,k-1}}(\rho) + \text{Cov}(\bar{V}_{n,k}, \bar{W}_{n,k}) \frac{\partial^2 g}{\partial \bar{V}_{n,k} \partial \bar{W}_{n,k}}(\rho) \\
&+ \text{Cov}(\bar{V}_{n,k}, \bar{W}_{n,k-1}) \frac{\partial^2 g}{\partial \bar{V}_{n,k} \partial \bar{W}_{n,k-1}}(\rho) + \text{Cov}(\bar{V}_{n,k-1}, \bar{W}_{n,k}) \frac{\partial^2 g}{\partial \bar{V}_{n,k-1} \partial \bar{W}_{n,k}}(\rho) \\
&(\rho) + \text{Cov}(\bar{V}_{n,k-1}, \bar{W}_{n,k-1}) \frac{\partial^2 g}{\partial \bar{V}_{n,k-1} \partial \bar{W}_{n,k-1}}(\rho) + \text{Cov}(\bar{W}_{n,k}, \bar{W}_{n,k-1}) \frac{\partial^2 g}{\partial \bar{W}_{n,k} \partial \bar{W}_{n,k-1}}(\rho) + O(n^{-2}) \\
&= p(1-p) + p^{1-2k}(1-p) \text{Var}(\bar{V}_{n,k-1}) + p(1-p)^{1-2k} \text{Var}(\bar{W}_{n,k-1}) \\
&- \frac{(1-p)}{p^{2k}} \text{Cov}(\bar{V}_{n,k}, \bar{V}_{n,k-1}) + \frac{1}{p^k(1-p)^k} \text{Cov}(\bar{V}_{n,k}, \bar{W}_{n,k}) - \frac{(1-p)^{1-k}}{p^k} \text{Cov}(\bar{V}_{n,k}, \bar{W}_{n,k-1}) \\
&- \frac{p^{1-k}}{(1-p)^k} \text{Cov}(\bar{V}_{n,k-1}, \bar{W}_{n,k}) + p^{1-k}(1-p)^{1-k} \text{Cov}(\bar{V}_{n,k-1}, \bar{W}_{n,k-1}) \\
&- \frac{p}{(1-p)^{2k}} \text{Cov}(\bar{W}_{n,k}, \bar{W}_{n,k-1}) + O(n^{-2}),
\end{aligned}$$

which can be expressed

$$\begin{aligned}
&\mathbb{E}[\hat{P}_{n,k}(\mathbf{X})\hat{Q}_{n,k}(\mathbf{X})] \\
&= p(1-p) + \frac{p^{1-2k}(1-p)}{n} \left( p^k - (2k-1)p^{2k} + \frac{2p^{k+1} - 2p^{2k}}{1-p} \right) \\
&+ \frac{p(1-p)^{1-2k}}{n} \left( (1-p)^k - (2k-1)(1-p)^{2k} + \frac{2(1-p)^{k+1} - 2(1-p)^{2k}}{p} \right) \\
&- \frac{(1-p)}{np^{2k}} \left( 2p^{k+1} - 2kp^{2k+1} + \frac{2p^{k+2} - 2p^{2k+1}}{1-p} \right) \\
&+ \frac{1}{np^k(1-p)^k} \left( -(2k+1)p^{k+1}(1-p)^{k+1} \right) - \frac{(1-p)^{1-k}}{np^k} \left( -(2k)p^{k+1}(1-p)^k \right) \\
&- \frac{p^{1-k}}{n(1-p)^k} \left( -(2k)p^k(1-p)^{k+1} \right) + \frac{p^{1-k}(1-p)^{1-k}}{n} \left( -(2k-1)p^k(1-p)^k \right)
\end{aligned}$$

$$\begin{aligned}
& - \frac{p}{n(1-p)^{2k}} \left( 2(1-p)^{k+1} - 2k(1-p)^{2k+1} + \frac{2(1-p)^{k+2} - 2(1-p)^{2k+1}}{p} \right) + O(n^{-2}) \\
& = p(1-p) - n^{-1}(1-p)^{1-k} p^{1-k} \left( p^k + (1-p)^k (1-2p^k) \right) + O(n^{-2}).
\end{aligned}$$

Therefore, we can see that

$$\begin{aligned}
& \text{Cov} \left( \hat{P}_{n,k}(\mathbf{X}), \hat{Q}_{n,k}(\mathbf{X}) \right) \\
& = \mathbb{E} \left[ \hat{P}_{n,k}(\mathbf{X}) \hat{Q}_{n,k}(\mathbf{X}) \right] - \mathbb{E} \left[ \hat{P}_{n,k}(\mathbf{X}) \right] \mathbb{E} \left[ \hat{Q}_{n,k}(\mathbf{X}) \right] \\
& = p(1-p) - n^{-1} \left( (1-p)^{1-k} p^{1-k} \left( p^k + (1-p)^k (1-2p^k) \right) \right) + O(n^{-2}) \\
& - p(1-p) - n^{-1} \left( p(1-p) \left( 2 - p^{-k} - (1-p)^{-k} \right) \right) \\
& + n^{-2} \left( p(1-p) (1-p^{-k}) \left( 1 - (1-p)^{-k} \right) \right) \\
& = n^{-2} \left( p(1-p) (1-p^{-k}) \left( 1 - (1-p)^{-k} \right) \right) + O(n^{-2}).
\end{aligned}$$

□

**Remark D.1.** Note that the asymptotic variance of  $\hat{D}_{n,k}(\mathbf{X}_i)$  is equal to the sum of the asymptotic variances of  $\hat{P}_{n,k}(\mathbf{X}_i)$  and  $\hat{Q}_{n,k}(\mathbf{X}_i)$ , suggesting that

$$n \text{Cov} \left( \hat{P}_{n,k}(\mathbf{X}_i), \hat{Q}_{n,k}(\mathbf{X}_i) \right) \rightarrow 0. \quad (\text{D.5})$$

In fact, we show that  $\text{Cov} \left( \hat{P}_{n,k}(\mathbf{X}_i), \hat{Q}_{n,k}(\mathbf{X}_i) \right) = O(n^{-2})$ . GVT and MS approximate the variance of  $\hat{D}_{n,k}(\mathbf{X}_i)$  with estimators that implicitly assume (D.5). MS cite a simulation exercise supporting their assumption. Our results justify this assumption mathematically. Additionally, the asymptotic variance of  $\hat{P}_{n,k}(\mathbf{X}_i) - p_i$  is equal to the sum of the asymptotic variance of  $\hat{P}_{n,k}(\mathbf{X}_i) - \hat{p}_{n,i}$  and  $p_i(1-p_i)$ , which implies  $\hat{P}_{n,k}(\mathbf{X}_i) - \hat{p}_{n,i}$  and  $\hat{p}_{n,i}$  are asymptotically independent. ■

**Remark D.2.** Using similar arguments, it can be shown that the parametric bootstrap bias-corrected statistics

$$\hat{P}_{n,k}(\mathbf{X}_i) - \hat{p}_{n,i} - \beta_P^{n,k}(\hat{p}_{n,i}) \text{ and } \hat{D}_{n,k}(\mathbf{X}_i) - \beta_D^{n,k}(\hat{p}_{n,i}),$$

have bias of order  $1/n^2$  when considered as estimators of  $\theta_P^k(\mathbb{P}_i)$  and  $\theta_D^k(\mathbb{P}_i)$  under the null hypothesis  $H_0^i$ , as opposed to a bias of order  $1/n$  for the statistics  $\hat{P}_{n,k}(\mathbf{X}_i) - \hat{p}_{n,i}$  and  $\hat{D}_{n,k}(\mathbf{X}_i)$ .

Online Appendix Figure 5 displays the second order approximation to the expectations of  $\hat{P}_{n,k}(\mathbf{X}_i)$  and  $\hat{D}_{n,k}(\mathbf{X}_i)$  under  $H_0^i$  for  $k = 1$  and 3 and  $p_i \in (0.25, 0.5, 0.75)$ . The approximation is not suitable for small values of  $p_i$  and  $n$  for large  $k$ , but does a remarkably good job for moderate values of  $p_i$  and  $n$ . Note that the second order approximation for  $\mathbb{E} \left[ \hat{D}_{n,k}(\mathbf{X}_i) \right]$  when  $k = 1$  is the same for all  $p_i$ , and in fact, the Monte Carlo estimates for the finite-sample values of  $\mathbb{E} \left[ \hat{D}_{n,k}(\mathbf{X}_i) \right]$  when  $k = 1$  are too close to discern at the scale that we have plotted them.

Online Appendix Figure 5: Second Order Approximation

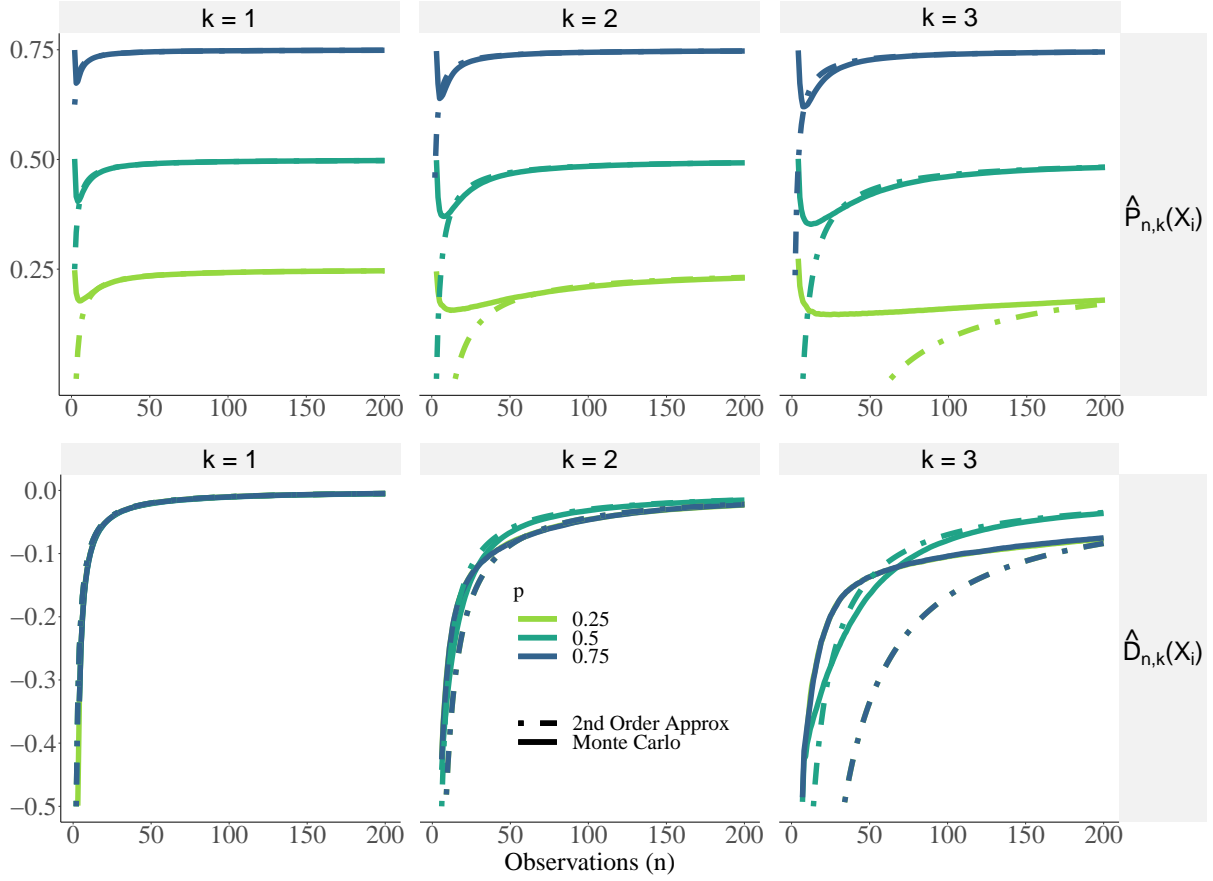

Notes: The figure displays the the second order approximations to the expectations of  $\hat{P}_{n,k}(\mathbf{X}_i)$  and  $\hat{D}_{n,k}(\mathbf{X}_i)$  under  $H_0^i$  for  $k = 1, 2$  and  $3$  and  $p \in (0.25, 0.5, 0.75)$ . In all panels, the solid lines give the Monte Carlo approximations and the dot-dashed lines give the second order approximation.

## E Variance Estimation

In this section we consider variance estimation under the null hypothesis. Any consistent estimate of  $p_i$  can be plugged into the asymptotic variances of  $\hat{P}_{n,k}(\mathbf{X}_i) - \hat{p}_{n,i}$  and  $\hat{D}_{n,k}(\mathbf{X}_i)$  to produce a set of consistent estimators. This includes  $\hat{P}_{n,k}(\mathbf{X}_i)$  for all  $k$ . Additionally, the variances can be estimated consistently with the permutation distribution or with the bootstrap. We show that  $\hat{P}_{n,k}(\mathbf{X}_i) \left(1 - \hat{P}_{n,k}(\mathbf{X}_i)\right) / V_{ik}$ , with  $V_{ik} = \sum_{j=1}^{n-k} Y_{ijk}$  for  $Y_{ijk} = \prod_{l=j}^{j+k} X_{il}$ , is also a consistent estimator for the asymptotic variance of  $\hat{P}_{n,k}(\mathbf{X}_i)$ . MS estimate the variance of  $\hat{D}_{n,k}(\mathbf{X}_i)$  with

$$\left( \frac{(V_{ik} - 1) s_{p,i}^2 + (W_{ik} - 1) s_{q,i}^2}{V_{ik} + W_{ik} - 2} \right) \left( \frac{1}{V_{ik}} + \frac{1}{W_{ik}} \right) \quad (\text{E.1})$$

where  $s_{p,i}^2 = \left(\frac{V_{ik}}{V_{ik}-1}\right) \hat{P}_{n,k}(\mathbf{X}_i) \left(1 - \hat{P}_{n,k}(\mathbf{X}_i)\right)$  and  $s_{q,i}^2 = \left(\frac{W_{ik}}{W_{ik}-1}\right) \hat{Q}_{n,k}(\mathbf{X}_i) \left(1 - \hat{Q}_{n,k}(\mathbf{X}_i)\right)$ , and  $\hat{Q}_{n,k}(\mathbf{X}_i) = W_{ik}/W_{i(k-1)}$  with  $Z_{ijk} = \prod_{l=j}^{j+k} (1 - X_{il})$  and  $W_{ik} = \sum_{j=1}^{n-k} Z_{ijk}$ . This estimator is typically employed when  $\hat{P}_{n,k}(\mathbf{X}_i)$  and  $\hat{Q}_{n,k}(\mathbf{X}_i)$  are the sample means of i.i.d. populations assumed to have equal variances. This is not the case in our setting, where the variances of  $\hat{P}_{n,k}(\mathbf{X}_i)$  and  $\hat{Q}_{n,k}(\mathbf{X}_i)$  are not equal and the covariance of  $\hat{P}_{n,k}(\mathbf{X}_i)$  and  $\hat{Q}_{n,k}(\mathbf{X}_i)$  is not equal to 0. We show that the ratio of (E.1) and the asymptotic variance of  $\hat{D}_{n,k}(\mathbf{X}_i)$  converges to 1 in probability.

**Theorem E.1.** *Under the assumption that  $\mathbf{X}_i = \{X_{ij}\}_{j=1}^n$  is a sequence of independent and identically distributed Bernoulli( $p$ ) random variables, then the ratio*

$$\frac{s_{p,i}^2/V_{ik}}{n^{-1} \hat{P}_{n,k}(\mathbf{X}_i)^{1-k} \left(1 - \hat{P}_{n,k}(\mathbf{X}_i)\right)}$$

tends to 1 in probability.

*Proof.* We consider the case with  $s = 1$ , and therefore drop the dependence on the individual  $i$ . Since by Theorem 3.1,  $\hat{P}_{n,k}(\mathbf{X})$  is a consistent estimator of  $p$ , it follows that

$$\frac{\hat{P}_{n,k}(\mathbf{X})^{1-k} \left(1 - \hat{P}_{n,k}(\mathbf{X})\right) / n}{p^{1-k} (1 - p) / n} \xrightarrow{P} 1.$$

So, in order to show

$$\frac{\hat{P}_{n,k}(\mathbf{X}) \left(1 - \hat{P}_{n,k}(\mathbf{X})\right) / V_k}{\hat{P}_{n,k}(\mathbf{X})^{1-k} \left(1 - \hat{P}_{n,k}(\mathbf{X})\right) / n} \xrightarrow{P} 1$$

it suffices to show that

$$\frac{\hat{P}_{n,k}(\mathbf{X}) \left(1 - \hat{P}_{n,k}(\mathbf{X})\right) / V_k}{p (1 - p) / np^k} \xrightarrow{P} 1.$$

This is equivalent to

$$\frac{np^k}{V_k} \xrightarrow{P} 1$$

and in turn to

$$\frac{V_k}{np^k} \xrightarrow{P} 1.$$

This follow from

$$\frac{\mathbb{E}[V_k]}{np^k} = \frac{(n-k)p^k}{np^k} \rightarrow 1$$

and

$$\text{Var}\left(\frac{V_k}{np^k}\right) = \frac{1}{n^2 p^{2k}} \text{Var}(V_k) = O(n^{-1}) \rightarrow 0$$

as  $\text{Var}(W_k)$  is given by

$$n \left( p^k - (2k-1)p^{2k} + \frac{2p^{k+1} - 2p^{2k}}{1-p} \right).$$

□

**Theorem E.2.** *Let  $\mathbf{X}_i = \{X_{ij}\}_{j=1}^n$  be a sequence of independent and identically distributed Bernoulli( $p_i$ ) random variables. Then, the ratio of*

$$\left( \frac{(V_{ik}-1)s_{p,i}^2 + (W_{ik}-1)s_{q,i}^2}{V_{ik} + W_{ik} - 2} \right) \left( \frac{1}{V_{ik}} + \frac{1}{W_{ik}} \right) \quad (\text{E.2})$$

and the asymptotic variance of  $\hat{D}_{n,k}(\mathbf{X}_i)$ , given by (6), tends to 1 in probability.

*Proof.* We consider the case with  $s = 1$ , and therefore drop the dependence on the individual  $i$ . By the proof of Theorem E.1, the ratio of

$$\left( \frac{(V_{ik}-1)s_{p,i}^2 + (W_{ik}-1)s_{q,i}^2}{V_{ik} + W_{ik} - 2} \right) \left( \frac{1}{V_{ik}} + \frac{1}{W_{ik}} \right)$$

and

$$\begin{aligned} & \left( \frac{np^{k+1}(1-p) + n(1-p)^{k+1}p}{np^k + n(1-p)^k} \right) \left( \frac{1}{np^k} + \frac{1}{n(1-p)^k} \right) \\ &= \frac{p(1-p)((1-p)^k + p^k)}{np^k(1-p)^k} \\ &= n^{-1}(p(1-p))^{1-k}((1-p)^k + p^k) \end{aligned}$$

tends to 1 in probability as  $n$  grows to infinity.

□

## F A General Convergence Theorem Under $\alpha$ -Mixing

Define the measure of dependence

$$\alpha(\mathcal{A}, \mathcal{B}) = \sup \{ |\mathbb{P}(A \cap B) - \mathbb{P}(A)\mathbb{P}(B)| : A \in \mathcal{A}, B \in \mathcal{B} \}, \quad (\text{F.1})$$

where  $\mathcal{A}$  and  $\mathcal{B}$  are two sub  $\sigma$ -fields of the  $\sigma$ -field  $\mathcal{F}$ . For  $\mathbf{X}_i = (X_{ij}, j \in \mathbb{Z}_+)$ , a sequence of random variables, let us define the mixing coefficient

$$\alpha(\mathbf{X}_i, n) = \sup_{j \in \mathbb{Z}} \alpha(\mathcal{F}_{-\infty}^j(\mathbf{X}_i), \mathcal{F}_{j+n}^\infty(\mathbf{X}_i)), \quad (\text{F.2})$$

where the  $\sigma$ -field  $\mathcal{F}_j^K(\mathbf{X}_i)$  is given by  $\sigma(X_{ij}, j \leq j \leq K)$ , with  $\sigma(\dots)$  denoting the  $\sigma$ -field generated by  $(\dots)$ . We say  $\mathbf{X}_i$  is  $\alpha$ -mixing if  $\alpha(\mathbf{X}_i, n) \rightarrow 0$  as  $n \rightarrow \infty$ . Additionally, for  $\mathbf{G} = (G_j, j \in \mathbb{Z}_+)$ , a stationary sequence of random vectors, let

$$\Sigma(\mathbf{G}) = \text{Var}(G_1) + 2 \sum_{i=2}^{\infty} \text{Cov}(G_1, G_i). \quad (\text{F.3})$$

By appealing to Theorem 1.7 of Ibragimov (1962), we can give a general form for the asymptotic distributions of the test statistics under  $\alpha$ -mixing processes.

**Theorem F.1.** *Assuming  $\mathbf{X}_i = (X_{ij}, j \in \mathbb{Z}_+)$  is a stationary,  $\alpha$ -mixing, Bernoulli sequence such that  $\sum_{j=1}^{\infty} \alpha(\mathbf{X}_i, j) < \infty$ , with  $\alpha(\mathbf{X}_i, j)$  given by (F.2), then*

(i)  $\hat{P}_{n,k}(\mathbf{X}_i) - \hat{p}_{n,i}$ , given by (2.4), is asymptotically normal with limiting distribution given by

$$\sqrt{n} \left( \left( \hat{P}_{n,k}(\mathbf{X}_i) - \hat{p}_{n,i} \right) - \left( \frac{\mathbb{E}[Y_{ijk}]}{\mathbb{E}[Y_{ij(k-1)}]} - p_i \right) \right) \xrightarrow{d} N \left( 0, \mathbb{E}[\Gamma_{ij}]^\top \Sigma(\Gamma_{ij}) \mathbb{E}[\Gamma_{ij}] \right), \quad (\text{F.4})$$

where  $\Gamma_{ij} = [Y_{ijk}, Y_{ij(k-1)}, X_j]^\top$  and  $\Sigma(\Gamma_{ij})$  is given by (F.3), and

(ii)  $\hat{D}_{n,k}(\mathbf{X}_i)$ , given by (2.4), is asymptotically normal with limiting distribution given by

$$\sqrt{n} \left( \hat{D}_{n,k}(\mathbf{X}_i) - \left( \frac{\mathbb{E}[Y_{ijk}]}{\mathbb{E}[Y_{ij(k-1)}]} - \left( 1 - \frac{\mathbb{E}[Z_{ijk}]}{\mathbb{E}[Z_{ij(k-1)}]} \right) \right) \right) \xrightarrow{d} N \left( 0, \mathbb{E}[\Lambda_{ij}]^\top \Sigma(\Lambda_{ij}) \mathbb{E}[\Lambda_{ij}] \right), \quad (\text{F.5})$$

where  $\Lambda_{ij} = [Y_{ijk}, Y_{ij(k-1)}, Z_{ijk}, Z_{ij(k-1)}]^\top$  and  $\Sigma(\Lambda_{ij})$  is given by (F.3).

*Proof.* We consider the case with  $s = 1$ , and therefore drop the dependence on the individual  $i$ . As before, let  $\mathbf{Y}_k = (Y_{jk} = \prod_{m=j}^{j+k} X_m, j \in \mathbb{Z}_+)$  and  $\mathbf{Z}_k = (Z_{jk} = \prod_{m=j}^{j+k} (1 - X_m), j \in \mathbb{Z}_+)$ . The  $\mathbf{Y}_k$  and  $\mathbf{Z}_k$  processes are also  $\alpha$ -mixing since they are  $k+1$ -dependent. For example,  $\alpha(\mathbf{Y}_j, n) \leq \alpha(\mathbf{X}_j, n-k)$  if  $n-k > 0$ , and similarly for  $\mathbf{Z}_k$ . This also implies that the mixing coefficients for  $\mathbf{Y}_k$  and  $\mathbf{Z}_k$  are summable, and similarly for  $\Gamma_j$  and  $\Lambda_j$ .

Next, we evaluate the asymptotic normal limiting distribution of  $\hat{P}_{n,k}(\mathbf{X}) - \hat{p}_n$ . Recall that  $\Gamma_j = [Y_{jk}, Y_{j(k-1)}, X_j]^\top$ . By Theorem 1.7 of Ibragimov (1962) and the Cramér-Wold device, as  $\mathbf{Y}_k$  is strictly stationary with finite absolute moments and summable mixing coefficients,

$$n^{-1/2} \sum_{j=1}^n [\Gamma_j - \mathbb{E}[\Gamma_j]] \xrightarrow{d} N(0, \Sigma(\Gamma_j))$$

and each component of  $\Sigma(\Gamma_j)$  is non-zero and finite. Therefore, by the Delta Method,

$$n^{1/2} \left( \hat{P}_{n,k}(\mathbf{X}) - \hat{p}_n - \frac{\mathbb{E}[Y_{jk}]}{\mathbb{E}[Y_{j(k-1)}]} - p \right) \xrightarrow{d} N \left( 0, \mathbb{E}[\Gamma_j]^\top \Sigma(\Gamma_j) \mathbb{E}[\Gamma_j] \right).$$

Likewise, we evaluate the asymptotic normal limiting distribution of  $\hat{D}_{n,k}(\mathbf{X})$ . Recall that  $\Lambda_j = [Y_{jk}, Y_{j(k-1)}, Z_{jk}, Z_{j(k-1)}]^\top$ . Again, by Theorem 1.7 of Ibragimov (1962) and the Cramér-Wold device, as  $\mathbf{Z}_k$  is strictly stationary with finite absolute moments and summable mixing coefficients,

$$n^{-1/2} \sum_{j=1}^n [\Lambda_j - \mathbb{E}[\Lambda_j]] \xrightarrow{d} N(0, \Sigma(\Lambda_j)),$$

where each component of  $\Sigma(\Lambda_j)$  is non-zero and finite. Therefore, by the Delta Method,

$$n^{1/2} \left( \hat{D}_{n,k}(\mathbf{X}) - \frac{\mathbb{E}[Y_{jk}]}{\mathbb{E}[Y_{j(k-1)}]} - \left( 1 - \frac{\mathbb{E}[Z_{jk}]}{\mathbb{E}[Z_{j(k-1)}]} \right) \right) \xrightarrow{d} N\left(0, \mathbb{E}[\Lambda_j]^\top \Sigma(\Lambda_j) \mathbb{E}[\Lambda_j]\right).$$

□

**Remark F.1.** Note that  $\mathbb{E}[Y_{ijk}] / \mathbb{E}[Y_{ij(k-1)}]$  is equal to the probability of a success following  $k$  consecutive successes, given by  $\theta_P^k(\mathbb{P}_i)$ . Likewise, the asymptotic mean of  $\hat{D}_{n,k}(\mathbf{X})$  is equal to the difference in the probability of successes following  $k$  consecutive successes and failures, given by  $\theta_D^k(\mathbb{P}_i)$ . The parameters  $\theta_P^k(\mathbb{P}_i)$  and  $\theta_D^k(\mathbb{P}_i)$  are functionals of the underlying stationary process  $\mathbb{P}_i$  and the value of  $k$ .

Theorem F.1 implies that

$$\begin{aligned} \sqrt{n} \left( \left( \hat{P}_{n,k}(\mathbf{X}_i) - \hat{p}_{n,i} \right) - \theta_P^k(\mathbb{P}_i) \right) &\xrightarrow{d} N(0, \tau_P^2(\mathbb{P}_i, k)) \text{ and} \\ \sqrt{n} \left( \hat{D}_{n,k}(\mathbf{X}_i) - \theta_D^k(\mathbb{P}_i) \right) &\xrightarrow{d} N(0, \tau_D^2(\mathbb{P}_i, k)) \end{aligned}$$

where the limiting variances  $\tau_P^2(\mathbb{P}_i, k)$  and  $\tau_D^2(\mathbb{P}_i, k)$  are also parameters or functionals of the underlying process  $\mathbb{P}_i$  and  $k$ . In particular,  $\tau_D^2(\mathbb{P}_i, k) = \mathbb{E}[\Lambda_{ij}]^\top \Sigma(\Lambda_{ij}) \mathbb{E}[\Lambda_{ij}]$ , as in part (iii) of Theorem F.1. If  $\hat{\tau}_P^2(k)$  and  $\hat{\tau}_D^2(k)$  are consistent estimators of  $\tau_P^2(\mathbb{P}_i, k)$  and  $\tau_D^2(\mathbb{P}_i, k)$ , then  $\hat{P}_{n,k}(\mathbf{X}_i) \pm \hat{\tau}_P(k) \frac{z_{1-\alpha/2}}{\sqrt{n}}$  and  $\hat{D}_{n,k}(\mathbf{X}_i) \pm \hat{\tau}_D(k) \frac{z_{1-\alpha/2}}{\sqrt{n}}$  are asymptotically valid confidence intervals for  $\theta_P^k(\mathbb{P}_i)$  and  $\theta_D^k(\mathbb{P}_i)$  respectively. Of course, when  $H_0^i$  is true,  $\tau_P^2(\mathbb{P}_i, k) = \sigma_P^2(p_i, k)$ , where  $p_i$  is the marginal probability of success at any time point for the process  $\mathbb{P}_i$ . ■

## G Additional Methods for Joint Hypothesis Testing

In this section, we outline three additional choices for joint test statistics that combine  $p$ -values of individual permutation tests across individuals. We then outline two methods for combining  $p$ -values of different joint tests to compute a single composite  $p$ -value. We estimate the power of these methods with a simulation and present the results of their application to the GVT controlled shooting experiment.

## G.1 Combining Results for Several Individuals with One Statistic

First, let  $\hat{Q}_{n,k}(\mathbf{X}_i)$  denote the proportion of zeros following  $k$  consecutive zeros. Recalling that,  $Z_{ijk} = \prod_{l=j}^{j+k} (1 - X_{il})$  and  $W_{ik} = \sum_{j=1}^{n-k} Z_{ijk}$ , then  $\hat{Q}_{n,k}(\mathbf{X}_i)$  is given by

$$\hat{Q}_{n,k}(\mathbf{X}_i) = W_{ik} / W_{i(k-1)}.$$

In this section, we specify three additional procedures for testing the joint hypothesis  $H_0$  using a single test statistic  $\hat{G}_{n,k}(\mathbf{X}_i)$ , given a choice of  $G \in \{D, P, Q\}$  and a value of  $k$ .

**Minimum  $p$ -value:** Let  $\rho_G(k, i)$  denote the  $p$ -value for individual  $i$  for a test of the hypothesis  $H_0^i$  which rejects for extreme values of  $\hat{G}_{n,k}(\mathbf{X}_i)$ . The minimum  $p$ -value joint hypothesis testing procedure rejects for small values of  $\hat{\psi}_{G,k} = \min_{1 \leq i \leq s} (\rho_G(k, i))$ . The critical values of the test rejecting for small values of  $\hat{\psi}_{G,k}$  can be approximated by the stratified permutation distribution of  $\hat{\psi}_{G,k}$ .

**Fisher's Method:** The Fisher joint hypothesis test statistic (Fisher, 1925) is given by

$$\hat{f}_{G,k} = -2 \sum_i \log(\rho_G(k, i)).$$

If  $\rho_G(k, i)$  are  $p$ -values for independent tests, then  $\hat{f}_{G,k}$  has a chi-squared distribution with  $2 \cdot s$  degrees of freedom under  $H_0$ . However, we need to account for the fact that  $\hat{D}_{n,k}(\mathbf{X}_i)$  and  $\hat{P}_{n,k}(\mathbf{X}_i)$  can be undefined for some sequences. By assigning a  $p$ -value of 1 to these sequences, the critical values of the test rejecting for large values of  $\hat{f}_{G,k}$  can be approximated with the stratified permutation distribution of  $\hat{f}_{G,k}$ .

**Tukey's Higher Criticism:** The Tukey Higher Criticism test statistic is given by

$$\hat{T}_{G,k} = \max_{0 < \delta < \delta_0} [T_\delta] = \max_{0 < \delta < \delta_0} \left[ \frac{\sqrt{\tilde{s}} (\xi_\delta - \delta)}{\sqrt{\delta(1 - \delta)}} \right], \quad (\text{G.1})$$

where

$$\xi_\delta = \tilde{s}^{-1} \sum_{i: \hat{G}_{n,k}(\mathbf{X}_i) \text{ is defined}} \mathbb{I} \{ \rho_G(k, i) \leq \delta \} \quad (\text{G.2})$$

is the fraction of individuals that are significant at level  $\delta$  for a given test of  $H_0^i$  rejecting for large values of  $\hat{G}_{n,k}(\mathbf{X}_i)$ ,  $\tilde{s}$  is the number of individuals for which  $\hat{G}_{n,k}(\mathbf{X}_i)$  is defined,  $\delta_0$  is a tuning parameter, and  $\mathbb{I} \{ \cdot \}$  is the indicator function. Again, critical values of the test rejecting for large values of  $\hat{T}_{G,k}$  can be approximated with the stratified permutation distribution of  $\hat{T}_{G,k}$ . See Donoho and Jin (2004) for further discussion. MS implement binomial tests (Clopper and Pearson, 1934) that reject for large proportions of significant individuals. A binomial test chooses a specified threshold of significance  $\delta$ , and rejects  $H_0$  at level  $\alpha$  if the number of individuals significant at

level  $\delta$  exceeds the  $1 - \alpha$  quantile of the distribution of a binomial variable with parameters  $s$  and  $\delta$ . Tukey's Higher Criticism is a refinement of this testing procedure that allows for a data-driven choice of the significance threshold  $\delta$ .

## G.2 Combining the Results of Several Joint Test Statistics

The results of any of the procedures that test the joint hypothesis for a single test statistic can be combined with the results from tests using different test statistics with Fisher's method or by computing the minimum  $p$ -value. Specifically, let  $\rho_G(k)$  be the  $p$ -value of a test of the joint null hypothesis using the test statistic  $\hat{G}_{n,k}(\mathbf{X}_i)$  for  $G \in \{D, P, Q\}$  and  $k$  in  $1, \dots, K$ . The Fisher test statistic is given by

$$\hat{\mathbf{F}} = -2 \log \sum_{G \in \{D, P, Q\}} \sum_{k=1}^K \rho_G(k) \quad (\text{G.3})$$

and the minimum  $p$ -value test statistic is given by

$$\hat{\Psi} = \min \{ \rho_G(k) \mid G \in \{D, P, Q\}, 1 \leq k \leq K \}. \quad (\text{G.4})$$

The critical values for the tests rejecting for large values of  $\hat{\mathbf{F}}$  and small values of  $\hat{\Psi}$  can be approximated with the stratified permutation distribution of  $\hat{\mathbf{F}}$  and  $\hat{\Psi}$ , respectively.

## G.3 Power Simulations

Online Appendix Figure 6 displays contours of the power surface on  $\epsilon$  and  $\zeta$  for the stratified permutation test rejecting at level 0.05 for large values of  $\bar{D}_1(\mathbf{X})$  against the streaky alternative specified in Section 4.1 for  $n$  equal to 100,  $s$  equal to 26, and  $m = 1$ . For each  $\epsilon$  and  $\zeta$  on a two dimensional grid, we measure the power of the stratified permutation tests that combine the  $p$ -values of the individual permutation tests that use  $\hat{D}_{n,1}(\mathbf{X}_i)$  with simulation by drawing and implementing the test on 1,000 replicates of  $s$  sequences. We group the estimates of power into five colored regions. The colored regions denote the set of  $\epsilon$  and  $\zeta$  values with estimated power in the intervals  $(0, 0.15]$ ,  $(0.15, 0.40]$ ,  $(0.40, 0.65]$ , and  $(0.65, 0.90]$ .

## G.4 Application to GVT

Online Appendix Table 3 presents the  $p$ -values for the four tests of  $H_0$  outlined in this Appendix implemented with each test statistic  $\hat{D}_{n,k}(\mathbf{X}_i)$ ,  $\hat{P}_{n,k}(\mathbf{X}_i)$ , and  $\hat{Q}_{n,k}(\mathbf{X}_i)$  for each  $k$  between 1 and 4. The majority of tests using individual test statistics reject  $H_0$  at the 5% level. The Fisher test statistic  $\hat{\mathbf{F}}$ , specified in (G.3), is highly significant for the test using the means of the test statistics, for Tukey's Higher Criticism, and for the test using the minimum  $p$ -value.  $\hat{\mathbf{F}}$  is significant at the 10% level for the test using the Fisher test statistic. The minimum  $p$ -value test statistic  $\hat{\Psi}$  is highly significant for all four tests.

The rejection of  $H_0$  at the 5% level is not robust to the exclusion of Shooter 109 from the sample. Online Appendix Table 3 also displays the  $p$ -values for the tests of  $H_0$  implemented

Online Appendix Figure 6: Power Contours for Permutation Tests of Joint Null

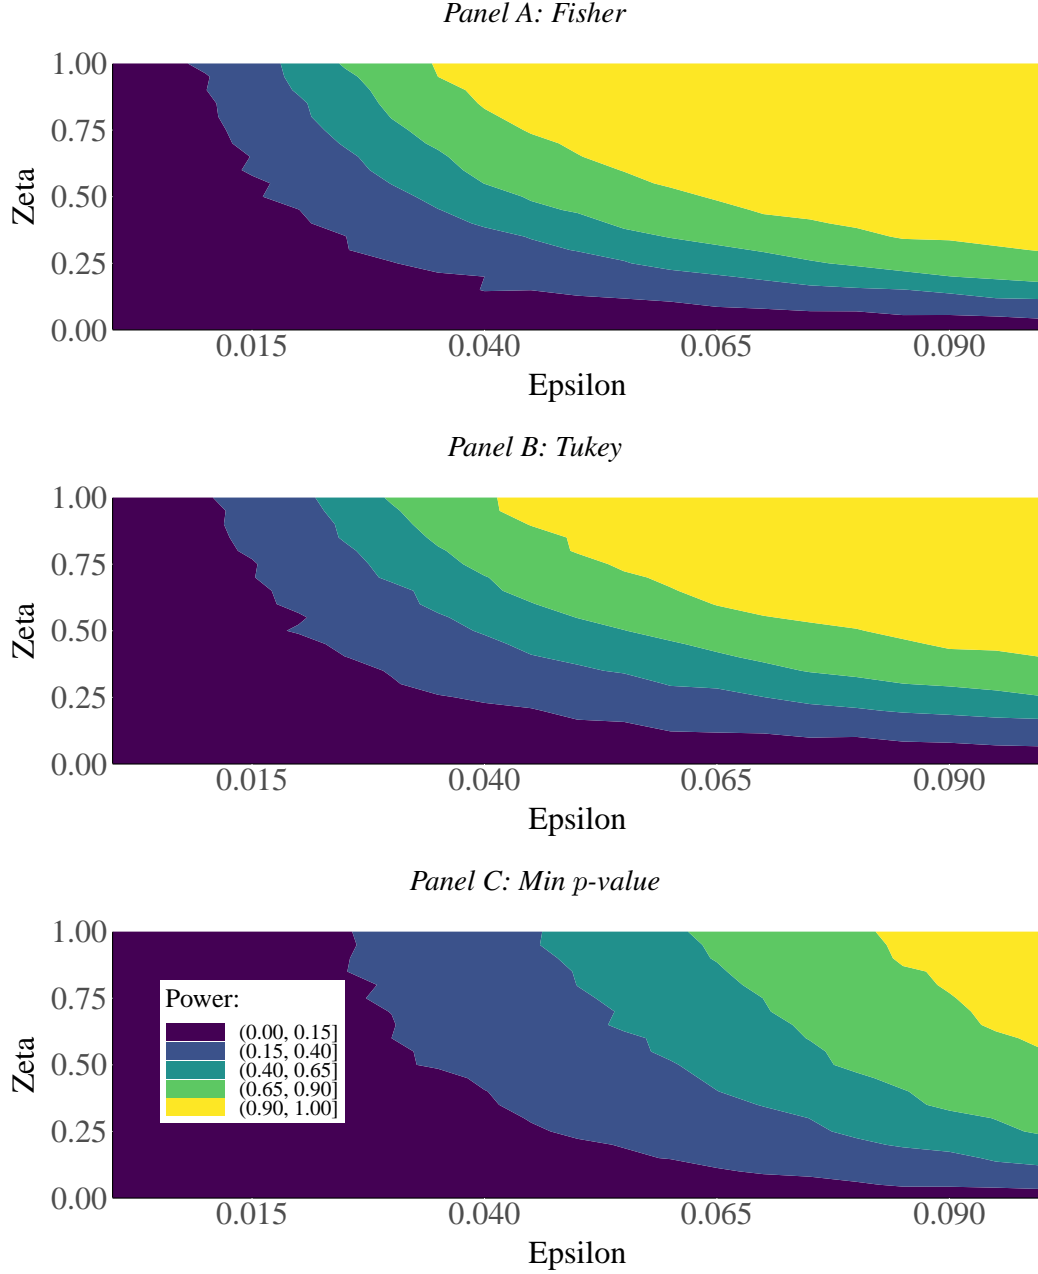

Notes: Figure displays contours of the power surface on  $\epsilon$  and  $\zeta$  for the stratified permutation tests of the joint null using the test statistic  $\hat{D}_{n,k}(\mathbf{X})$  for  $k = 1$  at level 0.05 against the streaky alternative specified in Section 4.1 for  $n$  equal to 100,  $s$  equal to 26, and  $m = 1$ . We draw 1,000 replicates of  $s$  Bernoulli sequences  $\mathbf{X}_i$  according to the streaky alternative specified in Section 4.1 with  $m = 1$  for each  $\epsilon$  and  $\zeta$ . The estimate of the power at each  $\epsilon$  and  $\zeta$  is given by the proportion of replicates in which the stratified permutation tests using the test statistic  $\hat{D}_{n,k}(\mathbf{X})$  for  $k = 1$  rejects  $H_0$  at level 0.05. The estimates of power are grouped into five colored regions. The colored regions correspond to the set of  $\epsilon$  and  $\zeta$  values with estimated power in five mutually exclusive intervals on  $(0, 1]$ .

without the inclusion of Shooter 109 in the sample. Now, at most three of the  $p$ -values for tests of  $H_0$  using a single test statistic for each method of testing the joint null are significant at the 5% level.  $\hat{F}$  and  $\hat{\Psi}$  are no longer significant at the 5% level for tests using the means of the test statistics over shooters and Tukey's Higher Criticism and are no longer significant at the 10% level for tests using the minimum  $p$ -value and Fisher's test statistic.

## H Asymptotic Power Approximations for General $m$ and $k$

We generalize the results of Section 4.3 to consider cases with  $m$  and  $k$  potentially greater than one. Again, we begin by characterizing the limiting distributions of the plug-in test statistics computed on  $\mathbf{X}_i$  for a streaky individual.

**Theorem H.1.** *Let  $0 \leq \epsilon < \frac{1}{2}$ . Assume  $\mathbf{X}_i = \{X_{ij}\}_{j=1}^n$  is a two-state stationary Markov chain of order  $2^m$  on  $\{0, 1\}$  such that the probability of transitioning from one to one (zero to zero) is  $\frac{1}{2} + \epsilon$  after  $m$  successive ones (zeros) and is  $\frac{1}{2}$  otherwise, then*

$$\begin{aligned} \sqrt{n} \left( \hat{P}_{n,k}(\mathbf{X}_i) - \hat{p}_{n,i} - \mu_P(k, m, \epsilon) \right) &\xrightarrow{d} N(0, \sigma_P^2(k, m, \epsilon)), \text{ and} \\ \sqrt{n} \left( \hat{D}_{n,k}(\mathbf{X}_i) - \mu_D(k, m, \epsilon) \right) &\xrightarrow{d} N(0, \sigma_D^2(k, m, \epsilon)) \end{aligned}$$

where  $\mu_P(k, m, \epsilon)$  and  $\mu_D(k, m, \epsilon)$  are given explicitly in the proof and  $\sigma_P^2(k, m, \epsilon)$  and  $\sigma_D^2(k, m, \epsilon)$  are functions of  $k$ ,  $m$ , and  $\epsilon$ .

*Proof.* We can rewrite the problem as a  $2^m$  state Markov Chain of order 2 on  $\prod_{j=1}^m \{0, 1\}$ . For example, suppose  $m = 2$ , then a transition from  $\{0, 1\}$  to  $\{1, 0\}$  occurs in the second position of the sequence  $\{0, 1, 0\}$ .

Let the  $j^{\text{th}}$  state be an  $m$ -tuple on  $\{0, 1\}$  denoted by  $\{I_m^j, \dots, I_1^j\}$ . The states are enumerated such that  $I_m^j I_{m-1}^j \dots I_1^j$  is  $j - 1$  expressed in the base 2 numeral system, i.e.  $\{1, 0, 0, 0\}$  is the 9<sup>th</sup> state when  $m = 4$ . Throughout this proof, we let  $j$  denote the state  $\{I_m^j, \dots, I_1^j\}$ .

Let  $l = 2^{m-1}$  and  $j' = j \pmod{l}$ . If the Markov Chain is in state  $j$ , then it can only transition to states  $2j' - 1 = \{I_{m-1}^j, \dots, 0\}$  and  $2j' = \{I_{m-1}^j, \dots, 1\}$ , as appending a 0 to the end of an integer expressed base 2 is equivalent to multiplication by 2, removing the first digit of an integer  $\geq 2^{m-1}$  and  $\leq 2^m$  expressed base 2 is equivalent to taking  $\pmod{l}$ , and  $\{I_m^{2r}, \dots, I_2^{2r}\} = \{I_m^{2r-1}, \dots, I_2^{2r-1}\}$  for all  $0 \leq r \leq l$ .

Let the stationary distribution of the Markov Chain be denoted by  $\pi = (\pi_1, \dots, \pi_{2^m})$  and the probability from transitioning from state  $j$  to state  $d$  be denoted by  $\varrho(j, d)$ . In general,  $\pi$  must satisfy the system of  $2^m + 1$  equations

$$\begin{aligned} \pi_1 \varrho(1, 1) + \pi_{l+1} \varrho(l+1, 1) &= \pi_1 \\ \pi_1 \varrho(1, 2) + \pi_{l+1} \varrho(l+1, 2) &= \pi_1 \\ &\vdots \end{aligned}$$

|                           | $k$ | Mean $\bar{G}_k$ |         | Min. $p$ -value $\hat{\psi}_{G,k}$ |         | Fisher $\hat{f}_{G,k}$ |         | Tukey HC $\hat{T}_{G,k}$ |         |
|---------------------------|-----|------------------|---------|------------------------------------|---------|------------------------|---------|--------------------------|---------|
|                           |     | w/ 109           | w/o 109 | w/ 109                             | w/o 109 | w/109                  | w/o 109 | w/109                    | w/o 109 |
| $\hat{D}_k(\mathbf{X}_i)$ | 1   | 0.1464           | 0.3678  | 0.0030                             | 0.4940  | 0.0428                 | 0.3654  | 0.1079                   | 0.2165  |
|                           | 2   | 0.0402           | 0.1261  | 0.0010                             | 0.0354  | 0.0021                 | 0.0648  | 0.2834                   | 0.4096  |
|                           | 3   | 0.0036           | 0.0125  | 0.0204                             | 0.1279  | 0.0021                 | 0.0213  | 0.0483                   | 0.0678  |
|                           | 4   | 0.0716           | 0.1294  | 0.1404                             | 0.1346  | 0.0054                 | 0.0165  | 0.0079                   | 0.0213  |
| $\hat{P}_k(\mathbf{X}_i)$ | 1   | 0.1548           | 0.3520  | 0.0008                             | 0.4868  | 0.0150                 | 0.2939  | 0.0096                   | 0.0417  |
|                           | 2   | 0.0323           | 0.0879  | 0.0021                             | 0.1273  | 0.0047                 | 0.0911  | 0.0001                   | 0.5405  |
|                           | 3   | 0.0418           | 0.0882  | 0.0131                             | 0.3555  | 0.0385                 | 0.2470  | 0.2445                   | 0.3299  |
|                           | 4   | 0.3035           | 0.4095  | 0.2721                             | 0.2642  | 0.1690                 | 0.3337  | 0.5154                   | 0.6729  |
| $\hat{Q}_k(\mathbf{X}_i)$ | 1   | 0.1492           | 0.3917  | 0.0035                             | 0.4916  | 0.0631                 | 0.4340  | 0.0571                   | 0.2777  |
|                           | 2   | 0.1891           | 0.3446  | 0.1356                             | 0.2796  | 0.1398                 | 0.3679  | 0.0113                   | 0.2764  |
|                           | 3   | 0.0126           | 0.0259  | 0.1539                             | 0.1458  | 0.0279                 | 0.0459  | 0.0877                   | 0.1502  |
|                           | 4   | 0.0361           | 0.0555  | 0.3360                             | 0.3238  | 0.0543                 | 0.0566  | 0.0126                   | 0.0097  |
| $\hat{\mathbf{F}}$        |     | 68.6796          | 49.6754 | 96.2418                            | 36.5842 | 93.0266                | 51.2112 | 82.2148                  | 46.7255 |
| $p$ -value                |     | 0.0191           | 0.0746  | 0.0002                             | 0.1342  | 0.0849                 | 0.1339  | 0.0019                   | 0.0672  |
| $\hat{\Psi}$              |     | 0.0036           | 0.0125  | 0.0008                             | 0.0354  | 0.0021                 | 0.0165  | 0.0001                   | 0.0097  |
| $p$ -value                |     | 0.0271           | 0.0828  | 0.0041                             | 0.21097 | 0.0907                 | 0.1509  | 0.0016                   | 0.0880  |

Online Appendix Table 3: Tests of the Joint Null Hypothesis  $H_0$   
with and without Shooter 109

Notes: Table displays the  $p$ -values for four tests of the joint null hypothesis  $H_0$  for  $\hat{D}_k(\mathbf{X}_i)$ ,  $\hat{P}_k(\mathbf{X}_i)$ , or  $\hat{Q}_k(\mathbf{X}_i)$  and each  $k$  in  $1, \dots, 4$  with and without the inclusion of shooter 109. The minimum  $p$ -value procedure, Fisher joint hypothesis testing procedure, and Tukey's Higher Criticism procedure use the  $p$ -values from the one-sided individual shooter permutation test. We choose  $\delta_0 = 0.5$  for computing  $\hat{T}_{G,k}$ . The  $p$ -values for all four procedures are estimated by permuting each shooter's observed shooting sequence 100,000 times, computing the test statistics for each set of permuted shooting sequences, and computing the proportion of test statistics greater than or equal to the observed test statistics. We compute Fisher's statistic  $\hat{\mathbf{F}}$  for all four procedures by taking  $-2$  times the log of the sum of the  $p$ -values for each  $\hat{D}_k(\mathbf{X}_i)$ ,  $\hat{P}_k(\mathbf{X}_i)$ , or  $\hat{Q}_k(\mathbf{X}_i)$  and each  $k$  in  $1, \dots, 4$ . We compute the minimum  $p$ -value statistic  $\hat{\Psi}$  for all four procedures by taking the minimum of the  $p$ -values for each  $\hat{D}_k(\mathbf{X}_i)$ ,  $\hat{P}_k(\mathbf{X}_i)$ , or  $\hat{Q}_k(\mathbf{X}_i)$  and each  $k$  in  $1, \dots, 4$ . The  $p$ -values for  $\hat{\mathbf{F}}$  and  $\hat{\Psi}$  are computed by estimating the stratified permutation distributions of  $\hat{\mathbf{F}}$  and  $\hat{\Psi}$ .

$$\begin{aligned}
\pi_j \varrho(j, 2j-1) + \pi_{l+j} \varrho(l+j, 2j-1) &= \pi_{2j-1} \\
\pi_j \varrho(j, 2j) + \pi_{l+j} \varrho(l+j, 2j) &= \pi_{2j} \\
&\vdots \\
\pi_l \varrho(l, 2^m-1) + \pi_{2^m} \varrho(2^m, 2^m-1) &= \pi_{2^m-1} \\
\pi_l \varrho(l, 2^m) + \pi_{2^m} \varrho(2^m, 2^m) &= \pi_{2^m} \\
\sum_{j=1}^{2^m} \pi_j &= 1
\end{aligned} \tag{H.1}$$

In the Markov Chain we consider,  $\varrho(1, 1) = \varrho(2^k, 2^k) = \frac{1}{2} + \epsilon$ ,  $\varrho(1, 2) = \varrho(2^k, 2^k - 1) = \frac{1}{2} - \epsilon$ ,  $\varrho(j, 2j-1) = \varrho(j, 2j) = \varrho(l+j, 2j-1) = \varrho(l+j, 2j) = \frac{1}{2}$  for all  $j$  in  $1, \dots, l$ , and all other transition probabilities be equal to 0.

We find that, in this model,

$$\pi_j = \begin{cases} \frac{1}{2+(2^m-2)(1-2\epsilon)} & \text{for } j = 1, 2^m \\ \frac{1-2\epsilon}{2+(2^m-2)(1-2\epsilon)} & \text{for } 2 \leq j \leq 2^{m-1}. \end{cases} \tag{H.2}$$

It is straightforward to show that the stationary distribution given by (H.2) satisfies the system of equations (H.1) and is therefore the stationary distribution of the Markov chain under consideration.

Let  $\mathcal{I}^m = \{0, 1\}^m$  be the set of sequences of zeros and ones of length  $m$ . Let  $\mathcal{I}_q^m \subset \mathcal{I}^m$  be the set of sequences of zeros and ones of length  $m$  where the first  $q$  elements are ones, the  $q+1$ <sup>th</sup> element is a 0, and elements  $q+2$  through  $m$  are either zeros or ones. Note that  $\{\mathcal{I}_0^m, \dots, \mathcal{I}_k^m\}$  is a partition of  $\mathcal{I}^m$  and that the cardinality of  $\mathcal{I}_q^m$  is  $2^{m-q-1}$  for  $0 \leq q < k$  and 1 for  $q = m$ . Finally, let  $\mathcal{I}_{1+}^m = \mathcal{I}^m \setminus \mathcal{I}_0^m$ .

We consider the case with  $s = 1$ , and therefore drop the dependence on the individual  $i$ . We can see that, for  $k \geq m-1$ ,

$$\begin{aligned}
\mathbb{E}[Y_{jk}] &= \sum_{I \in \mathcal{I}_{1+}^m} \mathbb{P}(X_{j+1} = 1, \dots, X_{j+k} = 1 | (X_j, \dots, X_{j-m+1}) = I) \mathbb{P}((X_j, \dots, X_{j-m+1}) = I) \\
&= \sum_{q=1}^{m-1} 2^{m-q-1} \left(\frac{1}{2}\right)^{m-q} \left(\frac{1}{2} + \epsilon\right)^{k-m+q} \left(\frac{1-2\epsilon}{2+(2^m-2)(1-2\epsilon)}\right) \\
&\quad + \left(\frac{1}{2} + \epsilon\right)^k \left(\frac{1}{2+(2^m-2)(1-2\epsilon)}\right) \\
&= \frac{\left(\frac{1}{2} + \epsilon\right)^{k-m+1}}{2+(2^m-2)(1-2\epsilon)}.
\end{aligned}$$

Likewise, for  $1 \leq k < m - 1$ ,

$$\begin{aligned}
\mathbb{E}[Y_{jk}] &= \sum_{I \in \mathcal{I}_{1+}^m} \mathbb{P}(X_{j+1} = 1, \dots, X_{j+k} = 1 | (X_j, \dots, X_{j-m+1}) = I) \mathbb{P}((X_j, \dots, X_{j-m+1}) = I) \\
&= \sum_{q=1}^{m-k} 2^{m-q-1} \left(\frac{1}{2}\right)^k \left(\frac{1-2\epsilon}{2 + (2^m - 2)(1-2\epsilon)}\right) \\
&\quad + \sum_{q=m-k+1}^{m-1} 2^{m-q-1} \left(\frac{1}{2}\right)^{m-q} \left(\frac{1}{2} + \epsilon\right)^{k-m+q} \left(\frac{1-2\epsilon}{2 + (2^m - 2)(1-2\epsilon)}\right) \\
&\quad + \left(\frac{1}{2} + \epsilon\right)^k \left(\frac{1}{2 + (2^m - 2)(1-2\epsilon)}\right) \\
&= \frac{2^{m-k-1} + (2 - 2^{m-k})\epsilon}{2 + (2^m - 2)(1-2\epsilon)}.
\end{aligned}$$

Finally,  $\mathbb{E}[Y_{jk}] = \frac{1}{2}$  for  $k = 0$ .

Therefore, by Theorem F.1,  $\hat{P}_{n,k}(\mathbf{X}) - \hat{p}_n$  is asymptotically normal with limiting distribution given by

$$n^{1/2} \left( \hat{P}_{n,k}(\mathbf{X}) - \hat{p} - \mu_P(k, m, \epsilon) \right) \xrightarrow{d} N(0, \sigma_{\hat{P}}^2(k, m, \epsilon)),$$

where

$$\mu_{\hat{P}}(k, m, \epsilon) = \begin{cases} \epsilon & \text{if } m \leq k \\ \frac{\epsilon}{2(1-\epsilon)} & \text{if } k = m - 1 \\ \frac{\epsilon}{2^{m-k} + (2 - 2^{m-k+1})\epsilon} & \text{if } 1 < k < m - 1 \\ \frac{2}{2 + (2^m - 2)(1-2\epsilon)} & \text{if } k = 1 \end{cases}$$

and  $\sigma_{\hat{P}}^2(k, m, \epsilon)$  is a function of  $k$ ,  $m$ , and  $\epsilon$ .  $\hat{D}_{n,k}(\mathbf{X})$  is asymptotically normal with limiting distribution given by

$$n^{1/2} \left( \hat{D}_{n,k}(\mathbf{X}) - \mu_D(k, m, \epsilon) \right) \xrightarrow{d} N(0, \sigma_D^2(k, m, \epsilon)).$$

where

$$\mu_D(k, m, \epsilon) = \begin{cases} 2\epsilon & \text{if } m \leq k \\ \frac{\epsilon}{1-\epsilon} & \text{if } k = m - 1 \\ \frac{\epsilon}{2^{m-k-1} + (1 - 2^{m-k})\epsilon} & \text{if } 1 < k < m - 1 \\ \frac{4\epsilon}{2 + (2^m - 2)(1-2\epsilon)} & \text{if } k = 1 \end{cases}$$

and  $\sigma_D^2(k, m, \epsilon)$  is a function of  $k$ ,  $m$ , and  $\epsilon$ . □

**Remark H.1.** The functions  $\sigma_{\hat{P}}^2(k, m, \epsilon)$  and  $\sigma_D^2(k, m, \epsilon)$  are continuous in  $\epsilon$ , so if we take  $\epsilon_n = \frac{h}{\sqrt{n}}$  then we expect that  $\sigma_{\hat{P}}^2(k, m, \epsilon)$  and  $\sigma_D^2(k, m, \epsilon)$  would converge to the asymptotic variances of  $\hat{P}_{n,k}(\mathbf{X}_i) - \hat{p}_{n,i}$  and  $\hat{D}_{n,k}(\mathbf{X}_i)$  under  $H_0$ , respectively. This is verified formally for the case

of  $m = 1$  in Section 4.3 and can be shown more generally by tracing the proof of Theorem 4.1, though the details are omitted. Therefore, if  $\epsilon_n = \frac{h}{\sqrt{n}}$ , then

$$\begin{aligned}\sqrt{n} \left( \hat{P}_{n,k}(\mathbf{X}_i) - \hat{p}_{n,i} - \mu_P(k, m, \epsilon_n) \right) &\xrightarrow{d} N(0, \sigma_P^2(1/2, k)), \\ \sqrt{n} \left( \hat{D}_{n,k}(\mathbf{X}_i) - \mu_D(k, m, \epsilon_n) \right) &\xrightarrow{d} N(0, \sigma_D^2(1/2, k)),\end{aligned}$$

where  $\sigma_P^2(1/2, k)$  and  $\sigma_D^2(1/2, k)$  are the asymptotic variances of  $\hat{P}_{n,k}(\mathbf{X}_i) - \hat{p}_{n,i}$  and  $\hat{D}_{n,k}(\mathbf{X}_i)$  under  $H_0$ , given by Theorem 3.1.  $\blacksquare$

**Remark H.2.** Define the limiting constant

$$\phi_T(k, m, h) = \lim_{n \rightarrow \infty} \frac{\sqrt{n} \mu_T(k, m, \epsilon_n)}{\sqrt{\sigma_T^2(1/2, k)}} \quad (\text{H.3})$$

for  $T$  equal to  $P$  or  $D$ , where  $\epsilon_n = h/\sqrt{n}$ . Observe that if  $\mathbf{X}_i = \{X_{ij}\}_{j=1}^n$  is a Bernoulli sequence associated with a streaky individual with  $\epsilon_n = h/\sqrt{n}$ , then

$$\begin{aligned}\mathbb{P} \left( \frac{\sqrt{n} \hat{D}_{n,k}(\mathbf{X}_i)}{\sqrt{\sigma_D^2(1/2, k)}} > z_{1-\alpha} \right) &= \mathbb{P} \left( \sqrt{n} \left( \frac{\hat{D}_{n,k}(\mathbf{X}_i)}{\sqrt{\sigma_D^2(1/2, k)}} - \frac{\mu_D(k, m, \epsilon_n)}{\sqrt{\sigma_D^2(1/2, k)}} \right) > z_{1-\alpha} - \frac{\sqrt{n} \mu_D(k, m, \epsilon_n)}{\sqrt{\sigma_D^2(1/2, k)}} \right) \\ &\rightarrow 1 - \Phi(z_{1-\alpha} - \phi_D(k, m, h)).\end{aligned}$$

and similarly for  $\hat{P}_{n,k}(\mathbf{X}_i) - \hat{p}_{n,i}$ , where  $z_{1-\alpha}$  is the  $1 - \alpha$  quantile of the standard normal distribution. This argument implies the following Corollary.  $\blacksquare$

**Corollary H.1.** *Consider the permutation test of the null hypothesis  $H_0^i$  that the Bernoulli sequence  $\mathbf{X}_i = \{X_{ij}\}_{j=1}^n$  is independent and identically distributed rejecting for large values of the test statistic  $T_n$ . The power of this test against the alternative that  $\mathbf{X}_i$  is a two-state Markov chain of order  $2^m$  on  $\{0, 1\}$  such that the probability of transitioning from one to one (zero to zero) is  $\frac{1}{2} + \epsilon$  after  $m$  successive ones (zeros) and is  $\frac{1}{2}$  otherwise and  $\epsilon = h/\sqrt{n}$  converges to*

$$1 - \Phi(z_{1-\alpha} - \phi_T(k, m, h)),$$

where  $\phi_T(k, m, h)$  is given by (H.3) as  $n \rightarrow \infty$  if the test statistic  $T_n$  is equal to  $\hat{P}_{n,1}(\mathbf{X}_i) - \hat{p}_{n,i}$  or  $\hat{D}_{n,1}(\mathbf{X}_i)$ .

Next, we characterize the limiting distributions of  $\bar{P}_k(\mathbf{X})$  and  $\bar{D}_k(\mathbf{X})$  under the Markov chain streaky alternatives specified in Section 4.3 for general  $m$ . We then derive an expression for limiting power of stratified permutation tests of  $H_0$  against these alternatives that use  $\bar{P}_k(\mathbf{X})$  and  $\bar{D}_k(\mathbf{X})$  as test statistics.

**Corollary H.2.** *Assume that a population of  $s$  individuals are associated with the two-state stationary Markov chains  $\mathbf{X}_i = \{X_{ij}\}_{j=1}^\infty$  on  $\{0, 1\}$  for each  $i$  in  $1, \dots, s$ , such that each sequence  $\mathbf{X}_i$*

has probability  $\zeta$  of satisfying the condition that the probability of transitioning from one to one (zero to zero) is  $\frac{1}{2} + \epsilon$  after  $m$  successive ones (zeros) and  $\frac{1}{2}$  for all other sequences of  $m$  ones and zeros with  $\epsilon = h/\sqrt{ns}$  and is otherwise independent and identically distributed Bernoulli(1/2), then

(i)  $\bar{P}_k$ , given by (2.6), is asymptotically normal with limiting distribution given by

$$\sqrt{ns}\bar{P}_k(\mathbf{X}) \xrightarrow{d} N\left(\sigma_P(1/2, k) \cdot \phi_P(k, m, h) \cdot \zeta, \sigma_P^2(1/2, k)\right),$$

and

(ii)  $\bar{D}_k$ , given by (2.6), is asymptotically normal with limiting distribution given by

$$\sqrt{ns}\bar{D}_k(\mathbf{X}) \xrightarrow{d} N\left(\sigma_D(1/2, k) \cdot \phi_D(k, m, h) \cdot \zeta, \sigma_D^2(1/2, k)\right)$$

as  $n \rightarrow \infty$  and  $s \rightarrow \infty$ .

(iii) Furthermore, the power of the stratified permutation test of the joint null hypothesis  $H_0$  rejecting for large values of the test statistic  $K_{n,s}$ , for  $K_{n,s}$  equal to  $\bar{P}_k(\mathbf{X})$  or  $\bar{D}_k(\mathbf{X})$ , against the alternative specified in the conditions of this corollary, converges to

$$1 - \Phi(z_{1-\alpha} - \phi_T(k, m, h) \cdot \zeta)$$

for  $T$  equal  $P$  or  $D$ , respectively, as  $n \rightarrow \infty$  and  $s \rightarrow \infty$ .

## I Asymptotic Equivalence to the Wald-Wolfowitz Runs Test

Given a Bernoulli sequence  $\mathbf{X}_i = \{X_{ij}\}_{i=1}^n$ , define the number of runs by

$$WW_n(\mathbf{X}_i) = \sum_{j=2}^n \mathbb{I}\{X_{ij} \neq X_{i(j-1)}\},$$

where  $\mathbb{I}\{\cdot\}$  is the indicator function.

The Wald-Wolfowitz Runs Test (Wald and Wolfowitz, 1940b) rejects for small values of the number of runs  $WW_n(\mathbf{X}_i)$ , or equivalently, for large values of

$$\hat{S}_{n,i}(\mathbf{X}_i) = \left( \frac{\frac{-WW(\mathbf{X}_i)}{2n} + \hat{p}_{n,i}(1 - \hat{p}_{n,i})}{\hat{p}_{n,i}(1 - \hat{p}_{n,i})} \right). \quad (\text{I.1})$$

As shown in Wald and Wolfowitz (1940b), under i.i.d. Bernoulli trials,  $\sqrt{n}\hat{S}_{n,i}(\mathbf{X}_i) \xrightarrow{d} N(0, 1)$ , so the runs test may use either  $z_{1-\alpha}$  or a critical value determined exactly from the permutation distribution. Note that the runs test is known to be the uniformly most powerful unbiased test against the Markov chain streaky alternatives considered in Section 4; see Lehmann and Romano (2005), Problems 4.29–4.31. The following Theorem shows the runs test is asymptotically equivalent to

the test based on  $\hat{D}_{n,1}(\mathbf{X}_i)$ .

**Theorem I.1.** *The Wald-Wolfowitz Runs Test and the test based on  $\hat{D}_{n,1}(\mathbf{X}_i)$  are asymptotically equivalent in the sense that they reach the same conclusion with probability tending to one, both under the null hypothesis and under contiguous alternatives. In particular, we show the following:*

(i) *Under independent and identically distributed Bernoulli trials,*

$$\sqrt{n} \left( \hat{D}_{n,1}(\mathbf{X}_i) - \hat{S}_{n,i}(\mathbf{X}_i) \right) \xrightarrow{P} 0. \quad (\text{I.2})$$

*Therefore, if both statistics are applied using  $z_{1-\alpha}$  as a critical value, they both lead to the same decision with probability tending to one.*

(ii) *Since (I.2) implies the same is true under contiguous alternatives to i.i.d. sampling (for some  $p_i$ ), the same conclusion holds.*

(iii) *The same conclusion holds if  $z_{1-\alpha}$  is replaced by critical values obtained by the permutation distribution.*

(iv) *Both tests have the same local limiting power functions under any sequence of contiguous alternatives (in the sense that if the local limiting power exists for one test, then it does for the other test with the same value), and in particular, under the Markov Chain streaky alternatives considered in Section 4, where the limiting local power function is given in Corollary H.1.*

*Proof.* We consider the case with  $s = 1$ , and therefore drop the dependence on the individual  $i$ . As before, let  $V_{n,1} = \sum_{j=1}^{n-1} X_j X_{j+1}$  and  $V_{n,0} = \sum_{j=1}^n X_j$ . Let  $WW_{n,0}$  denote the number of runs of zeros and  $WW_{n,1}$  the number of runs of ones, so that  $WW_n = WW_{n,0} + WW_{n,1}$ . Since the first success in a run of ones does not contribute to the sum  $V_{n,1}$ , the number of ones followed by a one in a particular run of ones is the number of ones in the run minus one. Therefore,  $V_{n,1} = V_{n,0} - WW_{n,1}$ . So, if  $WW$  is even,  $V_{n,1} = V_{n,0} - WW_n/2$ . On the other hand, if  $WW_n$  is odd, then there are either  $(WW_n - 1)/2$  or  $(WW_n + 1)/2$  runs of ones. It follows that

$$|V_{n,1} - \left( V_{n,0} - \frac{WW_n}{2} \right)| \leq \frac{1}{2}$$

or

$$\frac{V_{n,1}}{n} = \hat{p}_n - \frac{WW_n}{2n} + O_P(n^{-1}) \quad (\text{I.3})$$

where as before  $\hat{p} = V_{n,0}/n$ . In order to show (I.2), by K.7, it suffices to show

$$\sqrt{n} \left[ \left( \frac{\frac{V_{n,1}}{n} - \hat{p}_n^2}{\hat{p}_n(1 - \hat{p}_n)} \right) + \frac{\frac{WW_n}{2n} - \hat{p}_n(1 - \hat{p}_n)}{\hat{p}_n(1 - \hat{p}_n)} \right] \xrightarrow{P} 0,$$

or equivalently

$$\sqrt{n} \left[ \frac{V_{n,1}}{n} - \hat{p}_n^2 + \frac{WW_n}{2n} - \hat{p}_n(1 - \hat{p}_n) \right] = \sqrt{n} \left[ \frac{V_{n,1}}{n} + \frac{WW_n}{2n} - \hat{p}_n \right] \xrightarrow{P} 0,$$

which now follows trivially from (I.3). Thus (i) holds and (ii) trivially follows. Part (iii) follows from Slutsky's theorem for randomization distributions; see Chung and Romano (2013), Theorem 5.2. Indeed, from Theorem 3.4 we know the permutation distribution based on  $\sqrt{n}\hat{D}_{n,1}(\mathbf{X})$  is asymptotically  $N(0, 1)$  (in probability) and the same must then be true for  $\sqrt{n}\hat{S}_{n,i}(\mathbf{X})$ . Part (iv) then follows because the critical values are also asymptotically (or exactly)  $z_{1-\alpha}$  under contiguous alternatives.  $\square$

**Remark I.1.** The permutation test based on the standardized first sample autocorrelation divided by the sample variance, which is not known to have any optimality properties for binary data, is equivalent to the permutation test based on  $\sum_{j=1}^n X_{ij}X_{i(j+1)}$  by the invariance of the sample mean and variance under permutations. In turn, the permutation test based on  $\sum_{j=1}^n X_{ij}X_{i(j+1)}$  is asymptotically equivalent to the permutation test based on  $\hat{P}_{n,1}(\mathbf{X}_i)$ ; See Wald and Wolfowitz (1940a). It also follows from (K.7) that the test based on  $\hat{P}_{n,1}(\mathbf{X}_i) - \hat{p}_{n,i}$  and  $\hat{D}_{n,1}(\mathbf{X}_i)$  are asymptotically equivalent. Therefore, the permutation tests based on  $\hat{S}_{n,i}(\mathbf{X}_i)$ ,  $\hat{D}_{n,1}(\mathbf{X}_i)$ ,  $\hat{P}_{n,1}(\mathbf{X}_i) - \hat{p}_{n,i}$ , and the first sample autocorrelation are asymptotically equivalent and Theorem I.1 can be applied to any of the four tests. Miller and Sanjurjo (2018) note this approximate equivalence. Their results are not asymptotic and are based on an approximate algebraic equivalence supported by simulation of correlations between the various test statistics.  $\blacksquare$

## J Permutation Tests of Individual Hypotheses $H_0^i$ in GVT

In this section, we display the results of permutation tests of the individual hypotheses  $H_0^i$  using the statistics  $\hat{P}_{n,k}(\mathbf{X}_i) - \hat{p}_{n,i}$  and  $\hat{D}_{n,k}(\mathbf{X}_i)$  implemented for each shooter from the GVT controlled basketball shooting experiment.

Online Appendix Figures 7 and 8 overlay the estimates of  $\hat{D}_{n,k}(\mathbf{X}_i)$  and  $\hat{P}_{n,k}(\mathbf{X}_i) - \hat{p}_{n,i}$  on to estimates of the permutation distributions for each shooter and streak length  $k = 1, \dots, 4$ . Each panel displays the density of the statistics of interest for each shooter over the permutation replications in a white-to-black gradient. The 95<sup>th</sup> quantile of the estimated permutation distributions are denoted by green horizontal line segments. The observed estimates for  $\hat{D}_{n,k}(\mathbf{X}_i)$  and  $\hat{P}_{n,k}(\mathbf{X}_i) - \hat{p}_{n,i}$  are denoted by black horizontal line segments. The observed values of  $\hat{D}_{n,k}(\mathbf{X}_i)$  are above the 97.5<sup>th</sup> quantile of the permutation distribution for 1 shooter for  $k$  equal to 1, 3 shooters for  $k$  equal to 2 and 4, and 4 shooters for  $k$  equal to 3. Online Appendix Tables 7 and 8 display the  $p$ -values of the permutation tests using  $\hat{D}_{n,k}(\mathbf{X}_i)$  and  $\hat{P}_{n,k}(\mathbf{X}_i) - \hat{p}_{n,i}$  for each  $k$  in  $1, \dots, 4$ .

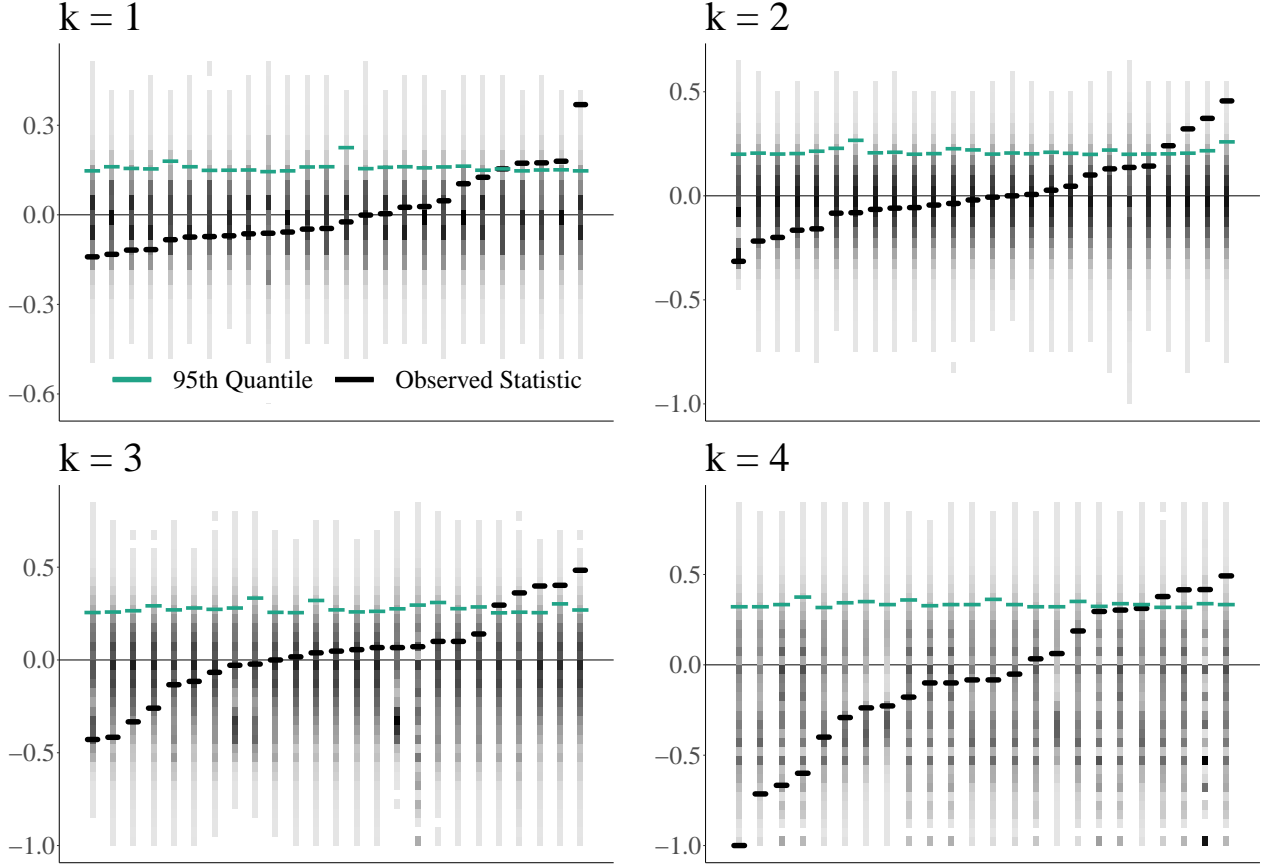

Online Appendix Figure 7: Individual Permutation Distributions and Critical Values:  $\hat{D}_{n,k}(\mathbf{X}_i)$

Notes: Figure displays the observed values of  $\hat{D}_{n,k}(\mathbf{X}_i)$  overlaid onto the estimated permutation distribution of  $\hat{D}_{n,k}(\mathbf{X}_i)$  under  $H_0^i$  for each  $k$  in  $1, \dots, 4$  and each shooter  $i$  with  $\hat{D}_{n,k}(\mathbf{X}_i)$  defined. The observed values of  $\hat{D}_{n,k}(\mathbf{X}_i)$  are denoted by black horizontal line segments. The estimated 95<sup>th</sup> quantile of the permutation distribution of  $\hat{D}_{n,k}(\mathbf{X}_i)$  under  $H_0^i$  is displayed by green horizontal line segments. We estimate the permutation distribution of  $\hat{D}_{n,k}(\mathbf{X}_i)$  under  $H_0^i$  by permuting  $\mathbf{X}_i$  100,000 times, computing  $\hat{D}_{n,k}(\mathbf{X}_i)$  for each permutation distribution. The estimates of the permutation distribution are displayed in vertical white to black gradients, shaded by the proportion of permutations whose computed value of  $\hat{D}_{n,k}(\mathbf{X}_i)$  lie in a fine partition of the observed support of  $\hat{D}_{n,k}(\mathbf{X}_i)$  under  $H_0^i$ . Within each panel, we sort the shooters by  $\hat{D}_{n,k}(\mathbf{X}_i)$ , with the smallest value on the left and the largest value on the right.

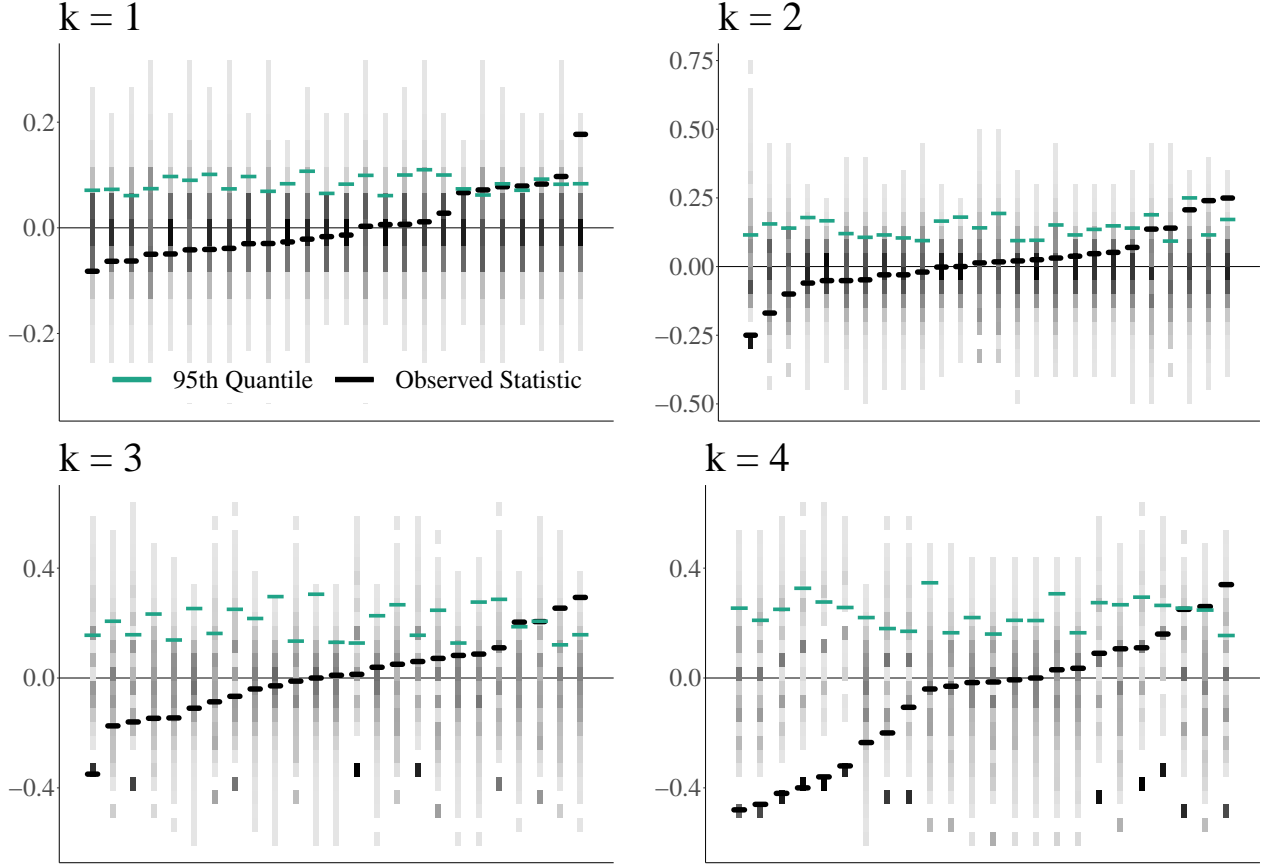

Online Appendix Figure 8: Individual Permutation Distributions and Critical Values:  $\hat{P}_{n,k}(\mathbf{X}_i) - \hat{p}_{n,i}$

Notes: Figure displays the observed values of  $\hat{P}_{n,k}(\mathbf{X}_i) - \hat{p}_{n,i}$  overlaid onto the estimated permutation distribution of  $\hat{P}_{n,k}(\mathbf{X}_i) - \hat{p}_{n,i}$  under  $H_0^i$  for each  $k$  in  $1, \dots, 4$  and each shooter  $i$  with  $\hat{P}_{n,k}(\mathbf{X}_i) - \hat{p}_{n,i}$  defined. The observed values of  $\hat{P}_{n,k}(\mathbf{X}_i) - \hat{p}_{n,i}$  are denoted by black horizontal line segments. The estimated 95<sup>th</sup> quantile of the permutation distribution of  $\hat{P}_{n,k}(\mathbf{X}_i) - \hat{p}_{n,i}$  under  $H_0^i$  is displayed by green horizontal line segments. We estimate the permutation distribution of  $\hat{P}_{n,k}(\mathbf{X}_i) - \hat{p}_{n,i}$  under  $H_0^i$  by permuting  $\mathbf{X}_i$  100,000 times, computing  $\hat{P}_{n,k}(\mathbf{X}_i) - \hat{p}_{n,i}$  for each permutation distribution. The estimates of the permutation distribution are displayed in vertical white to black gradients, shaded by the proportion of permutations whose computed value of  $\hat{P}_{n,k}(\mathbf{X}_i) - \hat{p}_{n,i}$  lie in a fine partition of the observed support of  $\hat{P}_{n,k}(\mathbf{X}_i) - \hat{p}_{n,i}$  under  $H_0^i$ . Within each panel, we sort the shooters by  $\hat{P}_{n,k}(\mathbf{X}_i) - \hat{p}_{n,i}$ , with the smallest value on the left and the largest value on the right.

| Shooter | $k$ | 1      | 2      | 3      | 4      |
|---------|-----|--------|--------|--------|--------|
| 101     |     | 0.8344 | 0.4824 | 0.2826 | 0.4393 |
| 102     |     | 0.4564 | 0.6254 | 0.8966 | –      |
| 103     |     | 0.0234 | 0.5820 | 0.4895 | 0.7063 |
| 104     |     | 0.6944 | 0.8675 | 0.5782 | 0.9637 |
| 105     |     | 0.8367 | 0.8649 | 0.9052 | 0.9921 |
| 106     |     | 0.0347 | 0.0259 | 0.0061 | 0.0304 |
| 107     |     | 0.0531 | 0.1548 | 0.0214 | 0.0752 |
| 108     |     | 0.5563 | 0.1700 | 0.2443 | 0.0341 |
| 109     |     | 0.0001 | 0.0000 | 0.0008 | 0.0188 |
| 110     |     | 0.6755 | 0.1905 | 0.3701 | 0.4101 |
| 111     |     | 0.3244 | 0.4094 | 0.3053 | 0.3862 |
| 112     |     | 0.6369 | 0.5446 | 0.3575 | 0.2956 |
| 113     |     | 0.7322 | 0.5718 | 0.2251 | 0.5630 |
| 114     |     | 0.5514 | 0.5216 | 0.2222 | 0.4174 |
| 201     |     | 0.8697 | 0.8120 | 0.8690 | 0.8977 |
| 202     |     | 0.1131 | 0.4383 | 0.4165 | 0.2789 |
| 203     |     | 0.0441 | 0.3112 | 0.1748 | 0.0646 |
| 204     |     | 0.6336 | 0.4240 | 0.2888 | 0.4126 |
| 205     |     | 0.3457 | 0.1255 | 0.4082 | 0.4652 |
| 206     |     | 0.9026 | 0.8165 | 0.7996 | 0.8777 |
| 207     |     | 0.0758 | 0.0014 | 0.0367 | 0.1447 |
| 208     |     | 0.7059 | 0.3595 | 0.2742 | 0.0546 |
| 209     |     | 0.6996 | 0.6436 | 0.3159 | 0.5357 |
| 210     |     | 0.4051 | 0.0043 | 0.0055 | 0.0068 |
| 211     |     | 0.2857 | 0.6081 | 0.5949 | 0.4421 |
| 212     |     | 0.6834 | 0.9557 | –      | –      |

Online Appendix Table 4: Individual Permutation Test  $p$ -values:  $\hat{D}_{n,k}(\mathbf{X}_i)$

Notes: Table displays the  $p$ -values for the individual level permutation tests rejecting for large values of  $\hat{D}_{n,k}(\mathbf{X}_i)$ . Each individual's shooting sequence is permuted 100,000 times.  $\hat{D}_{n,k}(\mathbf{X}_i)$  is computed on each permutation. The  $p$ -values are the proportions of permutations with  $\hat{D}_{n,k}(\mathbf{X}_i)$  greater than or equal to the observed  $\hat{D}_{n,k}(\mathbf{X}_i)$  among permutations where the statistic is defined.

| Shooter | $k$ | 1      | 2      | 3      | 4      |
|---------|-----|--------|--------|--------|--------|
| 101     |     | 0.8023 | 0.7377 | 0.5071 | 0.4210 |
| 102     |     | 0.3954 | 0.6891 | 0.6589 | –      |
| 103     |     | 0.0301 | 0.2987 | 0.4161 | 0.3924 |
| 104     |     | 0.6551 | 0.8638 | 0.4610 | 0.5191 |
| 105     |     | 0.8083 | 0.4928 | 0.5365 | 0.6016 |
| 106     |     | 0.0203 | 0.1901 | 0.1451 | 0.3102 |
| 107     |     | 0.0309 | 0.1550 | 0.1606 | 0.4302 |
| 108     |     | 0.6110 | 0.0885 | 0.2356 | 0.0461 |
| 109     |     | 0.0000 | 0.0001 | 0.0003 | 0.0115 |
| 110     |     | 0.5804 | 0.4318 | 0.5372 | 0.4515 |
| 111     |     | 0.3629 | 0.2377 | 0.2791 | 0.3137 |
| 112     |     | 0.5676 | 0.6121 | 0.4195 | 0.4562 |
| 113     |     | 0.6758 | 0.7232 | 0.7916 | 0.8964 |
| 114     |     | 0.5514 | 0.4434 | 0.3773 | 0.4191 |
| 201     |     | 0.8452 | 0.5693 | 0.7285 | 0.7942 |
| 202     |     | 0.0953 | 0.3849 | 0.2608 | 0.1019 |
| 203     |     | 0.0360 | 0.3315 | 0.1475 | 0.1441 |
| 204     |     | 0.5771 | 0.3480 | 0.2910 | 0.3480 |
| 205     |     | 0.3457 | 0.0697 | 0.6178 | 0.4310 |
| 206     |     | 0.9026 | 0.6241 | 0.7670 | 0.7319 |
| 207     |     | 0.0635 | 0.0048 | 0.0729 | 0.1656 |
| 208     |     | 0.6645 | 0.2271 | 0.0160 | 0.1744 |
| 209     |     | 0.6996 | 0.3754 | 0.2401 | 0.6096 |
| 210     |     | 0.3733 | 0.0055 | 0.0145 | 0.0106 |
| 211     |     | 0.2196 | 0.5480 | 0.8024 | 0.3941 |
| 212     |     | 0.6447 | 0.7288 | –      | –      |

Online Appendix Table 5: Individual Permutation Test  $p$ -values:  $\hat{P}_{n,k}(\mathbf{X}_i) - \hat{p}_{n,i}$

Notes: Table displays the  $p$ -values for the individual level permutation tests rejecting for large values of  $\hat{P}_{n,k}(\mathbf{X}_i) - \hat{p}_{n,i}$ . Each individual's shooting sequence is permuted 100,000 times.  $\hat{P}_{n,k}(\mathbf{X}_i) - \hat{p}_{n,i}$  is computed on each permutation. The  $p$ -values are the proportions of permutations with  $\hat{P}_{n,k}(\mathbf{X}_i) - \hat{p}_{n,i}$  greater than or equal to the observed  $\hat{P}_{n,k}(\mathbf{X}_i) - \hat{p}_{n,i}$  among permutations where the statistic is defined.

## K Proofs of Theorems Presented in the Main Text

### K.1 Proof of Theorem 3.1

**Proof of Theorem 3.1 (i)** We consider the case with  $s = 1$ , and therefore drop the dependence on the individual  $i$ . Recall that  $Y_{j,k} = \prod_{l=j}^{j+k} X_l$ .

First, we characterize the joint limiting distribution of  $(Y_{j,k}, Y_{j,k-1}, X_j)$ . Note that  $Y_{j,k}$  is  $k$ -dependent and strictly stationary. We need to compute the asymptotic expectations, variances, and covariances for each of the terms. First, the expectations. We can see that  $\mathbb{E}[Y_{j,k}] = p^{k+1}$  and that  $\mathbb{E}[X_j] = p$ .

Next, the variances. We can see that

$$\begin{aligned} \text{Cov}(Y_{j,k}, Y_{j+u,k}) &= \mathbb{E}[Y_{j,k} Y_{j+u,k}] - \mathbb{E}[Y_{j,k}] \mathbb{E}[Y_{j+u,k}] \\ &= p^{k+1+|u|} - p^{2k+2} \end{aligned}$$

for  $|u| \leq k$ . Therefore,

$$\begin{aligned} \sum_{u=-k}^{u=k} \text{Cov}(Y_{j,k}, Y_{j+u,k}) &= \sum_{u=-k}^{u=k} (p^{k+1+|u|} - p^{2k+2}) \\ &= p^{k+1} (1 - p^{k+1}) + 2 \sum_{u=1}^k (p^{k+1+u} - p^{2k+2}) \\ &= p^{k+1} - p^{2k+2} + 2 \sum_{u=1}^k (p^{k+1+u}) - 2kp^{2k+2} \\ &= p^{k+1} - (2k+1)p^{2k+2} + 2p^{k+1} \left( \frac{p(1-p^k)}{1-p} \right) \\ &= p^{k+1} - (2k+1)p^{2k+2} + \frac{2p^{k+2} - 2p^{2k+2}}{1-p}. \end{aligned} \tag{K.1}$$

Also, note that  $\text{Var}(X_j) = p(1-p)$ .

Finally, we compute the covariances. Note that

$$\begin{aligned} \text{Cov}(Y_{j,k}, Y_{j+u,k-1}) &= \mathbb{E}[Y_{j,k} Y_{j+u,k-1}] - \mathbb{E}[Y_{j,k}] \mathbb{E}[Y_{j+u,k-1}] \\ &= \mathbb{E} \left[ \prod_{l=j}^{j+k} X_l \prod_{l=j+u}^{j+u+k-1} X_l \right] - p^{2k+1} \\ &= \begin{cases} p^{k+u} - p^{2k+1} & \text{if } 1 < u \leq k \\ p^{k+1} - p^{2k+1} & \text{if } u \in \{0, 1\} \\ p^{k+1+|u|} - p^{2k+1} & \text{if } -k < u < 0 \\ 0 & \text{if } u \leq -k \text{ or } u > k. \end{cases} \end{aligned}$$

Therefore,

$$\begin{aligned}
\sum_{u=-k}^{u=k} \text{Cov}(Y_{j,k}, Y_{j+u,k-1}) &= 2p^{k+1} - 2p^{2k+1} + \sum_{u=2}^k (p^{k+u} - p^{2k+1}) + \sum_{u=1}^{k-1} (p^{k+1+u} - p^{2k+1}) \\
&= 2p^{k+1} - 2kp^{2k+1} + \sum_{u=2}^k p^{k+u} + \sum_{u=1}^{k-1} p^{k+1+u} \\
&= 2p^{k+1} - 2kp^{2k+1} + 2p^{k+1} \sum_{u=1}^{k-1} p^u \\
&= 2p^{k+1} - 2kp^{2k+1} + 2p^{k+1} \left( \frac{p(1-p^{k-1})}{1-p} \right) \\
&= 2p^{k+1} - 2kp^{2k+1} + \frac{2p^{k+2} - 2p^{2k+1}}{1-p}. \tag{K.2}
\end{aligned}$$

Additionally, observe that

$$\text{Cov}(Y_{j,k}, X_{j+u}) = \begin{cases} p^{k+1} - p^{k+2} & \text{if } 0 \leq u \leq k \\ 0 & \text{otherwise,} \end{cases}$$

and that therefore, we can evaluate

$$\sum_{u=-k}^{u=k} \text{Cov}(Y_{j,k}, X_{j+u}) = (k+1)(p^{k+1} - p^{k+2})$$

and

$$\sum_{u=-k}^{u=k} \text{Cov}(Y_{j,k-1}, X_{j+u}) = k(p^k - p^{k+1}).$$

By Theorem 1.7 of Ibragimov (1962) and the Cramér-Wold device, we have that

$$(n-k)^{-1/2} \left( \left( \sum_{j=1}^{n-k} Y_{j,k}, \sum_{j=1}^{n-k} Y_{j,k-1}, \sum_{j=1}^{n-k} X_j \right)^\top - (p^{k+1}, p^k, p)^\top \right) \xrightarrow{d} N(0, V),$$

where

$$V = \begin{bmatrix} p^{k+1} - (2k+1)p^{2k+2} + \frac{2p^{k+2}-2p^{2k+2}}{1-p} & 2p^{k+1} - 2kp^{2k+1} + \frac{2p^{k+2}-2p^{2k+1}}{1-p} & (k+1)(p^{k+1} - p^{k+2}) \\ \frac{2p^{k+1} - 2kp^{2k+1} + \frac{2p^{k+2}-2p^{2k+1}}{1-p}}{(k+1)(p^{k+1} - p^{k+2})} & p^k - (2k-1)p^{2k} + \frac{2p^{k+1}-2p^{2k}}{1-p} & k(p^k - p^{k+1}) \\ k(p^k - p^{k+1}) & & p(1-p) \end{bmatrix}.$$

Note that

$$n^{1/2} \left( n^{-1} \sum_{j=1}^n X_j / (n-k)^{-1} \sum_{j=1}^n X_j - 1 \right) \xrightarrow{p} 0,$$

so we can replace  $\frac{1}{n-k} \sum_{j=1}^{n-k} X_j$  with  $\frac{1}{n} \sum_{j=1}^n X_j$ .

Next, we use the delta method to evaluate the asymptotic distribution of  $\hat{P}_{n,k}(\mathbf{X}) - \hat{p}_n$ . Let  $g(\theta_1, \theta_2, \theta_3) = \theta_1/\theta_2 - \theta_3$ . Then  $\nabla g(\theta_1, \theta_2, \theta_3) = \left( \frac{1}{\theta_2}, \frac{-\theta_1}{\theta_2^2}, -1 \right)^\top$ . Evaluating at  $(p^{k+1}, p^k, p)^\top$ , we find

$$\nabla g(p^{k+1}, p^k, p) = \begin{bmatrix} p^{-k} \\ -p^{1-k} \\ -1 \end{bmatrix}.$$

Note that

$$\begin{aligned} & \begin{bmatrix} p^{-k} \\ -p^{1-k} \\ -1 \end{bmatrix}^\top V \begin{bmatrix} p^{-k} \\ -p^{1-k} \\ -1 \end{bmatrix} \\ &= \begin{bmatrix} p - (1+k(1-p))p^{1+k} \\ p - (k(1-p) + p)p^k \\ 0 \end{bmatrix}^\top \begin{bmatrix} p^{-k} \\ -p^{1-k} \\ -1 \end{bmatrix} \\ &= p^{1-k}(1-p)(1-p^k) \end{aligned}$$

and that  $p^{k+1}/p^k - p = 0$ . Hence,

$$n^{1/2} \left( \hat{P}_{n,k}(\mathbf{X}) - \hat{p}_n \right) \xrightarrow{d} N(0, p^{1-k}(1-p)(1-p^k)).$$

□

**Proof of Theorem 3.1 (ii)** We consider the case with  $s = 1$ , and therefore drop the dependence on the individual  $i$ . Recall that  $Y_{j,k} = \prod_{l=j}^{j+k} X_l$  and that  $Z_{j,k} = \prod_{l=j}^{j+k} (1 - X_l)$ .

First, we find the joint limiting distribution of  $(Y_{j,k}, Y_{j,k-1}, Z_{j,k}, Z_{j,k-1})$ . We need to compute the asymptotic expectations, variances, and covariances for each of the terms. First, the expectations. We can see that  $\mathbb{E}[Y_{j,k}] = p^{k+1}$  and  $\mathbb{E}[Z_{j,k}] = (1-p)^{k+1}$ .

Next, the variances. Recall from the proof of Theorem 3.1 (i) that  $\sum_{u=-k}^{u=k} \text{Cov}(Y_{j,k}, Y_{j+u,k})$  is given by (K.1) and so therefore

$$\sum_{u=-k}^{u=k} \text{Cov}(Z_{j,k}, Z_{j+u,k}) = (1-p)^{k+1} - (2k+1)(1-p)^{2k+2} + \frac{2(1-p)^{k+2} - 2(1-p)^{2k+2}}{p}.$$

Next, the covariances. Recall from the proof of Theorem 3.1 (i) that  $\sum_{u=-k}^{u=k} \text{Cov}(Y_{j,k}, Y_{j+u,k-1})$  is given by (K.2) and so therefore

$$\sum_{u=-k}^{u=k} \text{Cov}(Z_{j,k}, Z_{j+u,k-1}) = 2(1-p)^{k+1} - 2k(1-p)^{2k+1} + \frac{2(1-p)^{k+2} - 2(1-p)^{2k+1}}{p}.$$

Note that

$$\begin{aligned} \text{Cov}(Y_{j,k}, Z_{j+u,k}) &= \mathbb{E}[Y_{j,k}Z_{j+u,k}] - \mathbb{E}[Y_{j,k}]\mathbb{E}[Z_{j+u,k}] \\ &= \mathbb{E}[Y_{j,k}Z_{j+u,k}] - p^{k+1}(1-p)^{k+1} \\ &= -p^{k+1}(1-p)^{k+1} \text{ for } -k \leq u \leq k \\ \text{Cov}(Y_{j,k}, Z_{j+u,k-1}) &= \mathbb{E}[Y_{j,k}Z_{j+u,k-1}] - \mathbb{E}[Y_{j,k}]\mathbb{E}[Z_{j+u,k-1}] \\ &= \mathbb{E}[Y_{j,k}Z_{j+u,k-1}] - p^{k+1}(1-p)^k \\ &= -p^{k+1}(1-p)^k \text{ for } -k-1 \leq u \leq k \\ \text{Cov}(Y_{j,k-1}, Z_{j+u,k}) &= \mathbb{E}[Y_{j,k-1}Z_{j+u,k}] - \mathbb{E}[Y_{j,k-1}]\mathbb{E}[Z_{j+u,k}] \\ &= -p^k(1-p)^{k+1} \text{ for } -k \leq u \leq k-1 \end{aligned}$$

As  $\mathbb{E}[Y_{j,k}Z_{j+u,k}]$ ,  $\mathbb{E}[Y_{j,k}Z_{j+u,k-1}]$ , and  $\mathbb{E}[Y_{j,k-1}Z_{j+u,k}]$  are all equal to zero if there is any overlap in the  $X_j$ 's and  $(1-X_j)$ 's composing  $Y_{i,r}$  and  $Z_{i+u,s}$  for any  $r$  and  $s$ . We can see that

$$\begin{aligned} \sum_{u=-k}^{y=k} \text{Cov}(Y_{j,k}, Z_{j+u,k}) &= -(2k+1)p^{k+1}(1-p)^{k+1} \\ \sum_{u=-k}^{y=k} \text{Cov}(Y_{j,k+1}, Z_{j+u,k-1}) &= -(2k)p^{k+1}(1-p)^k \\ \sum_{u=-k+1}^{y=k+1} \text{Cov}(Y_{j,k}, Z_{j+u,k+1}) &= -(2k)p^k(1-p)^{k+1}. \end{aligned}$$

Therefore, by Theorem 1.7 of Ibragimov (1962) and the Cramér-Wold device, we have that

$$\begin{aligned} (n-k)^{-1/2} \left( \left( \sum_{j=1}^{n-k} Y_{j,k}, \sum_{j=1}^{n-k} Y_{j,k-1}, \sum_{j=1}^{n-k} Z_{j,k}, \sum_{j=1}^{n-k} Z_{j,k-1} \right)^\top - \left( p^{k+1}, p^k, (1-p)^{k+1}, (1-p)^k \right)^\top \right) \\ \xrightarrow{d} N \left( 0, \begin{bmatrix} \eta_{11} & \eta_{12} \\ \eta_{21} & \eta_{22} \end{bmatrix} \right). \end{aligned} \quad (\text{K.3})$$

where

$$\begin{aligned} \eta_{11} &= \begin{bmatrix} p^{k+1} - (2k+1)p^{2k+2} + \frac{2p^{k+2}-2p^{2k+2}}{1-p} & 2p^{k+1} - 2kp^{2k+1} + \frac{2p^{k+2}-2p^{2k+1}}{1-p} \\ 2p^{k+1} - 2kp^{2k+1} + \frac{2p^{k+2}-2p^{2k+1}}{1-p} & p^k - (2k-1)p^{2k} + \frac{2p^{k+1}-2p^{2k}}{1-p} \end{bmatrix}, \\ \eta_{21} &= \begin{bmatrix} -(2k+1)p^{k+1}(1-p)^{k+1} & -(2k)p^k(1-p)^{k+1} \\ -(2k)p^{k+1}(1-p)^k & -(2k-1)p^k(1-p)^k \end{bmatrix}, \\ \eta_{12} &= \begin{bmatrix} -(2k+1)p^{k+1}(1-p)^{k+1} & -(2k)p^{k+1}(1-p)^k \\ -(2k)p^k(1-p)^{k+1} & -(2k-1)p^k(1-p)^k \end{bmatrix}, \text{ and} \end{aligned}$$

$$\eta_{22} = \begin{bmatrix} (1-p)^{k+1} - (2k+1)(1-p)^{2k+2} + \frac{2(1-p)^{k+2} - 2(1-p)^{2k+2}}{p} & 2(1-p)^{k+1} - 2k(1-p)^{2k+1} + \frac{2(1-p)^{k+2} - 2(1-p)^{2k+1}}{p} \\ 2(1-p)^{k+1} - 2k(1-p)^{2k+1} + \frac{2(1-p)^{k+2} - 2(1-p)^{2k+1}}{p} & (1-p)^k - (2k-1)(1-p)^{2k} + \frac{2(1-p)^{k+1} - 2(1-p)^{2k}}{p} \end{bmatrix}.$$

Next, use the delta method to evaluate the asymptotic distribution of  $\hat{D}_{n,k}(\mathbf{X})$ .

Let  $g((\theta_1, \theta_2, \theta_3, \theta_4)^\top) = \theta_1/\theta_2 + \theta_3/\theta_4 - 1$ . Then  $\nabla g((\theta_1, \theta_2, \theta_3, \theta_4)^\top) = \left(\frac{1}{\theta_2}, \frac{-\theta_1}{\theta_2^2}, \frac{1}{\theta_4}, \frac{-\theta_3}{\theta_4^2}\right)^\top$ .

Evaluating at

$(p^{k+1}, p^k, (1-p)^{k+1}, (1-p)^k)^\top$ , we find  $g((p^{k+1}, p^k, (1-p)^{k+1}, (1-p)^k)^\top) = 0$  and

$$\nabla g\left((p^{k+1}, p^k, (1-p)^{k+1}, (1-p)^k)^\top\right) = \begin{bmatrix} p^{-k} \\ -p^{1-k} \\ (1-p)^{-k} \\ -(1-p)^{1-k} \end{bmatrix}.$$

Note that

$$\begin{aligned} & \begin{bmatrix} p^{-k} \\ -p^{1-k} \\ (1-p)^{-k} \\ -(1-p)^{1-k} \end{bmatrix}^\top \begin{bmatrix} \eta_{11} & \eta_{12} \\ \eta_{21} & \eta_{22} \end{bmatrix} \begin{bmatrix} p^{-k} \\ -p^{1-k} \\ (1-p)^{-k} \\ -(1-p)^{1-k} \end{bmatrix} \\ &= \begin{bmatrix} p(1-p^k) \\ p-p^k \\ (1-p)(1-(1-p)^k) \\ (1-p)-(1-p)^k \end{bmatrix}^\top \begin{bmatrix} p^{-k} \\ -p^{1-k} \\ (1-p)^{-k} \\ -(1-p)^{1-k} \end{bmatrix} \\ &= (p(1-p))^{1-k} \left((1-p)^k + p^k\right) \end{aligned}$$

Hence, we have that

$$n^{1/2} \hat{D}_{n,k}(\mathbf{X}) \xrightarrow{d} N\left(0, (p(1-p))^{1-k} \left((1-p)^k + p^k\right)\right).$$

□

## K.2 Proof of Theorem 3.2

Let  $G_i = \sum_{j=1}^n X_{ij}$  be the number of ones. Under  $H_0^i$ ,  $G_i$  is sufficient. Hence the test function  $\varphi(G_i)$  defined by

$$\varphi(G_i) = \mathbb{E}[\varphi(\mathbf{X}_i) | G_i] \tag{K.4}$$

does not depend on  $p_i$ , i.e., it only depends on the data through  $G_i$ . But,  $\mathbb{E}[\varphi(G_i)] = \mathbb{E}[\varphi(\mathbf{X}_i)]$ , which equals  $\alpha$  for all  $p_i$  by assumption. Moreover, the completeness of  $G_i$  implies that  $\varphi(G_i) = \alpha$ ; that is,

$$\mathbb{E}[\varphi(\mathbf{X}_i) | G_i] = \alpha. \tag{K.5}$$

But, the conditional distribution of  $\mathbf{X}_i$  given  $G_i = g$  puts mass  $1/n!$  at each of the data sets  $x_\pi$ , so (K.4) is equivalent to (K.5). □

### K.3 Proof of Theorem 3.3

**Proof of Theorem 3.3 (i)** We consider the case with  $s = 1$ , and therefore drop the dependence on the individual  $i$ . Recall that  $V_{n,k} = \sum_{j=1}^{n-k} Y_{j,k}$  and  $W_{n,k} = \sum_{j=1}^{n-k} Z_{j,k}$  where  $Y_{j,k} = \prod_{l=j}^{j+k} X_l$  and  $Z_{j,k} = \prod_{l=j}^{j+k} (1 - X_l)$ .

First, we prove the result in the case  $k = 1$ . The test statistic under consideration is  $\sqrt{n}\hat{D}_{n,1}(\mathbf{X})$ , where

$$\begin{aligned}\hat{D}_{n,1}(X_1, \dots, X_n) &= \frac{V_{n,1}}{V_{n,0}} - \left(1 - \frac{W_{n,1}}{W_{n,0}}\right) \\ &= \frac{V_{n,1}}{V_{n,0}} - \frac{\sum_{j=1}^{n-1} (1 - X_j) X_{j+1}}{n - V_{n,0}} = \frac{V_{n,1}}{V_{n,0}} - \frac{\sum_{j=2}^n X_j - V_{n,1}}{n - V_{n,0}} \\ &= \frac{\frac{V_{n,1}}{n} - \frac{(\sum_{j=2}^n X_j) \cdot V_{n,0}}{n^2}}{\frac{V_{n,0}}{n} \left(1 - \frac{V_{n,0}}{n}\right)}.\end{aligned}\tag{K.6}$$

The denominator of (K.6) tends to  $p(1 - p)$  with probability one. Since  $|V_{n,0} - \sum_{j=2}^n X_j| \leq 2$ , it follows that

$$\sqrt{n} \left( \frac{V_{n,1}}{n} - \frac{(\sum_{j=2}^n X_j) \cdot V_{n,0}}{n^2} \right) - \sqrt{n} \left( \frac{V_{n,1}}{n} - \frac{V_{n,0}^2}{n^2} \right) \xrightarrow{P} 0.$$

Therefore,

$$\sqrt{n}\hat{D}_{n,1}(\mathbf{X}) = \frac{\sqrt{n} \left( \frac{V_{n,1}}{n} - \frac{V_{n,0}^2}{n^2} \right)}{\frac{V_{n,0}}{n} \left(1 - \frac{V_{n,0}}{n}\right)} + o_P(1).\tag{K.7}$$

Let

$$\Pi = \Pi_n = (\Pi(1), \dots, \Pi(n))$$

denote a (uniform) random permutation of  $(1, 2, \dots, n)$  independent of  $X_j$  for all  $j$ .

We need to analyze the joint limiting distribution of  $\sqrt{n} \left( \hat{D}_{n,1}(\mathbf{X}), \hat{D}_{n,1}(\mathbf{X}_\Pi) \right)$ , where

$$\hat{D}_{n,1}(\mathbf{X}_\Pi) = \hat{D}_{n,1}(X_{\Pi(1)}, \dots, X_{\Pi(n)}).$$

In particular, to verify Hoeffding's condition (See Lehmann and Romano 2005, Theorem 15.2.3), we need to verify that  $\sqrt{n}\hat{D}_{n,1}(\mathbf{X})$  and  $\sqrt{n}\hat{D}_{n,1}(\mathbf{X}_\Pi)$  are asymptotically independent. We already know that the marginal distributions of the joint limiting distribution of  $\sqrt{n}\hat{D}_{n,1}(\mathbf{X})$  and  $\sqrt{n}\hat{D}_{n,1}(\mathbf{X}_\Pi)$  are standard normal. Since the denominator  $V_{n,0}/n(1 - V_{n,0}/n)$  is invariant under permutations and tends to  $p(1 - p)$  with probability one, it suffices to show  $\sqrt{n}f(\bar{V}_{n,1}, \bar{V}_{n,0})$  and

$\sqrt{n}f(\tilde{V}_{n,1}, \bar{V}_{n,0})$  are asymptotically independent, where

$$f(v_1, v_0) = v_1 - v_0^2 \quad \bar{V}_{n,1} = V_{n,1}/n \quad \bar{V}_{n,0} = V_{n,0}/n$$

and

$$\bar{V}_{n,1}^\Pi = \frac{1}{n} \sum_{j=1}^{n-1} X_{\Pi(j)} X_{\Pi(j+1)}.$$

Note that  $\sqrt{n}(\bar{V}_{n,1}, \bar{V}_{n,0})$  and  $\sqrt{n}(\bar{V}_{n,1}^\Pi, \bar{V}_{n,0})$  are not asymptotically independent. Next, apply the Delta Method, noting that averaging over  $n$  or  $n-1$  does not affect our analysis. So,

$$\sqrt{n}f(\bar{V}_{n,1}, \bar{V}_{n,0}) = \sqrt{n}[\bar{V}_{n,1} - p^2 - 2p(\bar{V}_{n,0} - p)] + o_p(1).$$

The variance of the linear approximation is equal to

$$\begin{aligned} & n [\text{Var}(\bar{V}_{n,1}) + 2p^2 \text{Var}(\bar{V}_{n,0}) - 4p \text{Cov}(\bar{V}_{n,1}, \bar{V}_{n,0})] \\ &= p^2(1-p^2) + 4(p^3 - p^4) + 4p^3(1-p) - 8p(p^2 - p^3) = p^2(1-p)^2. \end{aligned}$$

Using the linear approximation for both the original statistic and the permuted statistic, we can apply the Cramér-Wold device. Let

$$T_j = n^{-1/2} \{a[X_j X_{j+1} - p^2 - 2p(X_j - p)] + b[X_{\Pi(j)} X_{\Pi(j+1)} - p^2 - 2p(X_{\Pi(j)} - p)]\}. \quad (\text{K.8})$$

Therefore, it suffices to show that, for any  $a$  and  $b$ ,  $\sum_{j=1}^n T_j$  is asymptotically normal with mean 0 and variance  $(a^2 + b^2)p^2(1-p)^2$ .

We now determine the limiting behavior of  $\sum_j T_j$  by applying a Central Limit Theorem of Stein (1986) for dependent random variables in a form stated in Rinott (1994). To do this, we will condition on  $\Pi_n = \pi_n$ , so that Theorem 2.2 of Rinott (1994) is applicable. For shorthand, drop the subscript on  $\pi_n = \pi$ . Let  $S_j$  be the set of indices  $l$  such that  $T_j$  and  $T_l$  are dependent. Clearly,  $S_j$  contains both  $j$  and  $j+1$ . But,  $S_j$  also contains the indices  $l$  for which  $\pi(l) = j$  or  $\pi(l) = j+1$ , as well as the indices  $l$  for which  $\pi(l+1) = j$  or  $\pi(l+1) = j+1$ . So,  $|S_j| \leq 6$ , the important thing being that the size of  $|S_j|$  is uniformly bounded. Moreover,  $|T_j| \leq C/\sqrt{n}$  for some constant  $C$ , which only depends on  $a$  and  $b$ . Next we examine

$$\sigma_n^2 = \text{Var} \left( \sum_{j=1}^n T_j \right) = \frac{1}{n} \text{Var} \left( \sum_{j=1}^n a[X_j X_{j+1} - 2pX_j] + b[X_{\pi(j)} X_{\pi(j+1)} - 2pX_{\pi(j)}] \right).$$

Again, these terms are for a given permutation  $\pi$ , though we don't explicitly include the condition-

ing operation in all variance and covariance expressions. By our previous calculations,

$$\sigma_n^2 = (a^2 + b^2) p^2 (1-p)^2 + o(1) + \frac{2ab}{n} \text{Cov} \left[ \sum_{j=1}^{n-1} a (X_j X_{j+1} - 2p X_j), \sum_{j=1}^{n-1} b (X_{\pi(j)} X_{\pi(j+1)} - 2p X_{\pi(j)}) \right]. \quad (\text{K.9})$$

We now show that the covariance term in (K.9) is  $o(1)$ . It can be expressed as

$$\begin{aligned} & \frac{2ab}{n} \left[ \text{Cov} \left( \sum_{j=1}^{n-1} X_j X_{j+1}, \sum_{l=1}^{n-1} X_{\pi(l)} X_{\pi(l+1)} \right) + 4p^2 \text{Var} \left( \sum_{j=1}^n X_j \right) - 4p \text{Cov} \left( \sum_{j=1}^{n-1} X_j X_{j+1}, \sum_{l=1}^{n-1} X_l \right) \right] \\ &= 2ab \left[ \frac{1}{n} \text{Cov} \left( \sum_{j=1}^{n-1} X_j X_{j+1}, \sum_{l=1}^{n-1} X_{\pi(l)} X_{\pi(l+1)} \right) + 4p^3 (1-p) - 2p^3 (1-p) + o(1) \right]. \end{aligned} \quad (\text{K.10})$$

Next,

$$\frac{1}{n} \text{Cov} \left( \sum_{j=1}^{n-1} X_j X_{j+1}, \sum_{l=1}^{n-1} X_{\pi(l)} X_{\pi(l+1)} \right) = \frac{1}{n} \sum_{j=1}^{n-1} \sum_{l=1}^{n-1} \text{Cov} (X_j X_{j+1}, X_{\pi(l)} X_{\pi(l+1)}).$$

Now, for every  $j$ , there exists  $l$  such that  $\pi(l) = j$ . For such a  $l$ , if  $\pi(l+1) \neq j+1$ , then the  $(j, l)$  covariance term in the double sum equals  $p^3(1-p)$ . Similarly, there exists a  $l$  such that  $\pi(l+1) = j$ . If  $\pi(l) \neq j+1$ , then the  $(j, l)$  term also equals  $p^3(1-p)$ . Similarly, there exists a  $l$  such that  $\pi(l) = j+1$  and if  $\pi(l+1) \neq j$ , the term is also  $p^3(1-p)$ . Finally, there exists  $l+1$  such that  $\pi(l+1) = j+1$  and if  $\pi(l) \neq j$ , the term is also  $p^3(1-p)$ . So, the number of pairings of the above form is  $4(n-1)$ , except possibly if the permutation “preserves” ordering in the sense  $\pi(l) = j$  and  $\pi(l) = j+1$  or  $\pi(l+1) = j$  and  $\pi(l+1) = j+1$ , in which case the covariance term would be  $p^2 - p^4$ . If, for a given sequence  $\pi_n$ , the number of such pairings is uniformly bounded above by some constant  $E$ , then (K.10) is equal to  $4p^3(1-p) + o(1)$ , and therefore (K.9) is equal to  $o(1)$ , as desired.

Unfortunately, we cannot simply argue that there is such a finite constant  $E$ , because if  $\pi$  is the identity permutation, the number of terms grows with  $n$ , though the identity permutation is an extremely unlikely outcome for a random permutation. Hence, we argue as follows. Let  $N_n$  be the number of indices  $(j, l)$  for which a random permutation  $\Pi$  satisfies  $(\Pi(l), \Pi(l+1)) = (j, j+1)$  and similarly let  $N'_n$  be the number of  $(\Pi(l+1), \Pi(l)) = (j+1, j)$ . But,

$$\mathbb{E}[N_n] = \sum_{j=1}^{n-1} \sum_{l=1}^{n-1} \mathbb{P}\{\Pi(l) = j, \Pi(l+1) = j+1\} = \sum_{j=1}^{n-1} \sum_{l=1}^{n-1} \frac{1}{n} \cdot \frac{1}{n-1} = \frac{n-1}{n},$$

and similarly for  $\mathbb{E}'[N_n]$ . Therefore,  $M_n \equiv N_n + N'_n$  is uniformly bounded in expectation and, being nonnegative, is therefore tight. Hence, for any subsequence  $n_l$ , there exists a further subsequence for which  $M_n$  converges in distribution. By the almost sure representation theorem, there exists  $\tilde{M}_n$  with the same distribution as  $M_n$  which converges almost surely to some  $\tilde{M}$ . Based

on  $\tilde{M} = m$ , construct  $\tilde{\Pi}_n$  according to the conditional distribution of  $\Pi_n | M_n = m$ , so that unconditionally  $\tilde{\Pi}_n$  is uniform over permutations. Then, along a subsequence, the above argument applies as if  $M$  were finite. To sum up, given any subsequence  $n_l$  there exists a further subsequence  $n' = n_{lm}$  such that

$$\mathbb{P} \left\{ \sum_{j=1}^n Z_j \leq t | \tilde{\Pi}_{n'} \right\} \rightarrow \Phi \left( t / \left[ \sqrt{(a^2 + b^2)p(1-p)} \right] \right)$$

with probability one. Hence, unconditionally, by dominated convergence,

$$\mathbb{P} \left\{ \sum_{j=1}^n T_j \leq t \right\} \rightarrow \Phi \left( t / \left[ \sqrt{(a^2 + b^2)p(1-p)} \right] \right). \quad (\text{K.11})$$

Since, given any subsequence, the same limit obtains for a further subsequence, the limit in (K.11) holds along the original subsequence. Hence, Hoeffding's condition holds.

Now for general  $k$ . That is, we consider the test statistic

$$\sqrt{n} \hat{D}_{n,k}(\mathbf{X}) = \sqrt{n} \left[ \frac{\bar{V}_{n,k}}{\bar{V}_{n,k-1}} - \left( 1 - \frac{\bar{W}_{n,k}}{\bar{W}_{n,k-1}} \right) \right],$$

where

$$\bar{V}_{n,k} = \frac{1}{n} \sum_{j=1}^{n-k} X_j \cdots X_{j+k}$$

and

$$\bar{W}_{n,k} = \frac{1}{n} \sum_{j=1}^{n-k} (1 - X_j) \cdots (1 - X_{j+k}).$$

Using the Taylor approximation

$$\frac{\bar{V}_{n,k}}{\bar{V}_{n,k-1}} = p + p^{-k} \bar{V}_{n,k} - p^{1-k} \bar{V}_{n,k-1} + O_P(n^{-1})$$

and similarly for  $\bar{W}_{n,k}/\bar{W}_{n,k-1}$  yields

$$\hat{D}_{n,k}(\mathbf{X}) = p^{-k} \bar{V}_{n,k} - p^{1-k} \bar{V}_{n,k-1} + (1-p)^{-k} \bar{W}_{n,k} - (1-p)^{1-k} \bar{W}_{n,k-1} + O_P(n^{-1}).$$

As in the proof of  $k = 1$ , we need to verify Hoeffding's condition, i.e that  $\sqrt{n} \hat{D}_{n,k}(\mathbf{X})$  and  $\sqrt{n} \hat{D}_{n,k}(\mathbf{X}_{\Pi})$  are asymptotically independent, where

$$\hat{D}_{n,k}(\mathbf{X}_{\Pi}) = \hat{D}_{n,k}(X_{\Pi(1)}, \dots, X_{\Pi(n)})$$

is the statistic  $\hat{D}_{n,k}(\mathbf{X})$  evaluated at randomly permuted data  $X_{\Pi(1)}, \dots, X_{\Pi(n)}$ . As before, we first

fix (or condition on)  $\Pi = \pi$ . For a given permutation  $\pi$ , define

$$\bar{V}_{n,k}^\pi = \frac{1}{n} \sum_{i=1}^{n-k} X_{\pi(1)}, \dots, X_{\pi(i+k)},$$

and similarly for  $\bar{W}_{n,k}^\pi$ . Using the same argument as in  $k = 1$ , we must show that

$$\begin{aligned} n \operatorname{Cov} \left[ p^{-k} \bar{V}_{n,k} - p^{1-k} \bar{V}_{n,k-1} + (1-p)^{-k} \bar{W}_{n,k} - (1-p)^{1-k} \bar{W}_{n,k-1} \right. \\ \left. p^{-k} \bar{V}_{n,k}^\pi - p^{1-k} \bar{V}_{n,k-1}^\pi + (1-p)^{-k} \bar{W}_{n,k}^\pi - (1-p)^{1-k} \bar{W}_{n,k-1}^\pi \right] \rightarrow 0. \end{aligned} \quad (\text{K.12})$$

Before evaluating (K.12), which is a covariance between a linear combination of four random variables with another four random variables, we calculate the 16 individual covariances as follows:

$$\begin{aligned} n \operatorname{Cov}(\bar{V}_{n,k}, \bar{V}_{n,k}^\pi) &\rightarrow (k+1)^2 p^{2k+1} (1-p) \\ n \operatorname{Cov}(\bar{V}_{n,k}, \bar{V}_{n,k-1}^\pi) &\rightarrow k(k+1) p^{2k} (1-p) \\ n \operatorname{Cov}(\bar{V}_{n,k-1}, \bar{V}_{n,k}^\pi) &\rightarrow k(k+1) p^{2k} (1-p) \\ n \operatorname{Cov}(\bar{V}_{n,k-1}, \bar{V}_{n,k-1}^\pi) &\rightarrow k^2 p^{2k-1} (1-p) \\ n \operatorname{Cov}(\bar{W}_{n,k}, \bar{W}_{n,k}^\pi) &\rightarrow (k+1)^2 (1-p)^{2k+1} p \\ n \operatorname{Cov}(\bar{W}_{n,k}, \bar{W}_{n,k-1}^\pi) &\rightarrow k(k+1) (1-p)^{2k} p \\ n \operatorname{Cov}(\bar{W}_{n,k-1}, \bar{W}_{n,k}^\pi) &\rightarrow k(k+1) (1-p)^{2k} p \\ n \operatorname{Cov}(\bar{W}_{n,k-1}, \bar{W}_{n,k-1}^\pi) &\rightarrow k^2 (1-p)^{2k-1} p \\ n \operatorname{Cov}(\bar{V}_{n,k}, \bar{W}_{n,k}^\pi) &\rightarrow -(k+1)^2 p^{k+1} (1-p)^{k+1} \\ n \operatorname{Cov}(\bar{V}_{n,k}, \bar{W}_{n,k-1}^\pi) &\rightarrow -k(k+1) p^{k+1} (1-p)^k \\ n \operatorname{Cov}(\bar{V}_{n,k-1}, \bar{W}_{n,k}^\pi) &\rightarrow -k(k+1) p^k (1-p)^{k+1} \\ n \operatorname{Cov}(\bar{V}_{n,k-1}, \bar{W}_{n,k-1}^\pi) &\rightarrow -k^2 p^k (1-p)^k \\ n \operatorname{Cov}(\bar{W}_{n,k}, \bar{V}_{n,k}^\pi) &\rightarrow -(k+1)^2 p^{k+1} (1-p)^{k+1} \\ n \operatorname{Cov}(\bar{W}_{n,k-1}, \bar{V}_{n,k}^\pi) &\rightarrow -k(k+1) p^{k+1} (1-p)^k \\ n \operatorname{Cov}(\bar{W}_{n,k}, \bar{V}_{n,k-1}^\pi) &\rightarrow -k(k+1) p^k (1-p)^{k+1} \\ n \operatorname{Cov}(\bar{W}_{n,k-1}, \bar{V}_{n,k-1}^\pi) &\rightarrow -k^2 p^k (1-p)^k \end{aligned} \quad (\text{K.13})$$

The above 16 calculations are all similar, so we explain just (K.13). Note that

$$n \operatorname{Cov}(\bar{V}_{n,k}, \bar{V}_{n,k}^\pi) = \frac{1}{n} \sum_{j=1}^{n-k} \sum_{l=1}^{n-k} \operatorname{Cov}(X_1 \cdots X_{j+k}, X_{\pi(l)} \cdots X_{\pi(l+k)}). \quad (\text{K.14})$$

Clearly, the  $(j, l)$  term in the double sum is zero if there is no overlap between the sets of indices  $\{j, \dots, j+k\}$  and  $\{\pi(l), \dots, \pi(l+k)\}$ . Then, for any fixed  $j$ , there exists some  $l$  such that  $\pi(l) = j$ , in which case there is overlap. Similarly, for any fixed  $m$  and  $r$ , each in  $\{1, \dots, k\}$

there exists  $l$  such that  $\pi(l+r) = j+m$ . Hence, there are  $(k+1)^2$  sets of indices where there is some overlap between  $\{j, \dots, j+k\}$  and  $\{\pi(l), \dots, \pi(l+k)\}$ . If for each combination of  $m$  and  $r$ , there is only one index that is shared, then the covariance is  $p^{2k+1}(1-p)$ . There are  $(k+1)^2$  such terms. The only concern is there may be some further overlap in the sense that more than one index is shared among the sets. However, we will argue that, while this can occur, it has a small probability and hence will have negligible effect. To do this, for a given permutation  $\pi$ , let  $N_n = N_n^\pi$  be the number of terms with at least two indices in common; that is, let

$$N_n^\pi = \sum_{j=1}^{n-k} \sum_{l=1}^{n-k} I \left\{ |\{j, \dots, j+k\} \cap \{\pi(l), \dots, \pi(l+k)\}| \geq 2 \right\}.$$

Since  $N_n^\pi$  can be bounded by the number of times pairs of indices are in common, we have

$$N_n^\pi \leq \sum_{j=1}^{n-k} \sum_{l=1}^{n-k} \sum_{m=0}^k \sum_{m'=0}^k \sum_{r=0}^k \sum_{r'=0}^k I \left\{ \pi(l+r) = j+m \cap \pi(l+r') = j+m' \right\}.$$

Then, continuing from (K.14),

$$|n \text{Cov}(\bar{V}_{n,k}, \bar{V}_{n,k}^\pi) - \frac{1}{n} (n-k) (k+1)^2 p^{2k+1} (1-p)| \leq N_n^\pi/n.$$

Therefore, for any given  $\pi$  (sequence), as long as  $N_n^\pi/n \rightarrow 0$ , the above 16 convergences hold.

Moreover, by the bilinearity of covariance, the above 16 convergences then allow us to calculate the LHS of (K.12) as the limit of the following 16 terms

$$\begin{aligned} & np^{-2k} \text{Cov}(\bar{V}_{n,k}, \bar{V}_{n,k}^\pi) - np^{1-2k} \text{Cov}(\bar{V}_{n,k}, \bar{V}_{n,k-1}^\pi) + \dots + n(1-p)^{2-2k} \text{Cov}(\bar{V}_{n,k-1}, \bar{V}_{n,k-1}^\pi) \\ & \rightarrow p(1-p)[(k+1)^2 - k(k+1) - (k+1)^2 + k(k+1) - k(k+1) + k^2 + k(k+1) - k^2 \\ & - (k+1)^2 + k(k+1) + (k+1)^2 - k(k+1) + k(k+1) - k^2 - k(k+1) + k^2] = 0 \end{aligned}$$

yielding the desired conclusion.

Thus, the covariance calculation implying the required asymptotic independence in Hoeffding's condition holds, as long as  $N_n^\pi/n \rightarrow 0$ . (The asymptotic normality holds by the Central Limit Theorem of Stein 1986, used in the case  $k=1$  above.) This may not hold for every  $\pi$  (such as the identity permutation), but we now argue that, viewing  $N_n^\Pi$  as a function of  $\Pi$  (i.e a random variable),  $N_n^\Pi/n \rightarrow 0$  in probability. To see why,

$$\mathbb{E} [N_n^\Pi/n] \leq \sum_{j=1}^{n-k} \sum_{l=1}^{n-k} \frac{(k+1)^2 k^2}{n(n+1)} \leq (k+1)^2 k^2,$$

which is bounded in  $n$ . Thus, by Markov's inequality,

$$N_n^\Pi/n \xrightarrow{P} 0.$$

This does not guarantee  $N_n^\Pi/n \rightarrow 0$  for almost every realization of the random permutation sequence  $\Pi$  (really  $\Pi_n$ ), but we can use a subsequence argument as follows. Given any subsequence  $n_l$ , there exists a further subsequence  $n' = n_{lm}$  such that  $N_{n'} \rightarrow 0$  with probability one along the subsubsequence. Therefore, along the subsubsequence, we have that Hoeffding's condition holds for almost all realizations of  $\Pi'_n$ . We may then conclude, for any  $\epsilon > 0$

$$\mathbb{P} \left\{ |\hat{R}_{n'}(t) - \Phi(t/\sigma_k(p))| > \epsilon | \Pi_{n'} \right\} \rightarrow 0,$$

and so by dominated convergence

$$\hat{R}_{n'}^T(t) \rightarrow \Phi(t/\sigma_D(p, k))$$

with probability one along the subsubsequence. Since we can start with any subsequence before passing to a subsubsequence, and the limit remains the same, we can conclude that

$$\hat{R}_n^T(t) \xrightarrow{P} \Phi(t/\sigma_D(p, k)).$$

□

**Proof of Theorem 3.3 (ii)** We consider the case with  $s = 1$ , and therefore drop the dependence on the individual  $i$ . The proof is analogous to the proof of Theorem 3.3 (i). We provide the most important difference, the covariance calculation.

Similar to  $\hat{D}_{n,k}(\mathbf{X})$ ,

$$\hat{E}_{n,k}(\mathbf{X}) = \hat{P}_{n,k}(X_1, \dots, X_n) - \hat{p}_n$$

admits a Taylor approximation given by

$$\hat{E}_{n,k}(\mathbf{X}) = p^{-k} \bar{V}_{n,k} - p^{k-1} \bar{V}_{n,k-1} - \bar{X}_n + O_P(n^{-1}).$$

Therefore, we need to show that, for fixed sequences  $\pi = \pi_n$  (such that  $N_n^\pi/n \rightarrow 0$  where  $N_n^\pi$  is defined as in the proof of Theorem 3.3 (i)),

$$n \text{Cov} \left( p^{-k} \bar{V}_{n,k} - p^{k-1} \bar{V}_{n,k-1} - \bar{X}_n, p^{-k} \bar{V}_{n,k}^\pi - p^{k-1} \bar{V}_{n,k-1}^\pi - \bar{X}_n^\pi \right) \rightarrow 0.$$

But the left side is

$$\begin{aligned} & 2p^{1-2k} n \text{Cov}(\bar{V}_{n,k}, \bar{V}_{n,k-1}^\pi) - 2p^{-k} n \text{Cov}(\bar{V}_{n,k}, \bar{X}_n) + 2p^{1-k} n \text{Cov}(\bar{V}_{n,k-1}^\pi, \bar{X}_n) \\ & + n \text{Var}(\bar{X}_n) + p^{-2k} n \text{Cov}(\bar{V}_{n,k}, \bar{V}_{n,k}^\pi) + p^{2-2k} n \text{Cov}(\bar{V}_{n,k-1}, \bar{V}_{n,k-1}^\pi). \end{aligned} \quad (\text{K.15})$$

Similar to the argument for (K.14), we have

$$n \text{Cov}(\bar{X}_n, \bar{V}_{n,k}) \rightarrow (k+1)p^{k+1}(1-p)$$

and

$$n \text{Cov}(\bar{X}_n, \bar{V}_{n,k-1}) \rightarrow k^2 p^{2k-1} (1-p).$$

Plugging the limiting covariances into (K.15) yields the limiting variance of

$$\begin{aligned} & -2p^{1-2k}k(k+1)p^{2k}(1-p) - 2p^{-k}(k+1)p^{k+1}(1-p) + 2p^{1-2k}kp^k(1-p) \\ & + p(1-p) + p^{-2k}(k+1)^2p^{2k+1}(1-p) + p^{2-2k}k^2p^{2k-1}(1-p), \end{aligned}$$

which equals 0. □

#### K.4 Proof of Theorem 3.4

We consider the case with  $s = 1$ , and therefore drop the dependence on the individual  $i$ . First, We need to establish an asymptotic equicontinuity property of  $L_n(h)$ . Let  $\rho(F, G)$  denote the Levy metric between distributions  $F$  and  $G$ .

**Lemma K.1.** *Given any  $\delta > 0$ , there exists  $\delta' > 0$  such that if  $|h_n - h| \leq \delta'$ , then*

$$\rho(L_n(h_n), L_n(h)) \leq \delta$$

for sufficiently large  $n$ .

*Proof.* We use the following coupling of data sets based on  $a_n(h_n)$  number of successes and also  $a_n(h)$  number of successes. That is, let  $\mathbf{X} = (X_1, \dots, X_n)$  be the data set with the first  $a_n = a_n(h_n)$  entries equal to 1 and the rest 0. Similarly, let  $\mathbf{X}' = (X'_1, \dots, X'_n)$  be the data set with the first  $a'_n = a_n(h)$  entries equal to 1 and the rest 0. We first claim that, for any  $\delta > 0$  and any permutation  $\pi$  applied to both  $\mathbf{X}$  and  $\mathbf{X}'$ , there exists  $\delta' > 0$  independent of  $\pi$ , such that for sufficiently large  $n$  independent of  $\pi$ ,

$$\sqrt{n}|\hat{D}_{n,1}(\mathbf{X}_\pi) - \hat{D}_{n,1}(\mathbf{X}'_\pi)| \leq \delta \tag{K.16}$$

if  $|h_n - h| \leq \delta'$ . The lemma would then follow because  $L_n(h)$  puts equal mass at the values  $\sqrt{n}\hat{D}_{n,1}(\mathbf{X}_\pi)$  as  $\pi$  varies while  $L_n(h)$  puts equal mass at the values  $\sqrt{n}\hat{D}_{n,1}(\mathbf{X}'_\pi)$ . In general, if  $F$  puts mass  $1/N$  at data points  $a_1, \dots, a_N$  and  $G$  puts mass  $1/N$  at data points  $b_1, \dots, b_N$ , with  $|b_i - a_i| \leq \delta$ , then  $\rho(F, G) \leq \delta$ . We now verify the statement surrounding (K.16). Since the difference of two equicontinuous functions is equicontinuous, it suffices to verify the statement with  $\hat{D}_{n,1}(\mathbf{X})$  replaced by  $\hat{P}_{n,1}(\mathbf{X})$ . This entails showing that, given  $\delta > 0$ , there exists  $\delta' > 0$  such that

$$\sqrt{n} \left| \frac{\sum_{j=1}^{n-1} X_{\pi(j)} X_{\pi(j+1)}}{\sum_{j=1}^{n-1} X_{\pi(j)}} - \frac{\sum_{j=1}^{n-1} X'_{\pi(j)} X'_{\pi(j+1)}}{\sum_{j=1}^{n-1} X'_{\pi(j)}} \right| \tag{K.17}$$

is  $\leq \delta$  if  $|h_n - h| \leq \delta'$ . Let  $T = \sum_{j=1}^{n-1} X_{\pi(j)}$  and  $T' = \sum_{j=1}^{n-1} X'_{\pi(j)}$ . Clearly,

$$a_n(h_n) - 1 \leq T \leq S(h_n)$$

and

$$a_n(h) - 1 \leq T' \leq a_n(h).$$

Now, (K.17) can be expressed as

$$\frac{\sqrt{n}}{T'T} (T' - T) \sum_{j=1}^{n-1} X_{\pi(j)} X_{\pi(j+1)} + \frac{\sqrt{n}}{T'} \sum_{j=1}^{n-1} [X_{\pi(j)} X_{\pi(j+1)} - X'_{\pi(j)} X'_{\pi(j+1)}]. \quad (\text{K.18})$$

Separate (K.18) into the terms  $A_n + B_n$ , and we show each term is  $\leq \delta/2$  for an appropriate choice of  $\delta'$ . The sum in  $A_n$  can be bounded by  $T$ , so that

$$|A_n| \leq \sqrt{n} \left| \frac{T - T'}{T'} \right|.$$

Consider the case where  $h_n > h$ , so then

$$\begin{aligned} |A_n| &\leq \sqrt{n} \left( \frac{\lfloor \frac{n}{2} + \sqrt{n}h_n \rfloor - \lfloor \frac{n}{2} + \sqrt{n}h \rfloor - 1}{\lfloor \frac{n}{2} + \sqrt{n}h \rfloor - 1} \right) \\ &\leq \sqrt{n} \left( \frac{\frac{n}{2} + \sqrt{n}h_n - (\frac{n}{2} + \sqrt{n}h - 1) - 1}{\frac{n}{2} + \sqrt{n}h - 2} \right) \\ &= \frac{h_n - h}{\frac{1}{2} + \frac{h}{\sqrt{n}} - \frac{2}{\sqrt{n}}}. \end{aligned}$$

In general,

$$|A_n| \leq \frac{|h_n - h|}{\frac{1}{2} + \frac{h}{\sqrt{n}} - \frac{2}{\sqrt{n}}},$$

which can be made to be  $\leq \delta$  for all large  $n$  for  $\delta'$  chosen sufficiently small, as long as  $h$  is restricted to be in a bounded set.

To bound  $B_n$ , note that by the coupling construction of  $\mathbf{X}$  and  $\mathbf{X}'$ ,  $\mathbf{X}$  and  $\mathbf{X}'$  differ in at most  $|a_n(h_n) - a_n(h)|$  entries. Therefore, for any  $\pi$ ,  $X_{\pi(i)} X_{\pi(i+1)} - X'_{\pi(i)} X'_{\pi(i+1)}$  are 0 except for at most  $2|a_n(h_n) - a_n(h)|$  number of them, and the nonzero ones can be bounded above by 1. Therefore,

$$|B_n| \leq \frac{2\sqrt{n}}{T'} |a_n(h_n) - a_n(h)|,$$

which, similar to  $A_n$ , can be bounded above by

$$|B_n| \leq \frac{2|h_n - h| + \frac{2}{\sqrt{n}}}{\frac{1}{2} + \frac{h}{\sqrt{n}}}.$$

Therefore, for large enough  $n$ , chosen independently of  $\pi$ , the bound can be made  $\leq \delta/2$  if  $|h_n - h| \leq \delta'$  for sufficiently small  $\delta'$ .

In summary, for some sufficiently chosen positive  $\delta'$  and large enough  $n$ , (K.16) holds for all

$\pi$ , and the lemma follows.  $\square$

Next, we can characterize the behavior of the permutation distributions for the statistic test  $\sqrt{n}\hat{D}_{n,1}(\mathbf{X}_i)$  under nonrandom sequences  $h_n \rightarrow h$ . Note that, if  $h_n$  is nonrandom, so is  $L_n(h_n)$  and the limit result does not require any probabilistic qualification, such as convergence in probability or almost surely.

**Lemma K.2.** *Assume  $h_n \rightarrow h$ . Let  $L_n(h_n)$  be the permutation distribution for  $T_n = \hat{D}_{n,1}(\mathbf{X}_i)$  based on  $\lfloor \frac{n}{2} + h\sqrt{n} \rfloor$  ones (and the remaining zeros). Equivalently, if  $a_n$  is the number of ones at time  $n$ , then assume  $n^{-1/2}(\hat{a}_n - \frac{n}{2}) \rightarrow h$ . Then,*

$$L_n(h_n) \xrightarrow{d} N(0, 1)$$

as  $n \rightarrow \infty$ .

*Proof.* Assume the opposite. Then, there exists  $\epsilon > 0$  such that

$$\rho(L_n(h), N(0, 1)) > \epsilon$$

for infinitely many  $n$ . Assume this holds for all large  $n$ , or apply the argument below to a subsequence. Let  $\delta = \epsilon/2$ . Then, there exists  $\delta' > 0$  such that for large  $n$ ,  $\rho(L_n(h), L_n(h_n)) \leq \delta$  if  $|h_n - h| \leq \delta'$ . Let  $E_n$  be the set of  $a_n(h_n)$  with  $|h_n - h| \leq \delta'$ .

Consider i.i.d. sampling with  $p = \frac{1}{2}$  and let  $\hat{a}_n$  be the number of successes. Then, with an abuse of notation,

$$\mathbb{P}_{p=\frac{1}{2}}\{\hat{a}_n \in E_n\} = \mathbb{P}_{p=\frac{1}{2}}\left\{n^{-1/2}\left|\hat{a}_n - \frac{n}{2}\right| \leq \delta'\right\} \rightarrow c > 0. \quad (\text{K.19})$$

Let  $\hat{h}_n = n^{1/2}(\hat{a}_n - \frac{n}{2})$ . When  $E_n$  occurs, we have for sufficiently large  $n$ ,

$$\rho(L_n(\hat{h}_n), L_n(h)) \leq \delta = \epsilon/2,$$

which by the triangle inequality implies

$$\rho(L_n(\hat{h}_n), N(0, 1)) \geq \epsilon/2$$

for sufficiently large  $n$ . Note  $L_n(\hat{h}_n)$  is indeed the (random) permutation distribution based on i.i.d. Bernoulli trials with success probability  $1/2$ . But, because convergence in the Levy metric is weaker than convergence of distributions in the supremum metric,

$$\mathbb{P}_{p=\frac{1}{2}}\left\{\rho(L_n(\hat{h}_n), N(0, 1)) \geq \epsilon/2\right\} \rightarrow 0,$$

which is a contradiction because the probability of  $E_n$  does not tend to 0, by (K.19).  $\square$

We now turn to the proof of the main result. It suffices to show, given any subsequence  $n'$  there exists a further subsequence  $n''$  such that  $\sup_t |\hat{R}_{n''}^T(t) - \Phi(t)| \rightarrow 0$  with probability one. Now appeal to the Almost Sure Representation Theorem, and construct  $\tilde{a}_n$  with the same distribution as  $\hat{a}_n$  such that  $n^{-1/2}(\tilde{a}_n - np)$  converges to some  $G$  almost surely. But, for every sequence for which  $n^{-1/2}(\tilde{a}_n - np)$  converges, we have  $\sup_t |\hat{R}_{n''}^T(t) - \Phi(t)| \rightarrow 0$ , by Lemma K.2. Since convergence occurs with probability one, the result holds.  $\square$

## K.5 Proof of Theorem 4.1

We consider the case with  $s = 1$ , and therefore drop the dependence on the individual  $i$ .

Note that the  $n$ -step transition matrix admits a closed form, given by

$$\mathcal{P}^n = \begin{bmatrix} \frac{1}{2} + \frac{1}{2}(2\epsilon)^n & \frac{1}{2} - \frac{1}{2}(2\epsilon)^n \\ \frac{1}{2} - \frac{1}{2}(2\epsilon)^n & \frac{1}{2} + \frac{1}{2}(2\epsilon)^n \end{bmatrix},$$

and that the stationarity of  $\{X_j\}_{j=1}^n$  implies that  $X_1$  is 0 or 1 with probabilities  $1/2$ .

We apply the delta method, and so need to compute the asymptotic variances and covariances of  $\bar{V}_{n,1}$  and  $\bar{V}_{n,0}$ . First, we evaluate

$$\sqrt{n} \text{Var}(\bar{X}_n) = \text{Var}(X_1) + 2 \sum_{j=1}^{n-1} \left(1 - \frac{j}{n}\right) \text{Cov}(X_1, X_{j+1}).$$

For all  $j \geq 1$ ,

$$\begin{aligned} \mathbb{E}[X_1 X_{j+1}] &= \mathbb{E}[X_1 X_{j+1} | X_1 = 1] + \mathbb{E}[X_1 X_{j+1} | X_1 = 0] \\ &= \frac{1}{2} \mathbb{P}(X_{j+1} = 1 | X_1 = 1) \\ &= \frac{1}{2} \left( \frac{1}{2} + \frac{1}{2} (2\epsilon)^j \right) \end{aligned}$$

which implies that

$$\text{Cov}(X_1, X_{j+1}) = \frac{1}{2} \left( \frac{1}{2} + \frac{1}{2} (2\epsilon)^j \right) - \frac{1}{4} = \frac{1}{4} (2\epsilon)^j$$

and that therefore

$$\begin{aligned} \sqrt{n} \text{Var}(\bar{X}_n) &= \frac{1}{4} + 2 \sum_{j=1}^{n-1} \left(1 - \frac{j}{n}\right) \frac{1}{4} (2\epsilon)^j \\ &\rightarrow \frac{1}{4} + \frac{1}{2} \sum_{j=1}^{\infty} (2\epsilon)^j \end{aligned}$$

$$\begin{aligned}
&= \frac{1}{4} + \frac{1}{2} \left[ \frac{1}{1-2\epsilon} - 1 \right] \\
&= \frac{1}{4} + \frac{\epsilon}{1-2\epsilon}.
\end{aligned}$$

Next, we evaluate

$$\sqrt{n} \operatorname{Var} \left( \sum_{j=1}^{n-1} X_j X_{j+1} \right) = \operatorname{Var} (X_1 X_2) + 2 \sum_{j=1}^{n-1} \left( 1 - \frac{j}{n-1} \right) \operatorname{Cov} (X_1 X_2, X_{j+1} X_{j+2}).$$

In order to do so, we would need to evaluate  $\mathbb{E} [X_1 X_2 X_{j+1} X_{j+2}]$ . If we set  $j = 1$ , then

$$\begin{aligned}
\mathbb{E} [X_1 X_2 X_{j+1} X_{j+2}] &= \mathbb{E} [X_1 X_2 X_3] \\
&= \frac{1}{2} \mathbb{E} [X_1 X_2 X_3 | X_1 = 1] \\
&= \frac{1}{2} \left( \frac{1}{2} + \epsilon \right)^2,
\end{aligned}$$

and we can evaluate

$$\begin{aligned}
\operatorname{Cov} (X_1 X_2, X_2 X_3) &= \frac{1}{2} \left( \frac{1}{2} + \epsilon \right)^2 - \frac{1}{4} \left( \frac{1}{2} + \epsilon \right)^2 \\
&= \frac{1}{2} \left( \frac{1}{2} + \epsilon \right)^2.
\end{aligned}$$

If we set  $j > 1$ , then

$$\mathbb{E} [X_1 X_2 X_{j+1} X_{j+2}] = \frac{1}{2} \left( \frac{1}{2} + \frac{1}{2} (2\epsilon)^{j-1} \right) \left( \frac{1}{2} + \epsilon \right)^2$$

and

$$\begin{aligned}
\operatorname{Cov} (X_1 X_2, X_{j+1} X_{j+2}) &= \frac{1}{2} \left( \frac{1}{2} + \frac{1}{2} (2\epsilon)^{j-1} \right) \left( \frac{1}{2} + \epsilon \right)^2 - \frac{1}{4} \left( \frac{1}{2} + \epsilon \right)^2 \\
&= \frac{1}{4} (2\epsilon)^{j-1} \left( \frac{1}{2} + \epsilon \right)^2.
\end{aligned}$$

Therefore, we see that

$$\sqrt{n} \operatorname{Var} \left( \sum_{j=1}^{n-1} X_j X_{j+1} \right) = \frac{1}{2} \left( \frac{1}{2} + \epsilon \right) \left( 1 - \frac{1}{2} \left( \frac{1}{2} + \epsilon \right) \right) + \frac{1}{2} \sum_{j=1}^{n-2} \left( 1 - \frac{j}{n-1} \right) (2\epsilon)^{j-1} \left( \frac{1}{2} + \epsilon \right)^2$$

$$\begin{aligned}
& \rightarrow \left(\frac{1}{4} + \frac{\epsilon}{2}\right) \left(\frac{3}{4} - \frac{\epsilon}{2}\right) + \frac{1}{2} \left(\frac{1}{2} + \epsilon\right)^2 \sum_{j=0}^{\infty} (2\epsilon)^j \\
& = \left(\frac{1}{4} + \frac{\epsilon}{2}\right) \left(\frac{3}{4} - \frac{\epsilon}{2}\right) + \frac{1}{2} \left(\frac{1}{2} + \epsilon\right)^2 \frac{1}{1 - 2\epsilon}.
\end{aligned}$$

Finally, we evaluate

$$\text{Cov} \left( \sum_{j=1}^n X_j, \sum_{l=1}^{n-1} X_l X_{l+1} \right) = \sum_{j=1}^n \sum_{l=1}^{n-1} \text{Cov} (X_j, X_l X_{l+1}). \quad (\text{K.20})$$

In order to do so, we need to evaluate  $\mathbb{E} [X_j X_l X_{l+1}]$ . If we set  $j = l$ , then  $\mathbb{E} [X_l X_{l+1}] = \frac{1}{2} \left(\frac{1}{2} + \epsilon\right)$  and  $\text{Cov} (X_l, X_l X_{l+1}) = \frac{1}{2} \left(\frac{1}{2} + \epsilon\right) - \frac{1}{4} \left(\frac{1}{2} - \epsilon\right) = \frac{1}{4} \left(\frac{1}{2} + \epsilon\right)$ . Similarly, if  $j = l + 1$ , then  $\mathbb{E} [X_l X_{l+1}] = \frac{1}{2} \left(\frac{1}{2} + \epsilon\right)$  and  $\text{Cov} (X_{l+1}, X_l X_{l+1}) = \frac{1}{4} \left(\frac{1}{2} + \epsilon\right)$ . If we set  $j < l$ , then

$$\begin{aligned}
\mathbb{E} [X_j X_l X_{l+1}] &= \frac{1}{2} \left( \frac{1}{2} + \frac{(2\epsilon)^{l-j}}{2} \right) \left( \frac{1}{2} + \epsilon \right) \\
&= \frac{1}{4} \left( 1 + (2\epsilon)^{l-j} \right) \left( \frac{1}{2} + \epsilon \right)
\end{aligned}$$

and

$$\begin{aligned}
\text{Cov} (X_j X_l X_{l+1}) &= \frac{1}{4} \left( 1 + (2\epsilon)^{l-j} \right) \left( \frac{1}{2} + \epsilon \right) - \frac{1}{4} \left( \frac{1}{2} + \epsilon \right) \\
&= \frac{1}{4} \left( (2\epsilon)^{l-j} \right) \left( \frac{1}{2} + \epsilon \right).
\end{aligned}$$

If we set  $j > l + 1$ , then

$$\begin{aligned}
\mathbb{E} [X_j X_l X_{l+1}] &= \frac{1}{2} \left( \frac{1}{2} + \frac{(2\epsilon)^{j-l-1}}{2} \right) \left( \frac{1}{2} + \epsilon \right) \\
&= \frac{1}{4} \left( 1 + (2\epsilon)^{j-l-1} \right) \left( \frac{1}{2} + \epsilon \right)
\end{aligned}$$

and

$$\begin{aligned}
\text{Cov} (X_j X_l X_{l+1}) &= \frac{1}{4} \left( 1 + (2\epsilon)^{j-l-1} \right) \left( \frac{1}{2} + \epsilon \right) - \frac{1}{4} \left( \frac{1}{2} + \epsilon \right) \\
&= \frac{1}{4} \left( (2\epsilon)^{j-l-1} \right) \left( \frac{1}{2} + \epsilon \right).
\end{aligned}$$

Therefore, we have shown

$$\text{Cov}(X_j X_l X_{l+1}) = \begin{cases} \frac{1}{4} \left( (2\epsilon)^{l-j} \right) \left( \frac{1}{2} + \epsilon \right) & \text{if } j \leq l \\ \frac{1}{4} \left( (2\epsilon)^{j-l-1} \right) \left( \frac{1}{2} + \epsilon \right) & \text{if } j > l. \end{cases}$$

We can evaluate (K.20) by splitting the summation.

$$\sum_{j=1}^n \sum_{l=1}^{n-1} \text{Cov}(X_j, X_l X_{l+1}) = \sum_{j=1}^n \sum_{l=j}^{n-1} \text{Cov}(X_j, X_l X_{l+1}) + \sum_{j=2}^n \sum_{l=1}^{j-1} \text{Cov}(X_j, X_l X_{l+1}). \quad (\text{K.21})$$

The first term of (K.21) can be evaluated at the limit as

$$\begin{aligned} \frac{1}{n} \sum_{j=1}^n \sum_{l=j}^{n-1} \text{Cov}(X_j, X_l X_{l+1}) &= \frac{1}{n} \sum_{j=1}^n \sum_{l=1}^{n-1} \frac{1}{4} (2\epsilon)^{l-j} \left( \frac{1}{2} + \epsilon \right) \\ &= \frac{1}{n} \sum_{j=1}^n \sum_{m=0}^{n-j-1} \frac{1}{4} (2\epsilon)^m \left( \frac{1}{2} + \epsilon \right) \\ &= \frac{1}{n} \sum_{j=1}^n \frac{1}{4} \left( \frac{1}{2} + \epsilon \right) \sum_{m=0}^{n-j-1} (2\epsilon)^m \\ &= \frac{1}{n} \sum_{j=1}^n \frac{1}{4} \left( \frac{1}{2} + \epsilon \right) \frac{1 - (2\epsilon)^{n-j}}{1 - (2\epsilon)} \\ &\rightarrow \frac{1}{4} \left( \frac{1}{2} + \epsilon \right) \frac{1}{1 - 2\epsilon}. \end{aligned}$$

Likewise, the second term of (K.21) can be evaluated at the limit as

$$\begin{aligned} \frac{1}{n} \sum_{j=2}^n \sum_{l=1}^{j-1} \text{Cov}(X_j, X_l X_{l+1}) &= \frac{1}{n} \sum_{j=2}^n \sum_{l=1}^{j-1} \frac{1}{4} (2\epsilon)^{j-l-1} \left( \frac{1}{2} + \epsilon \right) \\ &= \frac{1}{n} \sum_{j=2}^n \frac{1}{4} \left( \frac{1}{2} + \epsilon \right) \sum_{m=1}^{j-1} (2\epsilon)^{m-1} \\ &= \frac{1}{n} \sum_{j=1}^n \frac{1}{4} \left( \frac{1}{2} + \epsilon \right) \frac{1 - (2\epsilon)^{j-1}}{1 - (2\epsilon)} \\ &\rightarrow \frac{1}{4} \left( \frac{1}{2} + \epsilon \right) \frac{1}{1 - 2\epsilon}. \end{aligned}$$

Hence, we can sum the limits to see that

$$\lim_{n \rightarrow \infty} \frac{1}{n} \sum_{j=1}^n \sum_{l=1}^{n-1} \text{Cov} (X_j, X_l X_{l+1}) \rightarrow \frac{1}{2} \left( \frac{1}{2} + \epsilon \right) \frac{1}{1-2\epsilon}.$$

As  $\{X_j\}_{j=1}^n$  and  $\{X_j X_{j+1}\}_{j=1}^{n-1}$  are irreducible and aperiodic, they are both  $\alpha$ -mixing by Theorem 3.1 of Bradley (2005). Therefore, by Theorem B.0.1 of Politis et. al (1999), a central limit theorem for  $\alpha$ -mixing triangular arrays, and the Cramér-Wold device, we have that

$$\sqrt{n} \left( \bar{X}_n - \frac{1}{2}, \frac{\sum_{j=1}^{n-1} X_j X_{j+1}}{n-1} - \frac{1}{2} \left( \frac{1}{2} + \epsilon \right) \right) \xrightarrow{d} N(0, \Sigma)$$

where

$$\Sigma = \begin{bmatrix} \frac{1}{4} + \frac{\epsilon}{1-2\epsilon} & \frac{1}{2} \left( \frac{1}{2} + \epsilon \right) \frac{1}{1-2\epsilon} \\ \frac{1}{2} \left( \frac{1}{2} + \epsilon \right) \frac{1}{1-2\epsilon} & \left( \frac{1}{4} + \frac{\epsilon}{2} \right) \left( \frac{3}{4} - \frac{\epsilon}{2} \right) + \frac{1}{2} \left( \frac{1}{2} + \epsilon \right)^2 \frac{1}{1-2\epsilon} \end{bmatrix}.$$

Next, we apply the delta method to evaluate the limiting distribution of  $\hat{D}_{n,1}(\mathbf{X})$ . Note that, as in the proof of Theorem 3.3 (i),

$$\sqrt{n} \left( \hat{D}_{n,1}(\mathbf{X}) - 2\epsilon \right) = \sqrt{n} \left( \frac{\bar{V}_{n,1} - \bar{V}_{n,0}^2}{\bar{V}_{n,0} (1 - \bar{V}_{n,0})} - 2\epsilon \right) + o_p(1).$$

Let

$$f(v_0, v_1) = \frac{v_1 - v_0^2}{v_0 (1 - v_0)}$$

and define  $\mu_1 = \mathbb{E} [\bar{V}_{n,1}] = \frac{1}{2} \left( \frac{1}{2} + \epsilon \right)$  and  $\mu_0 = \mathbb{E} [\bar{V}_{n,0}] = \frac{1}{2}$ . We can evaluate

$$f(\mu_0, \mu_1) = \frac{\frac{1}{2} \left( \frac{1}{2} + \epsilon \right) - \frac{1}{4}}{1/4} = 2\epsilon,$$

$$\left. \frac{\partial f}{\partial v_0} \right|_{\mu} = \left. \frac{-2v_0^2 (1 - v_0) - (v_1 - v_0^2) (1 - 2v_0)}{v_0^2 (1 - v_0)^2} \right|_{\mu} = -4,$$

and

$$\left. \frac{\partial f}{\partial v_1} \right|_{\mu} = \left. \frac{1}{v_0 (1 - v_0)} \right|_{\mu} = 4.$$

Therefore, we can see that

$$\sqrt{n} \left( \hat{D}_{n,1}(\mathbf{X}) - 2\epsilon \right) = \sqrt{n} \left( 4 (\bar{V}_{n,1} - \mu_1) - 4 (\bar{V}_{n,0} - \mu_0) \right) + o_p(1).$$

Note that

$$\text{Var} \left( 4 (\bar{V}_{n,1} - \mu_1) - 4 (\bar{V}_{n,0} - \mu_0) \right)$$

$$\begin{aligned}
&= 16 \left( \frac{1}{4} + \frac{\epsilon}{1-2\epsilon} + \left( \frac{1}{4} + \frac{\epsilon}{2} \right) \left( \frac{3}{4} - \frac{\epsilon}{2} \right) + \frac{1}{2} \left( \frac{1}{2} + \epsilon \right)^2 \frac{1}{1-2\epsilon} - 2 \left( \frac{1}{2} \right) \left( \frac{1}{2} + \epsilon \right) \frac{1}{1-2\epsilon} \right) \\
&= 1 - 4\epsilon^2.
\end{aligned}$$

Hence, we have that

$$n^{1/2} \left( \hat{D}_{n,1}(\mathbf{X}) - 2\epsilon \right) \xrightarrow{d} N(0, 1 - 4\epsilon^2).$$

Finally, we apply the delta method to evaluate the limiting distribution of  $\hat{P}_{n,1} - \hat{p}_n$ . Let

$$h(v_0, v_1) = \frac{v_1}{v_0} - v_0$$

We can evaluate

$$h(\mu_0, \mu_1) = \epsilon,$$

$$\left. \frac{\partial h}{\partial v_0} \right|_{\mu} = \left. \frac{-v_1}{v_0^2} - 1 \right|_{\mu} = -2 - 2\epsilon,$$

and

$$\left. \frac{\partial h}{\partial v_1} \right|_{\mu} = \left. \frac{1}{v_0} \right|_{\mu} = 2.$$

Therefore, we can see that

$$\sqrt{n} \left( \hat{P}_{n,1}(\mathbf{X}) - \hat{p}_n - \epsilon \right) = \sqrt{n} \left( 2(\bar{V}_{n,1} - \mu_1) - (2 + 2\epsilon)(\bar{V}_{n,0} - \mu_0) \right) + o_p(1).$$

Note that

$$\begin{aligned}
&\text{Var} \left( 2(\bar{V}_{n,1} - \mu_1) - (2 + 2\epsilon)(\bar{V}_{n,0} - \mu_0) \right) \\
&= 4 \left( \left( \frac{1}{4} + \frac{\epsilon}{2} \right) \left( \frac{3}{4} - \frac{\epsilon}{2} \right) + \frac{1}{2} \left( \frac{1}{2} + \epsilon \right)^2 \frac{1}{1-2\epsilon} \right) \\
&+ (2 + 2\epsilon)^2 \left( \frac{1}{4} + \frac{\epsilon}{1-2\epsilon} \right) - 4(2 + 2\epsilon) \left( \frac{1}{2} \left( \frac{1}{2} + \epsilon \right) \frac{1}{1-2\epsilon} \right) \\
&= \frac{1 - 2\epsilon + 16\epsilon^2}{4 - 8\epsilon}.
\end{aligned}$$

Hence, we have that

$$n^{1/2} \left( \hat{P}_{n,1} - \hat{p}_n - \epsilon \right) \xrightarrow{d} N \left( 0, \frac{1 - 2\epsilon + 16\epsilon^2}{4 - 8\epsilon} \right).$$

□

## References

- Carhart, M. M. (1997). On persistence in mutual fund performance. *The Journal of Finance*, 52(1):57–82.
- Chung, E. and Romano, J. P. (2013). Exact and asymptotically robust permutation tests. *Annals of Statistics*, 41(2):484–507.
- Clopper, C. J. and Pearson, E. S. (1934). The use of confidence or fiducial limits illustrated in the case of the binomial. *Biometrika*, 26(4):404–413.
- CRSP(Center for Research in Security Prices) (2020). *Daily Stock Security Files*. <http://www.crsp.org/> [Accessed: September 1, 2020].
- Donoho, D. and Jin, J. (2004). Higher criticism for detecting sparse heterogeneous mixtures. *Annals of Statistics*, 32(3):962–994.
- Fama, E. F. (1965). The behavior of stock-market prices. *The Journal of Business*, 38(1):34–105.
- Fama, E. F. (1970). Efficient capital markets: A review of theory and empirical work. *The Journal of Finance*, 25(2):383–417.
- FirstRate Data (2020). *Historical Intraday Dow Jones Industrial Average (DJI) Data*. <https://firstratedata.com/i/index/DJI> [Accessed: September 3, 2020].
- Fisher, R. A. (1925). Theory of statistical estimation. *Mathematical Proceedings of the Cambridge Philosophical Society*, 22(5):700–725.
- Hendricks, D., Patel, J., and Zeckhauser, R. (1993). Hot hands in mutual funds: Short-run persistence of relative performance, 1974–1988. *The Journal of Finance*, 48(1):93–130.
- Hendricks, D., Patel, J., and Zeckhauser, R. (1997). The j-shape of performance persistence given survivorship bias. *The Review of Economics and Statistics*, 79(2):161–166.
- Ibragimov, I. A. (1962). Some limit theorems for stationary processes. *Theory of Probability & Its Applications*, 7(4):349–382.
- Imbens, G. W. and Rubin, D. B. (2015). *Causal Inference for Statistics, Social, and Biomedical Sciences: An Introduction*. Cambridge University Press.
- Jensen, M. C. (1968). The performance of mutual funds in the period 1945-1964. *The Journal of Finance*, 23(2):389–416.
- Lehmann, E. L. and Romano, J. P. (2005). *Testing Statistical Hypotheses*. Springer, NY, 3<sup>rd</sup> edition.
- Malkiel, B. G. (2003). The efficient market hypothesis and its critics. *Journal of Economic Perspectives*, 17(1):59–82.

- Miller, J. B. and Sanjurjo, A. (2018). A cold shower for the hot hand fallacy: Robust evidence that belief in the hot hand is justified. *University of Alicante mimeo*.
- Rinott, Y. (1994). On normal approximation rates for certain sums of dependent random variables. *Computational and Applied Mathematics*, 55(2):134–143.
- Romano, J. P. and Wolf, M. (2005). Exact and approximate stepdown methods for multiple hypothesis testing. *Journal of the American Statistical Association*, 100(469):94–108.
- Rubin, D. (1990). Formal mode of statistical inference for causal effects. *Journal of Statistical Planning and Inference*, 25(3):279–292.
- Stein, C. (1986). Approximate computation of expectations.
- Wald, A. and Wolfowitz, J. (1940a). An exact test for randomness in the non-parametric case based on serial correlation. *Annals of Mathematical Statistics*, 14(4):378–388.
- Wald, A. and Wolfowitz, J. (1940b). On a test whether two samples are from the same population. *Annals of Mathematical Statistics*, 11(2):147–162.
